# Supplementary material for: Extremes of the internal energy of the Potts model on cubic graphs
Source: arXiv:1610.08496 ancillary file (2017-05-18)
Supplement: Supplementary file 1 [file PottsCompanionA3.pdf]

# PROPERTIES OF LOCAL VIEWS FOR CUBIC GRAPHS

EWAN DAVIES, MATTHEW JENSSEN, WILL PERKINS, AND BARNABY ROBERTS

This is a companion note to [1] presenting the output of the computer program used to verify the observations required for Theorem 1. The program itself is included in the ancillary files of the arXiv submission.

*Local view 1 of 35 (named  $C_1$ ).*

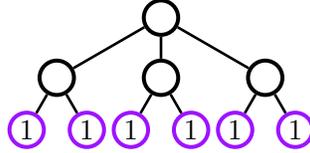

$$\begin{aligned}
 Z_C &= \lambda^9 + 4\lambda^6(q-1) + 3\lambda^5(q-1) + 3\lambda^4(q-1)(q-2) + 3\lambda^4(q-1) + 9\lambda^3(q-1)(q-2) + \\
 &\quad 3\lambda^2(q-1)(q-2)(q-3) + 4\lambda^3(q-1) + 6\lambda^2(q-1)(q-2) + 3\lambda(q-1)(q-2)(q-3) + \\
 &\quad (q-1)(q-2)(q-3)(q-4) + 3\lambda(q-1)(q-2) + 4(q-1)(q-2)(q-3) + 4(q-1)(q-2) + q-1. \\
 2Z_C U_C^V &= 3\lambda^9 + 6\lambda^6(q-1) + 3\lambda^5(q-1) + 6\lambda^4(q-1) + 9\lambda^3(q-1)(q-2) + 6\lambda^3(q-1) + 6\lambda^2(q-1)(q-2) + \\
 &\quad 3\lambda(q-1)(q-2)(q-3) + 3\lambda(q-1)(q-2). \\
 6Z_C U_C^N &= 9\lambda^9 + 24\lambda^6(q-1) + 15\lambda^5(q-1) + 12\lambda^4(q-1)(q-2) + 12\lambda^4(q-1) + 27\lambda^3(q-1)(q-2) + \\
 &\quad 6\lambda^2(q-1)(q-2)(q-3) + 12\lambda^3(q-1) + 12\lambda^2(q-1)(q-2) + 3\lambda(q-1)(q-2)(q-3) + 3\lambda(q-1)(q-2). \\
 \tilde{S}_C &= 0. \\
 D_C^U &= 3(2s^4t^7 + 14s^4t^6 + 12s^3t^7 + 42s^4t^5 + 91s^3t^6 + 27s^2t^7 + 70s^4t^4 + 300s^3t^5 + 221s^2t^6 + 27st^7 + 70s^4t^3 + \\
 &\quad 554s^3t^4 + 796s^2t^5 + 237st^6 + 10t^7 + 42s^4t^2 + 616s^3t^3 + 1619s^2t^4 + 928st^5 + 94t^6 + 14s^4t + 411s^3t^2 + \\
 &\quad 1994s^2t^3 + 2071st^4 + 400t^5 + 2s^4 + 152s^3t + 1481s^2t^2 + 2816st^3 + 978t^4 + 24s^3 + 612s^2t + 2325st^2 + \\
 &\quad 1464t^3 + 108s^2 + 1080st + 1341t^2 + 216s + 702t + 162)(s+3)(s+2)(t+1)^4. \\
 D_C^U|_{q=2} &= 6(t^2 + 2t + 2)(t+2)^4(t+1)^4.
 \end{aligned}$$

*Local view 2 of 35.*

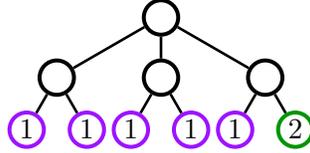

$$\begin{aligned}
 Z_C &= \lambda^8 + \lambda^7 + \lambda^6(q-2) + \lambda^6 + 5\lambda^5(q-2) + \lambda^4(q-2)(q-3) + 5\lambda^5 + 11\lambda^4(q-2) + 10\lambda^3(q-2)(q-3) + \\
 &\quad 2\lambda^2(q-2)(q-3)(q-4) + 5\lambda^4 + 19\lambda^3(q-2) + 15\lambda^2(q-2)(q-3) + 5\lambda(q-2)(q-3)(q-4) + \\
 &\quad (q-2)(q-3)(q-4)(q-5) + \lambda^3 + 15\lambda^2(q-2) + 17\lambda(q-2)(q-3) + 7(q-2)(q-3)(q-4) + \lambda^2 + \\
 &\quad 9\lambda(q-2) + 12(q-2)(q-3) + \lambda + 5q - 10. \\
 2Z_C U_C^V &= 3\lambda^8 + 2\lambda^7 + 2\lambda^6(q-2) + \lambda^6 + 5\lambda^5(q-2) + 8\lambda^5 + 12\lambda^4(q-2) + 6\lambda^3(q-2)(q-3) + 7\lambda^4 + 19\lambda^3(q-2) + \\
 &\quad 12\lambda^2(q-2)(q-3) + 3\lambda(q-2)(q-3)(q-4) + 2\lambda^3 + 16\lambda^2(q-2) + 9\lambda(q-2)(q-3) + \lambda^2 + 3\lambda(q-2).
 \end{aligned}$$

---

*Date:* May 18, 2017.

$$\begin{aligned}
6Z_C U_C^N &= 8\lambda^8 + 7\lambda^7 + 6\lambda^6(q-2) + 6\lambda^6 + 25\lambda^5(q-2) + 4\lambda^4(q-2)(q-3) + 25\lambda^5 + 44\lambda^4(q-2) + \\
&\quad 30\lambda^3(q-2)(q-3) + 4\lambda^2(q-2)(q-3)(q-4) + 20\lambda^4 + 57\lambda^3(q-2) + 30\lambda^2(q-2)(q-3) + \\
&\quad 5\lambda(q-2)(q-3)(q-4) + 3\lambda^3 + 30\lambda^2(q-2) + 17\lambda(q-2)(q-3) + 2\lambda^2 + 9\lambda(q-2) + \lambda. \\
\tilde{S}_C &= (4r^8t^{15} + 60r^8t^{14} + 42r^7t^{15} + 424r^8t^{13} + 662r^7t^{14} + 194r^6t^{15} + 1872r^8t^{12} + 4930r^7t^{13} + 3202r^6t^{14} + 514r^5t^{15} + \\
&\quad 5772r^8t^{11} + 22994r^7t^{12} + 25050r^6t^{13} + 8862r^5t^{14} + 851r^4t^{15} + 13156r^8t^{10} + 75032r^7t^{11} + 123078r^6t^{12} + \\
&\quad 72648r^5t^{13} + 15324r^4t^{14} + 895r^3t^{15} + 22880r^8t^9 + 181196r^7t^{10} + 424020r^6t^{11} + 375096r^5t^{12} + 131468r^4t^{13} + \\
&\quad 16896r^3t^{14} + 576r^2t^{15} + 30888r^8t^8 + 334044r^7t^9 + 1082836r^6t^{10} + 1361314r^5t^{11} + 712016r^4t^{12} + 151828r^3t^{13} + \\
&\quad 11526r^2t^{14} + 202rt^{15} + 32604r^8t^7 + 478020r^7t^8 + 2113148r^6t^9 + 3669346r^5t^{10} + 2716791r^4t^{11} + 861812r^3t^{12} + \\
&\quad 108975r^2t^{13} + 4396rt^{14} + 28t^{15} + 26884r^8t^6 + 534618r^7t^7 + 3202540r^6t^8 + 7568730r^5t^9 + 7715100r^4t^{10} + \\
&\quad 3451813r^3t^{11} + 648892r^2t^{12} + 44221rt^{13} + 704t^{14} + 17160r^8t^5 + 466734r^7t^6 + 3793562r^6t^7 + 12135518r^5t^8 + \\
&\quad 16794876r^4t^9 + 10309598r^3t^{10} + 2725907r^2t^{11} + 277292rt^{12} + 7710t^{13} + 8320r^8t^4 + 315146r^7t^5 + 3507018r^6t^6 + \\
&\quad 15216656r^5t^7 + 28456722r^4t^8 + 23648956r^3t^9 + 8550366r^2t^{10} + 1222221rt^{11} + 51336t^{12} + 2964r^8t^3 + \\
&\quad 161482r^7t^4 + 2506578r^6t^5 + 14895064r^5t^6 + 37743412r^4t^7 + 42293290r^3t^8 + 20637616r^2t^9 + 4022318rt^{10} + \\
&\quad 237894t^{11} + 732r^8t^2 + 60740r^7t^3 + 1358926r^6t^4 + 11273998r^5t^5 + 39109440r^4t^6 + 59288290r^3t^7 + \\
&\quad 38909474r^2t^8 + 10202454rt^9 + 821076t^{10} + 112r^8t + 15824r^7t^2 + 540560r^6t^3 + 6473218r^5t^4 + 31355250r^4t^5 + \\
&\quad 65005470r^3t^6 + 57600846r^2t^7 + 20256420rt^8 + 2186316t^9 + 8r^8 + 2552r^7t + 148864r^6t^2 + 2727300r^5t^3 + \\
&\quad 19081926r^4t^4 + 55206558r^3t^5 + 66794490r^2t^6 + 31642596rt^7 + 4566960t^8 + 192r^7 + 25368r^6t + 795600r^5t^2 + \\
&\quad 8527320r^4t^3 + 35630622r^3t^4 + 60082830r^2t^5 + 38788956rt^6 + 7523064t^7 + 2016r^6 + 143640r^5t + 2640600r^4t^2 + \\
&\quad 16909452r^3t^3 + 41140170r^2t^4 + 36949770rt^5 + 9745272t^6 + 12096r^5 + 506520r^4t + 5569776r^3t^2 + 20755440r^2t^3 + \\
&\quad 26847126rt^4 + 9829350t^5 + 45360r^4 + 1138536r^3t + 7286112r^2t^2 + 14409900rt^3 + 7579170t^4 + 108864r^3 + \\
&\quad 1592136r^2t + 5400432rt^2 + 4330260t^3 + 163296r^2 + 1265544rt + 1735020t^2 + 139968r + 437400t + 52488)(t+1)^2t.
\end{aligned}$$

$$\tilde{S}_C|_{q=2} = 4(t^2 + t + 1)(t + 2)^9(t + 1)^2t.$$

$$\begin{aligned}
D_C^U &= (6s^5t^{10} + 60s^5t^9 + 42s^4t^{10} + 270s^5t^8 + 449s^4t^9 + 117s^3t^{10} + 720s^5t^7 + 2163s^4t^8 + 1336s^3t^9 + 162s^2t^{10} + \\
&\quad 1260s^5t^6 + 6181s^4t^7 + 6875s^3t^8 + 1972s^2t^9 + 111st^{10} + 1512s^5t^5 + 11599s^4t^6 + 20997s^3t^7 + 10815s^2t^8 + \\
&\quad 1439st^9 + 30t^{10} + 1260s^5t^4 + 14931s^4t^5 + 42146s^3t^6 + 35222s^2t^7 + 8398st^8 + 414t^9 + 720s^5t^3 + \\
&\quad 13349s^4t^4 + 58090s^3t^5 + 75472s^2t^6 + 29118st^7 + 2568t^8 + 270s^5t^2 + 8183s^4t^3 + 55671s^3t^4 + 111207s^2t^5 + \\
&\quad 66507st^6 + 9468t^7 + 60s^5t + 3291s^4t^2 + 36625s^3t^3 + 114140s^2t^4 + 104641st^5 + 23030t^6 + 6s^5 + 784s^4t + \\
&\quad 15827s^3t^2 + 80595s^2t^3 + 114932st^4 + 38665t^5 + 84s^4 + 4056s^3t + 37479s^2t^2 + 87087st^3 + 45420t^4 + \\
&\quad 468s^3 + 10368s^2t + 43623st^2 + 36918t^3 + 1296s^2 + 13068st + 19926t^2 + 1782s + 6480t + 972)(s + 3)(t + 1).
\end{aligned}$$

$$D_C^U|_{q=2} = 2(3t^4 + 12t^3 + 20t^2 + 16t + 6)(t + 2)^4(t + 1).$$

Local view 3 of 35.

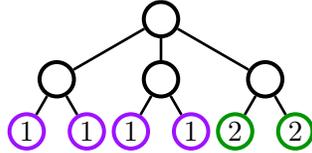

$$\begin{aligned}
Z_C &= \lambda^8 + 2\lambda^7 + 2\lambda^6(q-2) + 2\lambda^6 + 7\lambda^5(q-2) + 3\lambda^4(q-2)(q-3) + 3\lambda^5 + 11\lambda^4(q-2) + 9\lambda^3(q-2)(q-3) + \\
&\quad 3\lambda^2(q-2)(q-3)(q-4) + 3\lambda^4 + 14\lambda^3(q-2) + 15\lambda^2(q-2)(q-3) + 3\lambda(q-2)(q-3)(q-4) + \\
&\quad (q-2)(q-3)(q-4)(q-5) + 2\lambda^3 + 14\lambda^2(q-2) + 12\lambda(q-2)(q-3) + 8(q-2)(q-3)(q-4) + 2\lambda^2 + \\
&\quad 10\lambda(q-2) + 16(q-2)(q-3) + \lambda + 7q - 14.
\end{aligned}$$

$$\begin{aligned}
2Z_C U_C^V &= 2\lambda^8 + 4\lambda^7 + 2\lambda^6(q-2) + 4\lambda^6 + 7\lambda^5(q-2) + 5\lambda^5 + 14\lambda^4(q-2) + 9\lambda^3(q-2)(q-3) + 4\lambda^4 + 16\lambda^3(q-2) + \\
&\quad 6\lambda^2(q-2)(q-3) + 3\lambda(q-2)(q-3)(q-4) + 2\lambda^3 + 8\lambda^2(q-2) + 12\lambda(q-2)(q-3) + 2\lambda^2 + 10\lambda(q-2) + \lambda.
\end{aligned}$$

$$\begin{aligned}
6Z_C U_C^N &= 8\lambda^8 + 14\lambda^7 + 12\lambda^6(q-2) + 12\lambda^6 + 35\lambda^5(q-2) + 12\lambda^4(q-2)(q-3) + 15\lambda^5 + 44\lambda^4(q-2) + \\
&\quad 27\lambda^3(q-2)(q-3) + 6\lambda^2(q-2)(q-3)(q-4) + 12\lambda^4 + 42\lambda^3(q-2) + 30\lambda^2(q-2)(q-3) + \\
&\quad 3\lambda(q-2)(q-3)(q-4) + 6\lambda^3 + 28\lambda^2(q-2) + 12\lambda(q-2)(q-3) + 4\lambda^2 + 10\lambda(q-2) + \lambda.
\end{aligned}$$

$$\begin{aligned} \tilde{S}_C &= 2(4r^4t^9 + 36r^4t^8 + 27r^3t^9 + 144r^4t^7 + 252r^3t^8 + 69r^2t^9 + 336r^4t^6 + 1053r^3t^7 + 666r^2t^8 + 79rt^9 + 504r^4t^5 + \\ &\quad 2586r^3t^6 + 2895r^2t^7 + 786rt^8 + 34t^9 + 504r^4t^4 + 4113r^3t^5 + 7446r^2t^6 + 3540rt^7 + 348t^8 + 336r^4t^3 + \\ &\quad 4392r^3t^4 + 12495r^2t^5 + 9496rt^6 + 1620t^7 + 144r^4t^2 + 3147r^3t^3 + 14190r^2t^4 + 16746rt^5 + 4520t^6 + 36r^4t + \\ &\quad 1458r^3t^2 + 10905r^2t^3 + 20154rt^4 + 8352t^5 + 4r^4 + 396r^3t + 5466r^2t^2 + 16569rt^3 + 10620t^4 + 48r^3 + 1620r^2t + \\ &\quad 8982rt^2 + 9315t^3 + 216r^2 + 2916rt + 5454t^2 + 432r + 1944t + 324)(r^4t^7 + 8r^4t^6 + 4r^3t^7 + 27r^4t^5 + 40r^3t^6 + \\ &\quad 6r^2t^7 + 50r^4t^4 + 164r^3t^5 + 76r^2t^6 + 5rt^7 + 55r^4t^3 + 360r^3t^4 + 370r^2t^5 + 68rt^6 + 2t^7 + 36r^4t^2 + 460r^3t^3 + \\ &\quad 948r^2t^4 + 373rt^5 + 24t^6 + 13r^4t + 344r^3t^2 + 1402r^2t^3 + 1090rt^4 + 141t^5 + 2r^4 + 140r^3t + 1204r^2t^2 + \\ &\quad 1848rt^3 + 462t^4 + 24r^3 + 558r^2t + 1824rt^2 + 891t^3 + 108r^2 + 972rt + 1008t^2 + 216r + 621t + 162)(t+2)t. \end{aligned}$$

$$\tilde{S}_C|_{q=2} = 2(t^2 + 2t + 2)^3(t+2)^9t.$$

$$\begin{aligned} D_C^U &= (6s^5t^{11} + 66s^5t^{10} + 44s^4t^{11} + 330s^5t^9 + 501s^4t^{10} + 130s^3t^{11} + 990s^5t^8 + 2612s^4t^9 + 1524s^3t^{10} + 193s^2t^{11} + \\ &\quad 1980s^5t^7 + 8224s^4t^8 + 8238s^3t^9 + 2316s^2t^{10} + 143st^{11} + 2772s^5t^6 + 17360s^4t^7 + 27073s^3t^8 + 12904s^2t^9 + \\ &\quad 1749st^{10} + 42t^{11} + 2772s^5t^5 + 25774s^4t^6 + 60024s^3t^7 + 44023s^2t^8 + 9996st^9 + 522t^{10} + 1980s^5t^4 + \\ &\quad 27440s^4t^5 + 94143s^3t^6 + 102037s^2t^7 + 35230st^8 + 3048t^9 + 990s^5t^3 + 20932s^4t^4 + 106442s^3t^5 + \\ &\quad 168439s^2t^6 + 84987st^7 + 11048t^8 + 330s^5t^2 + 11204s^4t^3 + 86643s^3t^4 + 201738s^2t^5 + 147118st^6 + 27618t^7 + \\ &\quad 66s^5t + 4005s^4t^2 + 49698s^3t^3 + 175033s^2t^4 + 186160st^5 + 49947t^6 + 6s^5 + 860s^4t + 19109s^3t^2 + \\ &\quad 107664s^2t^3 + 171928st^4 + 66586t^5 + 84s^4 + 4428s^3t + 44661s^2t^2 + 113448st^3 + 65352t^4 + 468s^3 + \\ &\quad 11232s^2t + 50913st^2 + 46260t^3 + 1296s^2 + 13986st + 22518t^2 + 1782s + 6804t + 972)(s+3). \end{aligned}$$

$$D_C^U|_{q=2} = 2(2t^2 + 4t + 3)(t^2 + 2t + 2)(t+2)^4.$$

Local view 4 of 35.

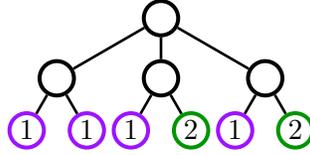

$$\begin{aligned} Z_C &= \lambda^7 + 3\lambda^6 + 2\lambda^5(q-2) + 4\lambda^5 + 15\lambda^4(q-2) + 7\lambda^3(q-2)(q-3) + \lambda^2(q-2)(q-3)(q-4) + 4\lambda^4 + \\ &\quad 18\lambda^3(q-2) + 21\lambda^2(q-2)(q-3) + 7\lambda(q-2)(q-3)(q-4) + (q-2)(q-3)(q-4)(q-5) + 3\lambda^3 + \\ &\quad 20\lambda^2(q-2) + 18\lambda(q-2)(q-3) + 6(q-2)(q-3)(q-4) + \lambda^2 + 7\lambda(q-2) + 9(q-2)(q-3) + 3q - 6. \\ 2Z_C U_C^v &= 3\lambda^7 + 6\lambda^6 + 4\lambda^5(q-2) + 6\lambda^5 + 14\lambda^4(q-2) + 3\lambda^3(q-2)(q-3) + 6\lambda^4 + 24\lambda^3(q-2) + 18\lambda^2(q-2)(q-3) + \\ &\quad 3\lambda(q-2)(q-3)(q-4) + 3\lambda^3 + 14\lambda^2(q-2) + 6\lambda(q-2)(q-3) + \lambda(q-2). \\ 6Z_C U_C^N &= 7\lambda^7 + 18\lambda^6 + 10\lambda^5(q-2) + 20\lambda^5 + 60\lambda^4(q-2) + 21\lambda^3(q-2)(q-3) + 2\lambda^2(q-2)(q-3)(q-4) + 16\lambda^4 + \\ &\quad 54\lambda^3(q-2) + 42\lambda^2(q-2)(q-3) + 7\lambda(q-2)(q-3)(q-4) + 9\lambda^3 + 40\lambda^2(q-2) + 18\lambda(q-2)(q-3) + \\ &\quad 2\lambda^2 + 7\lambda(q-2). \end{aligned}$$

$$\begin{aligned} \tilde{S}_C &= 2(2r^8t^{15} + 30r^8t^{14} + 20r^7t^{15} + 212r^8t^{13} + 318r^7t^{14} + 87r^6t^{15} + 936r^8t^{12} + 2385r^7t^{13} + 1466r^6t^{14} + 214r^5t^{15} + \\ & 2886r^8t^{11} + 11188r^7t^{12} + 11658r^6t^{13} + 3831r^5t^{14} + 322r^4t^{15} + 6578r^8t^{10} + 36681r^7t^{11} + 58024r^6t^{12} + \\ & 32319r^5t^{13} + 6177r^4t^{14} + 298r^3t^{15} + 11440r^8t^9 + 88936r^7t^{10} + 201983r^6t^{11} + 170565r^5t^{12} + 55484r^4t^{13} + \\ & 6244r^3t^{14} + 161r^2t^{15} + 15444r^8t^8 + 164526r^7t^9 + 520248r^6t^{10} + 629660r^5t^{11} + 310756r^4t^{12} + 60227r^3t^{13} + \\ & 3822r^2t^{14} + 44rt^{15} + 16302r^8t^7 + 236160r^7t^8 + 1022736r^6t^9 + 1720691r^5t^{10} + 1215887r^4t^{11} + 359076r^3t^{12} + \\ & 40197r^2t^{13} + 1274rt^{14} + 4t^{15} + 13442r^8t^6 + 264846r^7t^7 + 1560072r^6t^8 + 3590661r^5t^9 + 3521231r^4t^{10} + \\ & 1489548r^3t^{11} + 256633r^2t^{12} + 14992rt^{13} + 172t^{14} + 8580r^8t^5 + 231782r^7t^6 + 1858797r^6t^7 + 5816311r^5t^8 + \\ & 7790635r^4t^9 + 4567498r^3t^{10} + 1130413r^2t^{11} + 103508rt^{12} + 2372t^{13} + 4160r^8t^4 + 156837r^7t^5 + 1727442r^6t^6 + \\ & 7360789r^5t^7 + 13388834r^4t^8 + 10701410r^3t^9 + 3668451r^2t^{10} + 485621rt^{11} + 17988t^{12} + 1482r^8t^3 + \\ & 80508r^7t^4 + 1240394r^6t^5 + 7266070r^5t^6 + 17988696r^4t^7 + 19491608r^3t^8 + 9091388r^2t^9 + 1668073rt^{10} + \\ & 90342t^{11} + 366r^8t^2 + 30325r^7t^3 + 675120r^6t^4 + 5541140r^5t^5 + 18862222r^4t^6 + 27783569r^3t^7 + 17529532r^2t^8 + \\ & 4368276rt^9 + 328710t^{10} + 56r^8t + 7908r^7t^2 + 269389r^6t^3 + 3202160r^5t^4 + 15286059r^4t^5 + 30939606r^3t^6 + \\ & 26486622r^2t^7 + 8905641rt^8 + 908856t^9 + 4r^8 + 1276r^7t + 74348r^6t^2 + 1356117r^5t^3 + 9390348r^4t^4 + \\ & 26655057r^3t^5 + 31312386r^2t^6 + 14250276rt^7 + 1956834t^8 + 96r^7 + 12684r^6t + 397044r^5t^2 + 4228425r^4t^3 + \\ & 17423676r^3t^4 + 28681668r^2t^5 + 17874702rt^6 + 3312711t^7 + 1008r^6 + 71820r^5t + 1316520r^4t^2 + 8356311r^3t^3 + \\ & 19965096r^2t^4 + 17407062rt^5 + 4406076t^6 + 6048r^5 + 253260r^4t + 2773548r^3t^2 + 10213695r^2t^3 + \\ & 12910104rt^4 + 4560867t^5 + 22680r^4 + 569268r^3t + 3622644r^2t^2 + 7054047rt^3 + 3605148t^4 + 54432r^3 + \\ & 796068r^2t + 2679804rt^2 + 2106081t^3 + 81648r^2 + 632772rt + 858762t^2 + 69984r + 218700t + 26244)(t+1)^2t. \end{aligned}$$

$$\tilde{S}_C|_{q=2} = 2(t^2 + 2t + 2)(t+2)^9(t+1)^2t.$$

$$\begin{aligned} D_C^U &= (6s^5t^9 + 54s^5t^8 + 38s^4t^9 + 216s^5t^7 + 377s^4t^8 + 95s^3t^9 + 504s^5t^6 + 1656s^4t^7 + 1037s^3t^8 + 118s^2t^9 + \\ & 756s^5t^5 + 4231s^4t^6 + 4986s^3t^7 + 1405s^2t^8 + 73st^9 + 756s^5t^4 + 6934s^4t^5 + 13903s^3t^6 + 7356s^2t^7 + 937st^8 + \\ & 18t^9 + 504s^5t^3 + 7563s^4t^4 + 24835s^3t^5 + 22309s^2t^6 + 5310st^7 + 246t^8 + 216s^5t^2 + 5492s^4t^3 + 29523s^3t^4 + \\ & 43336s^2t^5 + 17450st^6 + 1500t^7 + 54s^5t + 2561s^4t^2 + 23384s^3t^3 + 56085s^2t^4 + 36767st^5 + 5320t^6 + 6s^5 + \\ & 696s^4t + 11909s^3t^2 + 48486s^2t^3 + 51720st^4 + 12118t^5 + 84s^4 + 3540s^3t + 27057s^2t^2 + 48792st^3 + 18477t^4 + \\ & 468s^3 + 8856s^2t + 29907st^2 + 18990t^3 + 1296s^2 + 10854st + 12798t^2 + 1782s + 5184t + 972)(s+3)(t+1)^2. \end{aligned}$$

$$D_C^U|_{q=2} = 6(t^2 + 2t + 2)(t+2)^4(t+1)^2.$$

Local view 5 of 35.

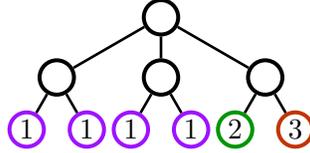

$$\begin{aligned} Z_C &= 3\lambda^7 + \lambda^6(q-3) + 2\lambda^6 + 3\lambda^5(q-3) + \lambda^4(q-3)(q-4) + 6\lambda^5 + 19\lambda^4(q-3) + 10\lambda^3(q-3)(q-4) + \\ & 2\lambda^2(q-3)(q-4)(q-5) + 24\lambda^4 + 35\lambda^3(q-3) + 21\lambda^2(q-3)(q-4) + 5\lambda(q-3)(q-4)(q-5) + \\ & (q-3)(q-4)(q-5)(q-6) + 14\lambda^3 + 41\lambda^2(q-3) + 32\lambda(q-3)(q-4) + 11(q-3)(q-4)(q-5) + 12\lambda^2 + \\ & 49\lambda(q-3) + 33(q-3)(q-4) + 18\lambda + 27q - 79. \end{aligned}$$

$$\begin{aligned} 2Z_C U_C^v &= 7\lambda^7 + 2\lambda^6(q-3) + 2\lambda^6 + \lambda^5(q-3) + 8\lambda^5 + 20\lambda^4(q-3) + 6\lambda^3(q-3)(q-4) + 30\lambda^4 + 31\lambda^3(q-3) + \\ & 12\lambda^2(q-3)(q-4) + 3\lambda(q-3)(q-4)(q-5) + 16\lambda^3 + 32\lambda^2(q-3) + 18\lambda(q-3)(q-4) + 10\lambda^2 + 25\lambda(q-3) + 8\lambda. \end{aligned}$$

$$\begin{aligned} 6Z_C U_C^N &= 21\lambda^7 + 6\lambda^6(q-3) + 12\lambda^6 + 15\lambda^5(q-3) + 4\lambda^4(q-3)(q-4) + 30\lambda^5 + 76\lambda^4(q-3) + 30\lambda^3(q-3)(q-4) + \\ & 4\lambda^2(q-3)(q-4)(q-5) + 96\lambda^4 + 105\lambda^3(q-3) + 42\lambda^2(q-3)(q-4) + 5\lambda(q-3)(q-4)(q-5) + 42\lambda^3 + \\ & 82\lambda^2(q-3) + 32\lambda(q-3)(q-4) + 24\lambda^2 + 49\lambda(q-3) + 18\lambda. \end{aligned}$$

$$\begin{aligned}
 \tilde{S}_C &= 2(6r^7t^{14} + 88r^7t^{13} + 58r^6t^{14} + 600r^7t^{12} + 902r^6t^{13} + 242r^5t^{14} + 2520r^7t^{11} + 6522r^6t^{12} + 3986r^5t^{13} + 568r^4t^{14} + \\
 &7282r^7t^{10} + 29044r^6t^{11} + 30502r^5t^{12} + 9882r^4t^{13} + 817r^3t^{14} + 15312r^7t^9 + 88950r^6t^{10} + 143666r^5t^{11} + \\
 &79780r^4t^{12} + 14927r^3t^{13} + 729r^2t^{14} + 24156r^7t^8 + 198108r^6t^9 + 465130r^5t^{10} + 396172r^4t^{11} + 126492r^3t^{12} + \\
 &13834r^2t^{13} + 378rt^{14} + 29040r^7t^7 + 330792r^6t^8 + 1094660r^5t^9 + 1351836r^4t^{10} + 659334r^3t^{11} + 122062r^2t^{12} + \\
 &7328rt^{13} + 88t^{14} + 26730r^7t^6 + 420576r^6t^7 + 1930768r^5t^8 + 3352802r^4t^9 + 2362335r^3t^{10} + 663832r^2t^{11} + \\
 &66585rt^{12} + 1712t^{13} + 18744r^7t^5 + 409086r^6t^6 + 2592356r^5t^7 + 6232646r^4t^8 + 6155251r^3t^9 + 2485939r^2t^{10} + \\
 &374998rt^{11} + 15834t^{12} + 9856r^7t^4 + 302902r^6t^5 + 2662222r^5t^6 + 8821590r^4t^7 + 12028550r^3t^8 + 6780484r^2t^9 + \\
 &1460034rt^{10} + 91644t^{11} + 3768r^7t^3 + 168050r^6t^4 + 2080858r^5t^5 + 9553402r^4t^6 + 17911252r^3t^7 + \\
 &13890298r^2t^8 + 4152645rt^9 + 369072t^{10} + 990r^7t^2 + 67740r^6t^3 + 1218558r^5t^4 + 7878116r^4t^5 + 20425384r^3t^6 + \\
 &21712632r^2t^7 + 8891904rt^8 + 1090674t^9 + 160r^7t + 18754r^6t^2 + 518442r^5t^3 + 4870194r^4t^4 + 17755560r^3t^5 + \\
 &26030328r^2t^6 + 14558202rt^7 + 2434536t^8 + 12r^7 + 3192r^6t + 151494r^5t^2 + 2188854r^4t^3 + 11585304r^3t^4 + \\
 &23827338r^2t^5 + 18316728rt^6 + 4166100t^7 + 252r^6 + 27216r^5t + 676170r^4t^2 + 5503788r^3t^3 + 16402338r^2t^4 + \\
 &17633430rt^5 + 5491800t^6 + 2268r^5 + 128520r^4t + 1800090r^3t^2 + 8239320r^2t^3 + 12797514rt^4 + 5553036t^5 + \\
 &11340r^4 + 362880r^3t + 2856870r^2t^2 + 6797682rt^3 + 4245210t^4 + 34020r^3 + 612360r^2t + 2501442rt^2 + \\
 &2383830t^3 + 61236r^2 + 571536rt + 931662t^2 + 61236r + 227448t + 26244)(rt^2 + 2rt + t^2 + r + 3t + 3)(t + 1)t. \\
 D_C^U &= (6s^5t^{10} + 60s^5t^9 + 38s^4t^{10} + 270s^5t^8 + 409s^4t^9 + 94s^3t^{10} + 720s^5t^7 + 1987s^4t^8 + 1085s^3t^9 + 112s^2t^{10} + \\
 &1260s^5t^6 + 5733s^4t^7 + 5673s^3t^8 + 1379s^2t^9 + 62st^{10} + 1512s^5t^5 + 10871s^4t^6 + 17675s^3t^7 + 7739s^2t^8 + \\
 &814st^9 + 12t^{10} + 1260s^5t^4 + 14147s^4t^5 + 36295s^3t^6 + 26036s^2t^7 + 4908st^8 + 168t^9 + 720s^5t^3 + 12789s^4t^4 + \\
 &51267s^3t^5 + 58010s^2t^6 + 17904st^7 + 1092t^8 + 270s^5t^2 + 7927s^4t^3 + 50395s^3t^4 + 89222s^2t^5 + 43578st^6 + \\
 &4376t^7 + 60s^5t + 3223s^4t^2 + 34013s^3t^3 + 95752s^2t^4 + 73556st^5 + 11860t^6 + 6s^5 + 776s^4t + 15075s^3t^2 + \\
 &70719s^2t^3 + 86848st^4 + 22398t^5 + 84s^4 + 3960s^3t + 34383s^2t^2 + 70707st^3 + 29568t^4 + 468s^3 + 9936s^2t + \\
 &38007st^2 + 26874t^3 + 1296s^2 + 12204st + 16146t^2 + 1782s + 5832t + 972)(s + 3)(t + 1).
 \end{aligned}$$

Local view 6 of 35.

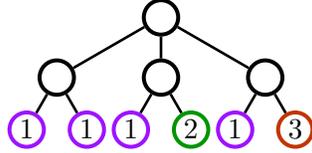

$$\begin{aligned}
 Z_C &= \lambda^7 + 2\lambda^6 + 2\lambda^5(q-3) + 9\lambda^5 + 14\lambda^4(q-3) + 7\lambda^3(q-3)(q-4) + \lambda^2(q-3)(q-4)(q-5) + 16\lambda^4 + 36\lambda^3(q-3) + \\
 &24\lambda^2(q-3)(q-4) + 7\lambda(q-3)(q-4)(q-5) + (q-3)(q-4)(q-5)(q-6) + 23\lambda^3 + 56\lambda^2(q-3) + \\
 &39\lambda(q-3)(q-4) + 10(q-3)(q-4)(q-5) + 18\lambda^2 + 47\lambda(q-3) + 27(q-3)(q-4) + 10\lambda + 20q - 58. \\
 2Z_C U_C^v &= 3\lambda^7 + 4\lambda^6 + 4\lambda^5(q-3) + 13\lambda^5 + 12\lambda^4(q-3) + 3\lambda^3(q-3)(q-4) + 22\lambda^4 + 36\lambda^3(q-3) + 18\lambda^2(q-3)(q-4) + \\
 &3\lambda(q-3)(q-4)(q-5) + 23\lambda^3 + 44\lambda^2(q-3) + 15\lambda(q-3)(q-4) + 14\lambda^2 + 15\lambda(q-3) + 2\lambda. \\
 6Z_C U_C^N &= 7\lambda^7 + 12\lambda^6 + 10\lambda^5(q-3) + 45\lambda^5 + 56\lambda^4(q-3) + 21\lambda^3(q-3)(q-4) + 2\lambda^2(q-3)(q-4)(q-5) + 64\lambda^4 + \\
 &108\lambda^3(q-3) + 48\lambda^2(q-3)(q-4) + 7\lambda(q-3)(q-4)(q-5) + 69\lambda^3 + 112\lambda^2(q-3) + 39\lambda(q-3)(q-4) + \\
 &36\lambda^2 + 47\lambda(q-3) + 10\lambda.
 \end{aligned}$$

$$\begin{aligned}
\tilde{S}_C &= 2(4r^8t^{14} + 56r^8t^{13} + 40r^7t^{14} + 366r^8t^{12} + 600r^7t^{13} + 176r^6t^{14} + 1480r^8t^{11} + 4199r^7t^{12} + 2816r^6t^{13} + 445r^5t^{14} + \\
&4136r^8t^{10} + 18169r^7t^{11} + 21018r^6t^{12} + 7564r^5t^{13} + 706r^4t^{14} + 8448r^8t^9 + 54288r^7t^{10} + 96982r^6t^{11} + \\
&59987r^5t^{12} + 12712r^4t^{13} + 718r^3t^{14} + 13002r^8t^8 + 118446r^7t^9 + 308972r^6t^{10} + 294200r^5t^{11} + 106786r^4t^{12} + \\
&13669r^3t^{13} + 455r^2t^{14} + 15312r^8t^7 + 194514r^7t^8 + 718618r^6t^9 + 996614r^5t^{10} + 554989r^4t^{11} + 121337r^3t^{12} + \\
&9155r^2t^{13} + 162rt^{14} + 13860r^8t^6 + 244134r^7t^7 + 1257620r^6t^8 + 2465659r^5t^9 + 1993742r^4t^{10} + 666580r^3t^{11} + \\
&85773r^2t^{12} + 3466rt^{13} + 24t^{14} + 9592r^8t^5 + 235212r^7t^6 + 1681324r^6t^7 + 4591516r^5t^8 + 5235414r^4t^9 + \\
&2533375r^3t^{10} + 497251r^2t^{11} + 34343rt^{12} + 560t^{13} + 4994r^8t^4 + 173032r^7t^5 + 1724480r^6t^6 + 653328r^5t^7 + \\
&10357086r^4t^8 + 7046204r^3t^9 + 1995702r^2t^{10} + 210118rt^{11} + 5922t^{12} + 1896r^8t^3 + 95631r^7t^4 + 1349604r^6t^5 + \\
&7132877r^5t^6 + 15669127r^4t^7 + 14783937r^3t^8 + 5869103r^2t^9 + 889848rt^{10} + 38352t^{11} + 496r^8t^2 + 38489r^7t^3 + \\
&792922r^6t^4 + 5942151r^5t^5 + 18203048r^4t^6 + 23753970r^3t^7 + 13040976r^2t^8 + 2764029rt^9 + 171504t^{10} + 80r^8t + \\
&10660r^7t^2 + 338974r^6t^3 + 3715869r^5t^4 + 16146918r^4t^5 + 29346600r^3t^6 + 22228443r^2t^7 + 6497001rt^8 + \\
&562590t^9 + 6r^8 + 1818r^7t + 99636r^6t^2 + 1690497r^5t^3 + 10758312r^4t^4 + 27720468r^3t^5 + 29185326r^2t^6 + \\
&11737197rt^7 + 1398330t^8 + 144r^7 + 18018r^6t + 528660r^5t^2 + 5217750r^4t^3 + 19693881r^3t^4 + 29352942r^2t^5 + \\
&16367319rt^6 + 2676078t^7 + 1512r^6 + 101682r^5t + 1740420r^4t^2 + 10198683r^3t^3 + 22247946r^2t^4 + \\
&17522973rt^5 + 3961710t^6 + 9072r^5 + 357210r^4t + 3637548r^3t^2 + 12318642r^2t^3 + 14173947rt^4 + \\
&4513968t^5 + 34020r^4 + 799470r^3t + 4709340r^2t^2 + 8400267rt^3 + 3897234t^4 + 81648r^3 + 1112454r^2t + \\
&3449628rt^2 + 2474226t^3 + 122472r^2 + 879174rt + 1093500t^2 + 104976r + 301806t + 39366)(t+1)^3t. \\
D_C^U &= (6s^5t^9 + 54s^5t^8 + 36s^4t^9 + 216s^5t^7 + 361s^4t^8 + 85s^3t^9 + 504s^5t^6 + 1600s^4t^7 + 945s^3t^8 + 99s^2t^9 + 756s^5t^5 + \\
&4119s^4t^6 + 4620s^3t^7 + 1208s^2t^8 + 56st^9 + 756s^5t^4 + 6794s^4t^5 + 13079s^3t^6 + 6476s^2t^7 + 750st^8 + 12t^9 + \\
&504s^5t^3 + 7451s^4t^4 + 23685s^3t^5 + 20091s^2t^6 + 4392st^7 + 180t^8 + 216s^5t^2 + 5436s^4t^3 + 28503s^3t^4 + \\
&39881s^2t^5 + 14873st^6 + 1152t^7 + 54s^5t + 2545s^4t^2 + 22822s^3t^3 + 52676s^2t^4 + 32282st^5 + 4238t^6 + 6s^5 + \\
&694s^4t + 11733s^3t^2 + 46404s^2t^3 + 46778st^4 + 10008t^5 + 84s^4 + 3516s^3t + 26337s^2t^2 + 45426st^3 + 15864t^4 + \\
&468s^3 + 8748s^2t + 28611st^2 + 16992t^3 + 1296s^2 + 10638st + 11934t^2 + 1782s + 5022t + 972)(s+3)(t+1)^2.
\end{aligned}$$

Local view 7 of 35.

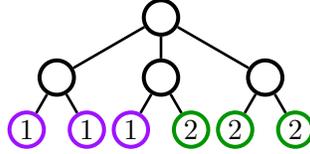

$$\begin{aligned}
Z_C &= 2\lambda^7 + 4\lambda^6 + 7\lambda^5(q-2) + \lambda^4(q-2)(q-3) + 2\lambda^5 + 12\lambda^4(q-2) + 10\lambda^3(q-2)(q-3) + 2\lambda^2(q-2)(q-3)(q-4) + \\
&2\lambda^4 + 15\lambda^3(q-2) + 15\lambda^2(q-2)(q-3) + 5\lambda(q-2)(q-3)(q-4) + (q-2)(q-3)(q-4)(q-5) + 4\lambda^3 + \\
&16\lambda^2(q-2) + 17\lambda(q-2)(q-3) + 7(q-2)(q-3)(q-4) + 2\lambda^2 + 11\lambda(q-2) + 12(q-2)(q-3) + 4q - 8. \\
2Z_C U_C^v &= 4\lambda^7 + 8\lambda^6 + 7\lambda^5(q-2) + 4\lambda^5 + 16\lambda^4(q-2) + 6\lambda^3(q-2)(q-3) + 2\lambda^4 + 15\lambda^3(q-2) + 12\lambda^2(q-2)(q-3) + \\
&3\lambda(q-2)(q-3)(q-4) + 4\lambda^3 + 14\lambda^2(q-2) + 9\lambda(q-2)(q-3) + 2\lambda^2 + 5\lambda(q-2). \\
6Z_C U_C^N &= 14\lambda^7 + 24\lambda^6 + 35\lambda^5(q-2) + 4\lambda^4(q-2)(q-3) + 10\lambda^5 + 48\lambda^4(q-2) + 30\lambda^3(q-2)(q-3) + \\
&4\lambda^2(q-2)(q-3)(q-4) + 8\lambda^4 + 45\lambda^3(q-2) + 30\lambda^2(q-2)(q-3) + 5\lambda(q-2)(q-3)(q-4) + 12\lambda^3 + \\
&32\lambda^2(q-2) + 17\lambda(q-2)(q-3) + 4\lambda^2 + 11\lambda(q-2).
\end{aligned}$$

$$\begin{aligned} \tilde{S}_C &= 2(4r^7t^{14} + 60r^7t^{13} + 38r^6t^{14} + 420r^7t^{12} + 602r^6t^{13} + 154r^5t^{14} + 1816r^7t^{11} + 4460r^6t^{12} + 2582r^5t^{13} + \\ &\quad 347r^4t^{14} + 5412r^7t^{10} + 20440r^6t^{11} + 20256r^5t^{12} + 6160r^4t^{13} + 472r^3t^{14} + 11748r^7t^9 + 64620r^6t^{10} + \\ &\quad 98330r^5t^{11} + 51139r^4t^{12} + 8865r^3t^{13} + 390r^2t^{14} + 19140r^7t^8 + 148848r^6t^9 + 329320r^5t^{10} + 262580r^4t^{11} + \\ &\quad 77743r^3t^{12} + 7733r^2t^{13} + 183rt^{14} + 23760r^7t^7 + 257292r^6t^8 + 803624r^5t^9 + 929933r^4t^{10} + 421286r^3t^{11} + \\ &\quad 71408r^2t^{12} + 3808rt^{13} + 38t^{14} + 22572r^7t^6 + 338712r^6t^7 + 1471540r^5t^8 + 2399420r^4t^9 + 1573944r^3t^{10} + \\ &\quad 407025r^2t^{11} + 36814rt^{12} + 820t^{13} + 16324r^7t^5 + 340998r^6t^6 + 2051924r^5t^7 + 4645999r^4t^8 + 4284089r^3t^9 + \\ &\quad 1599239r^2t^{10} + 219669rt^{11} + 8228t^{12} + 8844r^7t^4 + 261122r^6t^5 + 2187730r^5t^6 + 6851974r^4t^7 + 8753443r^3t^8 + \\ &\quad 4579412r^2t^9 + 904252rt^{10} + 51094t^{11} + 3480r^7t^3 + 149660r^6t^4 + 1773798r^5t^5 + 7729240r^4t^6 + 13630488r^3t^7 + \\ &\quad 9850467r^2t^8 + 2715769rt^9 + 219468t^{10} + 940r^7t^2 + 62240r^6t^3 + 1076160r^5t^4 + 6633028r^4t^5 + 16247086r^3t^6 + \\ &\quad 16163688r^2t^7 + 6134631rt^8 + 689322t^9 + 156r^7t + 17752r^6t^2 + 473618r^5t^3 + 4261338r^4t^4 + 14747784r^3t^5 + \\ &\quad 20328300r^2t^6 + 10586070rt^7 + 1631466t^8 + 12r^7 + 3108r^6t + 142908r^5t^2 + 1986834r^4t^3 + 10033272r^3t^4 + \\ &\quad 19499346r^2t^5 + 14024340rt^6 + 2954988t^7 + 252r^6 + 26460r^5t + 635400r^4t^2 + 4960188r^3t^3 + 14044428r^2t^4 + \\ &\quad 14199246rt^5 + 4117014t^6 + 2268r^5 + 124740r^4t + 1684260r^3t^2 + 7366356r^2t^3 + 10821276rt^4 + 4394088t^5 + \\ &\quad 11340r^4 + 351540r^3t + 2660040r^2t^2 + 6023322rt^3 + 3540510t^4 + 34020r^3 + 591948r^2t + 2316276rt^2 + \\ &\quad 2091258t^3 + 61236r^2 + 551124rt + 857304t^2 + 61236r + 218700t + 26244)(rt^2 + 2rt + t^2 + r + 3t + 3)(t + 1)t. \end{aligned}$$

$$\tilde{S}_C|_{q=2} = 4(t^4 + 3t^3 + 6t^2 + 6t + 3)(t + 2)^9(t + 1)t.$$

$$\begin{aligned} D_C^U &= (6s^4t^8 + 48s^4t^7 + 34s^3t^8 + 168s^4t^6 + 293s^3t^7 + 72s^2t^8 + 336s^4t^5 + 1107s^3t^6 + 666s^2t^7 + 68st^8 + 420s^4t^4 + \\ &\quad 2396s^3t^5 + 2697s^2t^6 + 667st^7 + 24t^8 + 336s^4t^3 + 3250s^3t^4 + 6267s^2t^5 + 2862st^6 + 246t^7 + 168s^4t^2 + \\ &\quad 2829s^3t^3 + 9165s^2t^4 + 7073st^5 + 1104t^6 + 48s^4t + 1543s^3t^2 + 8655s^2t^3 + 11077st^4 + 2870t^5 + 6s^4 + \\ &\quad 482s^3t + 5160s^2t^2 + 11310st^3 + 4774t^4 + 66s^3 + 1776s^2t + 7383st^2 + 5250t^3 + 270s^2 + 2826st + 376t^2 + \\ &\quad 486s + 1620t + 324)(st^2 + 2st + t^2 + s + 3t + 3)(s + 3)(t + 1). \end{aligned}$$

$$D_C^U|_{q=2} = 4(2t^2 + 4t + 3)(t + 2)^4(t + 1).$$

Local view 8 of 35 (named  $C_2$ ).

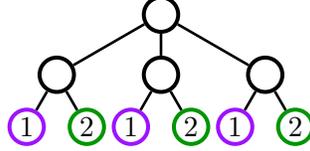

$$\begin{aligned} Z_C &= 2\lambda^6 + 6\lambda^5 + 6\lambda^4(q - 2) + 6\lambda^4 + 39\lambda^3(q - 2) + 33\lambda^2(q - 2)(q - 3) + 9\lambda(q - 2)(q - 3)(q - 4) + \\ &\quad (q - 2)(q - 3)(q - 4)(q - 5) + 2\lambda^3 + 12\lambda^2(q - 2) + 15\lambda(q - 2)(q - 3) + 5(q - 2)(q - 3)(q - 4) + 6\lambda(q - 2) + \\ &\quad 7(q - 2)(q - 3) + 2q - 4. \end{aligned}$$

$$2Z_C U_C^v = 6\lambda^6 + 12\lambda^5 + 12\lambda^4(q - 2) + 6\lambda^4 + 39\lambda^3(q - 2) + 24\lambda^2(q - 2)(q - 3) + 3\lambda(q - 2)(q - 3)(q - 4) + 6\lambda^2(q - 2) + 3\lambda(q - 2)(q - 3).$$

$$6Z_C U_C^N = 12\lambda^6 + 30\lambda^5 + 24\lambda^4(q - 2) + 24\lambda^4 + 117\lambda^3(q - 2) + 66\lambda^2(q - 2)(q - 3) + 9\lambda(q - 2)(q - 3)(q - 4) + 6\lambda^3 + 24\lambda^2(q - 2) + 15\lambda(q - 2)(q - 3) + 6\lambda(q - 2).$$

$$\tilde{S}_C = 0.$$

$$\begin{aligned} D_C^U &= 3(2s^5t^8 + 16s^5t^7 + 12s^4t^8 + 56s^5t^6 + 109s^4t^7 + 28s^3t^8 + 112s^5t^5 + 429s^4t^6 + 289s^3t^7 + 32s^2t^8 + 140s^5t^4 + \\ &\quad 958s^4t^5 + 1277s^3t^6 + 372s^2t^7 + 18st^8 + 112s^5t^3 + 1330s^4t^4 + 3178s^3t^5 + 1840s^2t^6 + 232st^7 + 4t^8 + 56s^5t^2 + \\ &\quad 1177s^4t^3 + 4898s^3t^4 + 5097s^2t^5 + 1280st^6 + 56t^7 + 16s^5t + 649s^4t^2 + 4805s^3t^3 + 8715s^2t^4 + 3943st^5 + \\ &\quad 344t^6 + 2s^5 + 204s^4t + 2937s^3t^2 + 9487s^2t^3 + 7471st^4 + 1178t^5 + 28s^4 + 1024s^3t + 6457s^2t^2 + 9019st^3 + \\ &\quad 2466t^4 + 156s^3 + 2520s^2t + 6855st^2 + 3288t^3 + 432s^2 + 3024st + 2790t^2 + 594s + 1404t + 324)(s + 3)(t + 1)^3. \end{aligned}$$

$$D_C^U|_{q=2} = 12(t + 2)^4(t + 1)^3.$$

Local view 9 of 35.

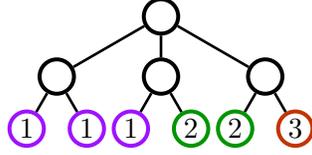

$$\begin{aligned}
Z_C &= 4\lambda^6 + \lambda^5(q-3) + 9\lambda^5 + 17\lambda^4(q-3) + 7\lambda^3(q-3)(q-4) + \lambda^2(q-3)(q-4)(q-5) + 15\lambda^4 + 34\lambda^3(q-3) + \\
&\quad 24\lambda^2(q-3)(q-4) + 7\lambda(q-3)(q-4)(q-5) + (q-3)(q-4)(q-5)(q-6) + 22\lambda^3 + 54\lambda^2(q-3) + \\
&\quad 39\lambda(q-3)(q-4) + 10(q-3)(q-4)(q-5) + 18\lambda^2 + 50\lambda(q-3) + 27(q-3)(q-4) + 12\lambda + 19q - 56. \\
2Z_C U_C^v &= 9\lambda^6 + 2\lambda^5(q-3) + 13\lambda^5 + 16\lambda^4(q-3) + 3\lambda^3(q-3)(q-4) + 20\lambda^4 + 36\lambda^3(q-3) + 18\lambda^2(q-3)(q-4) + \\
&\quad 3\lambda(q-3)(q-4)(q-5) + 24\lambda^3 + 40\lambda^2(q-3) + 15\lambda(q-3)(q-4) + 11\lambda^2 + 17\lambda(q-3) + 4\lambda. \\
6Z_C U_C^N &= 24\lambda^6 + 5\lambda^5(q-3) + 45\lambda^5 + 68\lambda^4(q-3) + 21\lambda^3(q-3)(q-4) + 2\lambda^2(q-3)(q-4)(q-5) + 60\lambda^4 + \\
&\quad 102\lambda^3(q-3) + 48\lambda^2(q-3)(q-4) + 7\lambda(q-3)(q-4)(q-5) + 66\lambda^3 + 108\lambda^2(q-3) + 39\lambda(q-3)(q-4) + \\
&\quad 36\lambda^2 + 50\lambda(q-3) + 12\lambda. \\
\tilde{S}_C &= (12r^8t^{15} + 184r^8t^{14} + 122r^7t^{15} + 1320r^8t^{13} + 1992r^7t^{14} + 544r^6t^{15} + 5876r^8t^{12} + 15210r^7t^{13} + 9440r^6t^{14} + \\
&\quad 1393r^5t^{15} + 18148r^8t^{11} + 72024r^7t^{12} + 76538r^6t^{13} + 25621r^5t^{14} + 2245r^4t^{15} + 41184r^8t^{10} + 236472r^7t^{11} + \\
&\quad 384604r^6t^{12} + 219969r^5t^{13} + 43624r^4t^{14} + 2338r^3t^{15} + 70928r^8t^9 + 570044r^7t^{10} + 1339354r^6t^{11} + \\
&\quad 1169849r^5t^{12} + 395367r^4t^{13} + 47785r^3t^{14} + 1542r^2t^{15} + 94380r^8t^8 + 1041984r^7t^9 + 3423180r^6t^{10} + \\
&\quad 4310637r^5t^{11} + 2218972r^4t^{12} + 455499r^3t^{13} + 32926r^2t^{14} + 590rt^{15} + 97812r^8t^7 + 1470240r^7t^8 + \\
&\quad 6631728r^6t^9 + 11657023r^5t^{10} + 8629373r^4t^{11} + 2689500r^3t^{12} + 328617r^2t^{13} + 13048rt^{14} + 100t^{15} + \\
&\quad 78936r^8t^6 + 1614138r^7t^7 + 9913608r^6t^8 + 23896081r^5t^9 + 24636774r^4t^{10} + 11009206r^3t^{11} + 2034488r^2t^{12} + \\
&\quad 135646rt^{13} + 2272t^{14} + 49192r^8t^5 + 1378544r^7t^6 + 11526036r^6t^7 + 37802919r^5t^8 + 53345249r^4t^9 + \\
&\quad 33108193r^3t^{10} + 8742594r^2t^{11} + 877585rt^{12} + 24480t^{13} + 23244r^8t^4 + 908202r^7t^5 + 10419640r^6t^6 + \\
&\quad 46517906r^5t^7 + 89191552r^4t^8 + 75581141r^3t^9 + 27633528r^2t^{10} + 3949192rt^{11} + 164994t^{12} + 8060r^8t^3 + \\
&\quad 453192r^7t^4 + 7262426r^6t^5 + 44512308r^5t^6 + 116070972r^4t^7 + 133368090r^3t^8 + 66387341r^2t^9 + \\
&\quad 13093898rt^{10} + 775944t^{11} + 1936r^8t^2 + 165780r^7t^3 + 3831788r^6t^4 + 32840950r^5t^5 + 117535058r^4t^6 + \\
&\quad 183375982r^3t^7 + 123452570r^2t^8 + 33050346rt^9 + 2694588t^{10} + 288r^8t + 41964r^7t^2 + 1481170r^6t^3 + \\
&\quad 18341500r^5t^4 + 91824204r^4t^5 + 196417116r^3t^6 + 179152290r^2t^7 + 64680591rt^8 + 7136856t^9 + 20r^8 + \\
&\quad 6572r^7t + 395932r^6t^2 + 7504140r^5t^3 + 54335520r^4t^4 + 162509274r^3t^5 + 202857912r^2t^6 + 98961318rt^7 + \\
&\quad 14682726t^8 + 480r^7 + 65436r^6t + 2122812r^5t^2 + 23566050r^4t^3 + 101961792r^3t^4 + 177733062r^2t^5 + \\
&\quad 118376208rt^6 + 23662314t^7 + 5040r^6 + 371196r^5t + 7070220r^4t^2 + 46945980r^3t^3 + 118302876r^2t^4 + \\
&\quad 109802790rt^5 + 29879766t^6 + 30240r^5 + 1311660r^4t + 14969988r^3t^2 + 57897990r^2t^3 + 77562684rt^4 + \\
&\quad 29332044t^5 + 113400r^4 + 2955204r^3t + 19664532r^2t^2 + 40391460rt^3 + 21991500t^4 + 272160r^3 + 4143636r^2t + \\
&\quad 14641236rt^2 + 12196170t^3 + 408240r^2 + 3303828rt + 4726836t^2 + 349920r + 1145988t + 131220)(t+1)^2. \\
D_C^U &= (6s^5t^9 + 54s^5t^8 + 34s^4t^9 + 216s^5t^7 + 343s^4t^8 + 74s^3t^9 + 504s^5t^6 + 1530s^4t^7 + 836s^3t^8 + 77s^2t^9 + 756s^5t^5 + \\
&\quad 3965s^4t^6 + 4152s^3t^7 + 965s^2t^8 + 37st^9 + 756s^5t^4 + 6584s^4t^5 + 11941s^3t^6 + 5322s^2t^7 + 514st^8 + 6t^9 + \\
&\quad 504s^5t^3 + 7269s^4t^4 + 21970s^3t^5 + 16997s^2t^6 + 3153st^7 + 96t^8 + 216s^5t^2 + 5338s^4t^3 + 26862s^3t^4 + \\
&\quad 34739s^2t^5 + 11217st^6 + 666t^7 + 54s^5t + 2515s^4t^2 + 21848s^3t^3 + 47241s^2t^4 + 25587st^5 + 2662t^6 + 6s^5 + \\
&\quad 690s^4t + 11405s^3t^2 + 42834s^2t^3 + 38955st^4 + 6826t^5 + 84s^4 + 3468s^3t + 25005s^2t^2 + 39720st^3 + 11745t^4 + \\
&\quad 468s^3 + 8532s^2t + 26235st^2 + 13644t^3 + 1296s^2 + 10206st + 10368t^2 + 1782s + 4698t + 972)(s+3)(t+1)^2.
\end{aligned}$$

Local view 10 of 35.

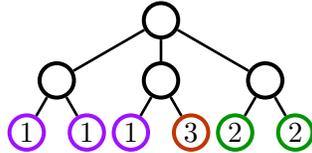

$$\begin{aligned}
 Z_C &= \lambda^7 + 6\lambda^6 + 6\lambda^5(q-3) + \lambda^4(q-3)(q-4) + 9\lambda^5 + 17\lambda^4(q-3) + 10\lambda^3(q-3)(q-4) + \\
 &\quad 2\lambda^2(q-3)(q-4)(q-5) + 13\lambda^4 + 33\lambda^3(q-3) + 21\lambda^2(q-3)(q-4) + 5\lambda(q-3)(q-4)(q-5) + \\
 &\quad (q-3)(q-4)(q-5)(q-6) + 18\lambda^3 + 44\lambda^2(q-3) + 32\lambda(q-3)(q-4) + 11(q-3)(q-4)(q-5) + 18\lambda^2 + \\
 &\quad 48\lambda(q-3) + 33(q-3)(q-4) + 13\lambda + 27q - 78. \\
 2Z_C U_C^v &= 2\lambda^7 + 9\lambda^6 + 5\lambda^5(q-3) + 16\lambda^5 + 20\lambda^4(q-3) + 6\lambda^3(q-3)(q-4) + 16\lambda^4 + 27\lambda^3(q-3) + 12\lambda^2(q-3)(q-4) + \\
 &\quad 3\lambda(q-3)(q-4)(q-5) + 15\lambda^3 + 34\lambda^2(q-3) + 18\lambda(q-3)(q-4) + 17\lambda^2 + 25\lambda(q-3) + 6\lambda. \\
 6Z_C U_C^N &= 7\lambda^7 + 36\lambda^6 + 30\lambda^5(q-3) + 4\lambda^4(q-3)(q-4) + 45\lambda^5 + 68\lambda^4(q-3) + 30\lambda^3(q-3)(q-4) + \\
 &\quad 4\lambda^2(q-3)(q-4)(q-5) + 52\lambda^4 + 99\lambda^3(q-3) + 42\lambda^2(q-3)(q-4) + 5\lambda(q-3)(q-4)(q-5) + 54\lambda^3 + \\
 &\quad 88\lambda^2(q-3) + 32\lambda(q-3)(q-4) + 36\lambda^2 + 48\lambda(q-3) + 13\lambda. \\
 \tilde{S}_C &= (12r^8t^{16} + 204r^8t^{15} + 124r^7t^{16} + 1628r^8t^{14} + 2224r^7t^{15} + 560r^6t^{16} + 8092r^8t^{13} + 18744r^7t^{14} + \\
 &\quad 10598r^6t^{15} + 1449r^5t^{16} + 28028r^8t^{12} + 98452r^7t^{13} + 94258r^6t^{14} + 28902r^5t^{15} + 2360r^4t^{16} + 71708r^8t^{11} + \\
 &\quad 360432r^7t^{12} + 522470r^6t^{13} + 270832r^5t^{14} + 49475r^4t^{15} + 2491r^3t^{16} + 140140r^8t^{10} + 974620r^7t^{11} + \\
 &\quad 2018518r^6t^{12} + 1581392r^5t^{13} + 487190r^4t^{14} + 54609r^3t^{15} + 1672r^2t^{16} + 213356r^8t^9 + 2012516r^7t^{10} + \\
 &\quad 5759548r^6t^{11} + 6435446r^5t^{12} + 2989397r^4t^{13} + 562841r^3t^{14} + 38050r^2t^{15} + 652rt^{16} + 255684r^8t^8 + \\
 &\quad 3235848r^7t^9 + 12548376r^6t^{10} + 19342576r^5t^{11} + 12786028r^4t^{12} + 3617707r^3t^{13} + 408294r^2t^{14} + \\
 &\quad 15296rt^{15} + 112t^{16} + 241956r^8t^7 + 4092924r^7t^8 + 21284460r^6t^9 + 44395064r^5t^{10} + 40401943r^4t^{11} + \\
 &\quad 16220843r^3t^{12} + 2738395r^2t^{13} + 169957rt^{14} + 2704t^{15} + 180180r^8t^6 + 4085224r^7t^7 + 28395276r^6t^8 + \\
 &\quad 79339936r^5t^9 + 97524496r^4t^{10} + 53770313r^3t^{11} + 12834156r^2t^{12} + 1184677rt^{13} + 31002t^{14} + 104468r^8t^5 + \\
 &\quad 3206368r^7t^6 + 29885390r^6t^7 + 111539609r^5t^8 + 183382229r^4t^9 + 136262671r^3t^{10} + 44532146r^2t^{11} + \\
 &\quad 5786935rt^{12} + 223846t^{13} + 46228r^8t^4 + 1957860r^7t^5 + 24726482r^6t^6 + 123728950r^5t^7 + 271397042r^4t^8 + \\
 &\quad 269204933r^3t^9 + 118267914r^2t^{10} + 20973866rt^{11} + 1136790t^{12} + 15092r^8t^3 + 911704r^7t^4 + 15910942r^6t^5 + \\
 &\quad 107913884r^5t^6 + 317106478r^4t^7 + 418949958r^3t^8 + 245144867r^2t^9 + 58282811rt^{10} + 4296036t^{11} + \\
 &\quad 3428r^8t^2 + 312972r^7t^3 + 7805102r^6t^4 + 73211456r^5t^5 + 291496218r^4t^6 + 515224702r^3t^7 + 400729520r^2t^8 + \\
 &\quad 126590649rt^9 + 12475590t^{10} + 484r^8t + 74692r^7t^2 + 2821456r^6t^3 + 37868944r^5t^4 + 208559766r^4t^5 + \\
 &\quad 498997944r^3t^6 + 518288724r^2t^7 + 217141005rt^8 + 28367550t^9 + 32r^8 + 11072r^7t + 708772r^6t^2 + \\
 &\quad 14435652r^5t^3 + 113843214r^4t^4 + 376569828r^3t^5 + 528629382r^2t^6 + 295127820rt^7 + 51019974t^8 + 768r^7 + \\
 &\quad 110544r^6t + 3824244r^5t^2 + 45825120r^4t^3 + 217058472r^3t^4 + 420758442r^2t^5 + 316844460rt^6 + \\
 &\quad 72824292t^7 + 8064r^6 + 628992r^5t + 12826620r^4t^2 + 92375316r^3t^3 + 256228218r^2t^4 + 265946328rt^5 + \\
 &\quad 82254042t^6 + 48384r^5 + 2230200r^4t + 27370764r^3t^2 + 115416576r^2t^3 + 171153648rt^4 + 72789678t^5 + \\
 &\quad 181440r^4 + 5044032r^3t + 36268236r^2t^2 + 81676188rt^3 + 49514166t^4 + 435456r^3 + 7103376r^2t + \\
 &\quad 27267516rt^2 + 25051356t^3 + 653184r^2 + 5692032rt + 8899632t^2 + 559872r + 1985796t + 209952)(t+1)t. \\
 D_C^U &= (6s^5t^{10} + 60s^5t^9 + 38s^4t^{10} + 270s^5t^8 + 407s^4t^9 + 96s^3t^{10} + 720s^5t^7 + 1969s^4t^8 + 1093s^3t^9 + 121s^2t^{10} + \\
 &\quad 1260s^5t^6 + 5663s^4t^7 + 5639s^3t^8 + 1450s^2t^9 + 75st^{10} + 1512s^5t^5 + 10717s^4t^6 + 17367s^3t^7 + 7901s^2t^8 + \\
 &\quad 944st^9 + 18t^{10} + 1260s^5t^4 + 13937s^4t^5 + 35357s^3t^6 + 25842s^2t^7 + 5395st^8 + 240t^9 + 720s^5t^3 + 12607s^4t^4 + \\
 &\quad 49699s^3t^5 + 56251s^2t^6 + 18571st^7 + 1434t^8 + 270s^5t^2 + 7829s^4t^3 + 48813s^3t^4 + 85169s^2t^5 + 42861st^6 + \\
 &\quad 5142t^7 + 60s^5t + 3193s^4t^2 + 33049s^3t^3 + 90800s^2t^4 + 69516st^5 + 12422t^6 + 6s^5 + 772s^4t + 14747s^3t^2 + \\
 &\quad 67239s^2t^3 + 80330st^4 + 21349t^5 + 84s^4 + 3912s^3t + 33051s^2t^2 + 65271st^3 + 26610t^4 + 468s^3 + 9720s^2t + \\
 &\quad 35631st^2 + 23796t^3 + 1296s^2 + 11772st + 14580t^2 + 1782s + 5508t + 972)(s+3)(t+1).
 \end{aligned}$$

Local view 11 of 35.

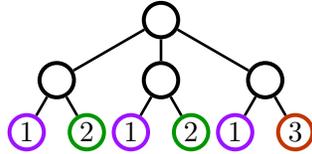

$$\begin{aligned}
 Z_C &= \lambda^6 + 6\lambda^5 + 4\lambda^4(q-3) + 21\lambda^4 + 47\lambda^3(q-3) + 33\lambda^2(q-3)(q-4) + 9\lambda(q-3)(q-4)(q-5) + \\
 &\quad (q-3)(q-4)(q-5)(q-6) + 25\lambda^3 + 66\lambda^2(q-3) + 42\lambda(q-3)(q-4) + 9(q-3)(q-4)(q-5) + 21\lambda^2 + \\
 &\quad 44\lambda(q-3) + 22(q-3)(q-4) + 6\lambda + 14q - 41.
 \end{aligned}$$

$$\begin{aligned}
2Z_C U_C^v &= 3\lambda^6 + 13\lambda^5 + 8\lambda^4(q-3) + 32\lambda^4 + 51\lambda^3(q-3) + 24\lambda^2(q-3)(q-4) + 3\lambda(q-3)(q-4)(q-5) + 21\lambda^3 + \\
&\quad 42\lambda^2(q-3) + 12\lambda(q-3)(q-4) + 11\lambda^2 + 10\lambda(q-3) + \lambda. \\
6Z_C U_C^N &= 6\lambda^6 + 30\lambda^5 + 16\lambda^4(q-3) + 84\lambda^4 + 141\lambda^3(q-3) + 66\lambda^2(q-3)(q-4) + 9\lambda(q-3)(q-4)(q-5) + 75\lambda^3 + \\
&\quad 132\lambda^2(q-3) + 42\lambda(q-3)(q-4) + 42\lambda^2 + 44\lambda(q-3) + 6\lambda. \\
\tilde{S}_C &= (2r^4t^8 + 16r^4t^7 + 12r^3t^8 + 56r^4t^6 + 104r^3t^7 + 28r^2t^8 + 112r^4t^5 + 396r^3t^6 + 260r^2t^7 + 31rt^8 + 140r^4t^4 + \\
&\quad 864r^3t^5 + 1064r^2t^6 + 301rt^7 + 14t^8 + 112r^4t^3 + 1180r^3t^4 + 2504r^2t^5 + 1298rt^6 + 138t^7 + 56r^4t^2 + \\
&\quad 1032r^3t^3 + 3704r^2t^4 + 3246rt^5 + 612t^6 + 16r^4t + 564r^3t^2 + 3524r^2t^3 + 5146rt^4 + 1596t^5 + 2r^4 + 176r^3t + \\
&\quad 2104r^2t^2 + 5292rt^3 + 2676t^4 + 24r^3 + 720r^2t + 3444rt^2 + 2952t^3 + 108r^2 + 1296rt + 2088t^2 + 216r + 864t + \\
&\quad 162)(4r^4t^6 + 24r^4t^5 + 15r^3t^6 + 60r^4t^4 + 120r^3t^5 + 21r^2t^6 + 80r^4t^3 + 378r^3t^4 + 210r^2t^5 + 12rt^6 + 60r^4t^2 + \\
&\quad 612r^3t^3 + 828r^2t^4 + 150rt^5 + 2t^6 + 24r^4t + 543r^3t^2 + 1650r^2t^3 + 741rt^4 + 36t^5 + 4r^4 + 252r^3t + 1767r^2t^2 + \\
&\quad 1836rt^3 + 225t^4 + 48r^3 + 972r^2t + 2421rt^2 + 702t^3 + 216r^2 + 1620rt + 1161t^2 + 432r + 972t + 324)(t+1)^3t. \\
D_C^U &= (6s^5t^8 + 48s^5t^7 + 32s^4t^8 + 168s^5t^6 + 299s^4t^7 + 65s^3t^8 + 336s^5t^5 + 1203s^4t^6 + 708s^3t^7 + 64s^2t^8 + 420s^5t^4 + \\
&\quad 2734s^4t^5 + 3273s^3t^6 + 793s^2t^7 + 31st^8 + 336s^5t^3 + 3850s^4t^4 + 8464s^3t^5 + 4188s^2t^6 + 423st^7 + 6t^8 + 168s^5t^2 + \\
&\quad 3447s^4t^3 + 13479s^3t^4 + 12337s^2t^5 + 2508st^6 + 90t^7 + 48s^5t + 1919s^4t^2 + 13596s^3t^3 + 22309s^2t^4 + 8369st^5 + \\
&\quad 576t^6 + 6s^5 + 608s^4t + 8507s^3t^2 + 25530s^2t^3 + 17218st^4 + 2110t^5 + 84s^4 + 3024s^3t + 18147s^2t^2 + 22512st^3 + \\
&\quad 4872t^4 + 468s^3 + 7344s^2t + 18405st^2 + 7299t^3 + 1296s^2 + 8640st + 6966t^2 + 1782s + 3888t + 972)(s+3)(t+1)^3.
\end{aligned}$$

Local view 12 of 35.

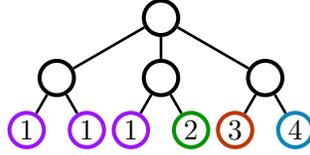

$$\begin{aligned}
Z_C &= 3\lambda^6 + \lambda^5(q-4) + 13\lambda^5 + 16\lambda^4(q-4) + 7\lambda^3(q-4)(q-5) + \lambda^2(q-4)(q-5)(q-6) + 28\lambda^4 + 52\lambda^3(q-4) + \\
&\quad 27\lambda^2(q-4)(q-5) + 7\lambda(q-4)(q-5)(q-6) + (q-4)(q-5)(q-6)(q-7) + 62\lambda^3 + 96\lambda^2(q-4) + \\
&\quad 60\lambda(q-4)(q-5) + 14(q-4)(q-5)(q-6) + 63\lambda^2 + 132\lambda(q-4) + 57(q-4)(q-5) + 69\lambda + 72q - 270. \\
2Z_C U_C^v &= 7\lambda^6 + 2\lambda^5(q-4) + 18\lambda^5 + 14\lambda^4(q-4) + 3\lambda^3(q-4)(q-5) + 36\lambda^4 + 48\lambda^3(q-4) + 18\lambda^2(q-4)(q-5) + \\
&\quad 3\lambda(q-4)(q-5)(q-6) + 62\lambda^3 + 70\lambda^2(q-4) + 24\lambda(q-4)(q-5) + 45\lambda^2 + 49\lambda(q-4) + 24\lambda. \\
6Z_C U_C^N &= 18\lambda^6 + 5\lambda^5(q-4) + 65\lambda^5 + 64\lambda^4(q-4) + 21\lambda^3(q-4)(q-5) + 2\lambda^2(q-4)(q-5)(q-6) + 112\lambda^4 + \\
&\quad 156\lambda^3(q-4) + 54\lambda^2(q-4)(q-5) + 7\lambda(q-4)(q-5)(q-6) + 186\lambda^3 + 192\lambda^2(q-4) + 60\lambda(q-4)(q-5) + \\
&\quad 126\lambda^2 + 132\lambda(q-4) + 69\lambda.
\end{aligned}$$

$$\begin{aligned} \tilde{S}_C &= (16r^8t^{15} + 244r^8t^{14} + 162r^7t^{15} + 1740r^8t^{13} + 2636r^7t^{14} + 722r^6t^{15} + 7696r^8t^{12} + 20038r^7t^{13} + \\ &12492r^6t^{14} + 1855r^5t^{15} + 23608r^8t^{11} + 94384r^7t^{12} + 100890r^6t^{13} + 33977r^5t^{14} + 3013r^4t^{15} + 53196r^8t^{10} + \\ &308024r^7t^{11} + 504556r^6t^{12} + 290433r^5t^{13} + 58106r^4t^{14} + 3178r^3t^{15} + 90948r^8t^9 + 737640r^7t^{10} + \\ &1747296r^6t^{11} + 1537093r^5t^{12} + 523395r^4t^{13} + 64071r^3t^{14} + 2130r^2t^{15} + 120120r^8t^8 + 1338852r^7t^9 + \\ &4437864r^6t^{10} + 5632945r^5t^{11} + 2921010r^4t^{12} + 605057r^3t^{13} + 44502r^2t^{14} + 826rt^{15} + 123552r^8t^7 + \\ &1875216r^7t^8 + 8538732r^6t^9 + 15140187r^5t^{10} + 11295061r^4t^{11} + 3547182r^3t^{12} + 438079r^2t^{13} + 17756rt^{14} + \\ &140t^{15} + 98956r^8t^6 + 2043138r^7t^7 + 12671352r^6t^8 + 30829109r^5t^9 + 32052624r^4t^{10} + 14430020r^3t^{11} + \\ &2687270r^2t^{12} + 181280rt^{13} + 3096t^{14} + 61204r^8t^5 + 1731468r^7t^6 + 14620050r^6t^7 + 48419903r^5t^8 + \\ &68948979r^4t^9 + 43132355r^3t^{10} + 11467674r^2t^{11} + 1159491rt^{12} + 32700t^{13} + 28704r^8t^4 + 1131854r^7t^5 + \\ &13112924r^6t^6 + 59128656r^5t^7 + 114466310r^4t^8 + 97838603r^3t^9 + 36026236r^2t^{10} + 5177882rt^{11} + 217566t^{12} + \\ &9880r^8t^3 + 560416r^7t^4 + 9066690r^6t^5 + 56130224r^5t^6 + 147837930r^4t^7 + 171460688r^3t^8 + 86024723r^2t^9 + \\ &17065506rt^{10} + 1014972t^{11} + 2356r^8t^2 + 203428r^7t^3 + 4745340r^6t^4 + 41074710r^5t^5 + 148510546r^4t^6 + \\ &234009984r^3t^7 + 158932344r^2t^8 + 42835854rt^9 + 3505356t^{10} + 348r^8t + 51104r^7t^2 + 1819612r^6t^3 + \\ &22749912r^5t^4 + 115062546r^4t^5 + 248672040r^3t^6 + 229006584r^2t^7 + 83337705rt^8 + 9240984t^9 + 24r^8 + \\ &7944r^7t + 482544r^6t^2 + 9230220r^5t^3 + 67506948r^4t^4 + 204027858r^3t^5 + 257309676r^2t^6 + 126669798rt^7 + \\ &18917874t^8 + 576r^7 + 79128r^6t + 2589408r^5t^2 + 29025540r^4t^3 + 126899568r^3t^4 + 223571502r^2t^5 + \\ &150407388rt^6 + 30312468t^7 + 6048r^6 + 449064r^5t + 8632440r^4t^2 + 57905820r^3t^3 + 147505860r^2t^4 + \\ &138382506rt^5 + 38018970t^6 + 36288r^5 + 1587600r^4t + 18296928r^3t^2 + 71526564r^2t^3 + 96890904rt^4 + \\ &37032714t^5 + 136080r^4 + 3578904r^3t + 24062832r^2t^2 + 49983156rt^3 + 27524124t^4 + 326592r^3 + 5021352r^2t + \\ &17939232rt^2 + 15119460t^3 + 489888r^2 + 4006584rt + 5799924t^2 + 419904r + 1390932t + 157464)(t+1)^2t. \\ D_C^U &= (6s^5t^9 + 54s^5t^8 + 62s^4t^9 + 216s^5t^7 + 597s^4t^8 + 252s^3t^9 + 504s^5t^6 + 2554s^4t^7 + 2592s^3t^8 + 502s^2t^9 + 756s^5t^5 + \\ &6373s^4t^6 + 11842s^3t^7 + 5502s^2t^8 + 486st^9 + 756s^5t^4 + 10224s^4t^5 + 31569s^3t^6 + 26804s^2t^7 + 5673st^8 + 180t^9 + \\ &504s^5t^3 + 10937s^4t^4 + 54156s^3t^5 + 76288s^2t^6 + 29453st^7 + 2250t^8 + 216s^5t^2 + 7802s^4t^3 + 62030s^3t^4 + \\ &139968s^2t^5 + 89481st^6 + 12471t^7 + 54s^5t + 3579s^4t^2 + 47454s^3t^3 + 171860s^2t^4 + 175686st^5 + 40473t^6 + 6s^5 + \\ &958s^4t + 23385s^3t^2 + 141342s^2t^3 + 231611st^4 + 85122t^5 + 114s^4 + 6736s^3t + 75126s^2t^2 + 205364st^3 + 120732t^4 + \\ &864s^3 + 23424s^2t + 118272st^2 + 115824t^3 + 3264s^2 + 40192st + 72672t^2 + 6144s + 27136t + 4608)(s+4)(t+1)^2. \end{aligned}$$

Local view 13 of 35.

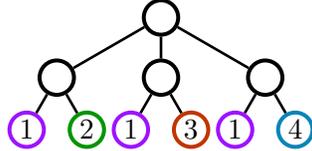

$$\begin{aligned} Z_C &= \lambda^6 + 3\lambda^5 + 3\lambda^4(q-4) + 36\lambda^4 + 51\lambda^3(q-4) + 33\lambda^2(q-4)(q-5) + 9\lambda(q-4)(q-5)(q-6) + \\ &(q-4)(q-5)(q-6)(q-7) + 58\lambda^3 + 126\lambda^2(q-4) + 69\lambda(q-4)(q-5) + 13(q-4)(q-5)(q-6) + 93\lambda^2 + \\ &132\lambda(q-4) + 49(q-4)(q-5) + 51\lambda + 57q - 214. \\ 2Z_C U_C^v &= 3\lambda^6 + 6\lambda^5 + 6\lambda^4(q-4) + 60\lambda^4 + 57\lambda^3(q-4) + 24\lambda^2(q-4)(q-5) + 3\lambda(q-4)(q-5)(q-6) + 54\lambda^3 + \\ &84\lambda^2(q-4) + 21\lambda(q-4)(q-5) + 57\lambda^2 + 36\lambda(q-4) + 12\lambda. \\ 6Z_C U_C^N &= 6\lambda^6 + 15\lambda^5 + 12\lambda^4(q-4) + 144\lambda^4 + 153\lambda^3(q-4) + 66\lambda^2(q-4)(q-5) + 9\lambda(q-4)(q-5)(q-6) + 174\lambda^3 + \\ &252\lambda^2(q-4) + 69\lambda(q-4)(q-5) + 186\lambda^2 + 132\lambda(q-4) + 51\lambda. \\ \tilde{S}_C &= 3(2r^4t^8 + 16r^4t^7 + 12r^3t^8 + 56r^4t^6 + 104r^3t^7 + 28r^2t^8 + 112r^4t^5 + 396r^3t^6 + 260r^2t^7 + 31rt^8 + 140r^4t^4 + \\ &864r^3t^5 + 1064r^2t^6 + 301rt^7 + 14t^8 + 112r^4t^3 + 1180r^3t^4 + 2504r^2t^5 + 1298rt^6 + 138t^7 + 56r^4t^2 + \\ &1032r^3t^3 + 3704r^2t^4 + 3246rt^5 + 612t^6 + 16r^4t + 564r^3t^2 + 3524r^2t^3 + 5146rt^4 + 1596t^5 + 2r^4 + 176r^3t + \\ &2104r^2t^2 + 5292rt^3 + 2676t^4 + 24r^3 + 720r^2t + 3444rt^2 + 2952t^3 + 108r^2 + 1296rt + 2088t^2 + 216r + \\ &864t + 162)(2r^3t^4 + 8r^3t^3 + 7r^2t^4 + 12r^3t^2 + 38r^2t^3 + 9rt^4 + 8r^3t + 73r^2t^2 + 57rt^3 + 4t^4 + 2r^3 + 60r^2t + \\ &138rt^2 + 27t^3 + 18r^2 + 144rt + 81t^2 + 54r + 108t + 54)(rt+r+3)(t+1)^4t. \end{aligned}$$

$$\begin{aligned}
D_C^U &= 3(2s^5t^8 + 16s^5t^7 + 20s^4t^8 + 56s^5t^6 + 175s^4t^7 + 79s^3t^8 + 112s^5t^5 + 667s^4t^6 + 752s^3t^7 + 155s^2t^8 + 140s^5t^4 + \\
&\quad 1448s^4t^5 + 3111s^3t^6 + 1589s^2t^7 + 152st^8 + 112s^5t^3 + 1960s^4t^4 + 7320s^3t^5 + 7095s^2t^6 + 1658st^7 + 60t^8 + \\
&\quad 56s^5t^2 + 1695s^4t^3 + 10733s^3t^4 + 18047s^2t^5 + 7918st^6 + 690t^7 + 16s^5t + 915s^4t^2 + 10056s^3t^3 + 28656s^2t^4 + \\
&\quad 21659st^5 + 3477t^6 + 2s^5 + 282s^4t + 5885s^3t^2 + 29144s^2t^3 + 37179st^4 + 10122t^5 + 38s^4 + 1968s^3t + \\
&\quad 18570s^2t^2 + 41100st^3 + 18684t^4 + 288s^3 + 6784s^2t + 28640st^2 + 22448t^3 + 1088s^2 + 11520st + 17184t^2 + \\
&\quad 2048s + 7680t + 1536)(s+4)(t+1)^3.
\end{aligned}$$

Local view 14 of 35.

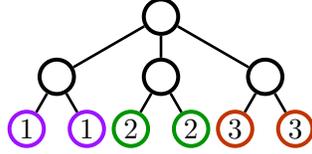

$$\begin{aligned}
Z_C &= 3\lambda^7 + \lambda^6(q-3) + 6\lambda^6 + 9\lambda^5(q-3) + 3\lambda^4(q-3)(q-4) + 9\lambda^5 + 18\lambda^4(q-3) + 9\lambda^3(q-3)(q-4) + \\
&\quad 3\lambda^2(q-3)(q-4)(q-5) + 12\lambda^4 + 28\lambda^3(q-3) + 24\lambda^2(q-3)(q-4) + 3\lambda(q-3)(q-4)(q-5) + \\
&\quad (q-3)(q-4)(q-5)(q-6) + 15\lambda^3 + 45\lambda^2(q-3) + 21\lambda(q-3)(q-4) + 12(q-3)(q-4)(q-5) + 18\lambda^2 + \\
&\quad 36\lambda(q-3) + 40(q-3)(q-4) + 12\lambda + 38q - 108. \\
2Z_C U_C^v &= 3\lambda^7 + 12\lambda^6 + 9\lambda^5(q-3) + 15\lambda^5 + 18\lambda^4(q-3) + 9\lambda^3(q-3)(q-4) + 12\lambda^4 + 30\lambda^3(q-3) + 6\lambda^2(q-3)(q-4) + \\
&\quad 3\lambda(q-3)(q-4)(q-5) + 15\lambda^3 + 18\lambda^2(q-3) + 21\lambda(q-3)(q-4) + 12\lambda^2 + 36\lambda(q-3) + 12\lambda. \\
6Z_C U_C^N &= 21\lambda^7 + 6\lambda^6(q-3) + 36\lambda^6 + 45\lambda^5(q-3) + 12\lambda^4(q-3)(q-4) + 45\lambda^5 + 72\lambda^4(q-3) + 27\lambda^3(q-3)(q-4) + \\
&\quad 6\lambda^2(q-3)(q-4)(q-5) + 48\lambda^4 + 84\lambda^3(q-3) + 48\lambda^2(q-3)(q-4) + 3\lambda(q-3)(q-4)(q-5) + 45\lambda^3 + \\
&\quad 90\lambda^2(q-3) + 21\lambda(q-3)(q-4) + 36\lambda^2 + 36\lambda(q-3) + 12\lambda. \\
\tilde{S}_C &= 6(r^4t^7 + 8r^4t^6 + 4r^3t^7 + 27r^4t^5 + 40r^3t^6 + 6r^2t^7 + 50r^4t^4 + 164r^3t^5 + 76r^2t^6 + 5rt^7 + 55r^4t^3 + 360r^3t^4 + \\
&\quad 370r^2t^5 + 68rt^6 + 2t^7 + 36r^4t^2 + 460r^3t^3 + 948r^2t^4 + 373rt^5 + 24t^6 + 13r^4t + 344r^3t^2 + 1402r^2t^3 + \\
&\quad 1090rt^4 + 141t^5 + 2r^4 + 140r^3t + 1204r^2t^2 + 1848rt^3 + 462t^4 + 24r^3 + 558r^2t + 1824rt^2 + 891t^3 + 108r^2 + \\
&\quad 972rt + 1008t^2 + 216r + 621t + 162)(2r^3t^6 + 12r^3t^5 + 11r^2t^6 + 30r^3t^4 + 69r^2t^5 + 21rt^6 + 40r^3t^3 + \\
&\quad 183r^2t^4 + 136rt^5 + 14t^6 + 30r^3t^2 + 263r^2t^3 + 376rt^4 + 92t^5 + 12r^3t + 216r^2t^2 + 573rt^3 + 260t^4 + 2r^3 + \\
&\quad 96r^2t + 510rt^2 + 414t^3 + 18r^2 + 252rt + 396t^2 + 54r + 216t + 54)(rt^2 + 2rt + t^2 + r + 3t + 3)(t+2)(t+1)t. \\
D_C^U &= 3(2s^4t^8 + 16s^4t^7 + 12s^3t^8 + 56s^4t^6 + 99s^3t^7 + 28s^2t^8 + 112s^4t^5 + 363s^3t^6 + 233s^2t^7 + 30st^8 + 140s^4t^4 + 772s^3t^5 + \\
&\quad 874s^2t^6 + 246st^7 + 12t^8 + 112s^4t^3 + 1040s^3t^4 + 1936s^2t^5 + 918st^6 + 96t^7 + 56s^4t^2 + 907s^3t^3 + 2772s^2t^4 + \\
&\quad 2063st^5 + 348t^6 + 16s^4t + 499s^3t^2 + 2623s^2t^3 + 3082st^4 + 766t^5 + 2s^4 + 158s^3t + 1596s^2t^2 + 3144st^3 + 1156t^4 + \\
&\quad 22s^3 + 568s^2t + 2131st^2 + 1258t^3 + 90s^2 + 870st + 966t^2 + 162s + 468t + 108)(st^2 + 2st + t^2 + s + 3t + 3)(s+3)(t+1).
\end{aligned}$$

Local view 15 of 35.

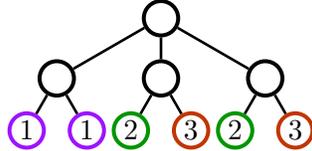

$$\begin{aligned}
Z_C &= 2\lambda^6 + 15\lambda^5 + 21\lambda^4(q-3) + 7\lambda^3(q-3)(q-4) + \lambda^2(q-3)(q-4)(q-5) + 12\lambda^4 + 28\lambda^3(q-3) + \\
&\quad 24\lambda^2(q-3)(q-4) + 7\lambda(q-3)(q-4)(q-5) + (q-3)(q-4)(q-5)(q-6) + 14\lambda^3 + 58\lambda^2(q-3) + \\
&\quad 39\lambda(q-3)(q-4) + 10(q-3)(q-4)(q-5) + 30\lambda^2 + 49\lambda(q-3) + 27(q-3)(q-4) + 6\lambda + 19q - 55. \\
2Z_C U_C^v &= 4\lambda^6 + 25\lambda^5 + 22\lambda^4(q-3) + 3\lambda^3(q-3)(q-4) + 16\lambda^4 + 30\lambda^3(q-3) + 18\lambda^2(q-3)(q-4) + \\
&\quad 3\lambda(q-3)(q-4)(q-5) + 14\lambda^3 + 42\lambda^2(q-3) + 15\lambda(q-3)(q-4) + 20\lambda^2 + 17\lambda(q-3) + 2\lambda. \\
6Z_C U_C^N &= 12\lambda^6 + 75\lambda^5 + 84\lambda^4(q-3) + 21\lambda^3(q-3)(q-4) + 2\lambda^2(q-3)(q-4)(q-5) + 48\lambda^4 + 84\lambda^3(q-3) + \\
&\quad 48\lambda^2(q-3)(q-4) + 7\lambda(q-3)(q-4)(q-5) + 42\lambda^3 + 116\lambda^2(q-3) + 39\lambda(q-3)(q-4) + 60\lambda^2 + \\
&\quad 49\lambda(q-3) + 6\lambda.
\end{aligned}$$

$$\begin{aligned} \tilde{S}_C &= 2(6r^8t^{15} + 94r^8t^{14} + 59r^7t^{15} + 688r^8t^{13} + 988r^7t^{14} + 252r^6t^{15} + 3120r^8t^{12} + 7727r^7t^{13} + 4514r^6t^{14} + 610r^5t^{15} + \\ & 9802r^8t^{11} + 37420r^7t^{12} + 37702r^6t^{13} + 11702r^5t^{14} + 911r^4t^{15} + 22594r^8t^{10} + 125434r^7t^{11} + 194742r^6t^{12} + \\ & 104357r^5t^{13} + 18780r^4t^{14} + 852r^3t^{15} + 39468r^8t^9 + 308166r^7t^{10} + 695544r^6t^{11} + 574402r^5t^{12} + 179005r^4t^{13} + \\ & 19014r^3t^{14} + 480r^2t^{15} + 53196r^8t^8 + 573066r^7t^9 + 1819074r^6t^{10} + 2183288r^5t^{11} + 1049694r^4t^{12} + \\ & 194327r^3t^{13} + 11760r^2t^{14} + 144rt^{15} + 55770r^8t^7 + 821184r^7t^8 + 3597912r^6t^9 + 6071290r^5t^{10} + 4242621r^4t^{11} + \\ & 1215280r^3t^{12} + 129735r^2t^{13} + 3996rt^{14} + 16t^{15} + 45474r^8t^6 + 914055r^7t^7 + 5478900r^6t^8 + 12759962r^5t^9 + \\ & 12531878r^4t^{10} + 5222615r^3t^{11} + 867936r^2t^{12} + 48258rt^{13} + 552t^{14} + 28600r^8t^5 + 790208r^7t^6 + 6475188r^6t^7 + \\ & 20636932r^5t^8 + 27961299r^4t^9 + 16376750r^3t^{10} + 3970620r^2t^{11} + 347760rt^{12} + 7536t^{13} + 13624r^8t^4 + \\ & 526195r^7t^5 + 5938254r^6t^6 + 25892270r^5t^7 + 47997990r^4t^8 + 38764066r^3t^9 + 13220244r^2t^{10} + 1699353rt^{11} + \\ & 59328t^{12} + 4758r^8t^3 + 265028r^7t^4 + 4190846r^6t^5 + 25197866r^5t^6 + 63913684r^4t^7 + 70582724r^3t^8 + \\ & 33187851r^2t^9 + 6016896rt^{10} + 311850t^{11} + 1150r^8t^2 + 97732r^7t^3 + 2234998r^6t^4 + 18863029r^5t^5 + \\ & 66016256r^4t^6 + 99716067r^3t^7 + 64072452r^2t^8 + 16027956rt^9 + 1178496t^{10} + 172r^8t + 24910r^7t^2 + \\ & 871848r^6t^3 + 10665930r^5t^4 + 52456332r^4t^5 + 109320894r^3t^6 + 96005988r^2t^7 + 32809878rt^8 + 3337308t^9 + \\ & 12r^8 + 3924r^7t + 234846r^6t^2 + 4409280r^5t^3 + 31486464r^4t^4 + 92251521r^3t^5 + 111712392r^2t^6 + 52135812rt^7 + \\ & 7249500t^8 + 288r^7 + 39060r^6t + 1258038r^5t^2 + 13818600r^4t^3 + 58843800r^3t^4 + 100151586r^2t^5 + \\ & 64386144rt^6 + 12219822t^7 + 3024r^6 + 221508r^5t + 4185810r^4t^2 + 27462564r^3t^3 + 67948470r^2t^4 + \\ & 61341543rt^5 + 16018560t^6 + 18144r^5 + 782460r^4t + 8852490r^3t^2 + 33775056r^2t^3 + 44299386rt^4 + \\ & 16221708t^5 + 68040r^4 + 1762236r^3t + 11612970r^2t^2 + 23485464rt^3 + 12477564t^4 + 163296r^3 + 2469852r^2t + \\ & 8632818rt^2 + 7064010t^3 + 244944r^2 + 1968300rt + 2781864t^2 + 209952r + 682344t + 78732)(t + 1)^2t. \\ D_C^U &= (6s^5t^9 + 54s^5t^8 + 34s^4t^9 + 216s^5t^7 + 341s^4t^8 + 76s^3t^9 + 504s^5t^6 + 1516s^4t^7 + 840s^3t^8 + 86s^2t^9 + 756s^5t^5 + \\ & 3923s^4t^6 + 4110s^3t^7 + 1018s^2t^8 + 50st^9 + 756s^5t^4 + 6514s^4t^5 + 11717s^3t^6 + 5378s^2t^7 + 618st^8 + 12t^9 + \\ & 504s^5t^3 + 7199s^4t^4 + 21480s^3t^5 + 16691s^2t^6 + 3432st^7 + 156t^8 + 216s^5t^2 + 5296s^4t^3 + 26274s^3t^4 + \\ & 33592s^2t^5 + 11326st^6 + 888t^7 + 54s^5t + 2501s^4t^2 + 21442s^3t^3 + 45482s^2t^4 + 24652st^5 + 2984t^6 + 6s^5 + \\ & 688s^4t + 11253s^3t^2 + 41400s^2t^3 + 36785st^4 + 6744t^5 + 84s^4 + 3444s^3t + 24393s^2t^2 + 37542st^3 + 10860t^4 + \\ & 468s^3 + 8424s^2t + 25155st^2 + 12456t^3 + 1296s^2 + 9990st + 9666t^2 + 1782s + 4536t + 972)(s + 3)(t + 1)^2. \end{aligned}$$

Local view 16 of 35.

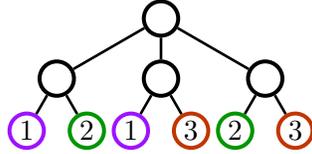

$$\begin{aligned} Z_C &= 9\lambda^5 + 3\lambda^4(q - 3) + 18\lambda^4 + 51\lambda^3(q - 3) + 33\lambda^2(q - 3)(q - 4) + 9\lambda(q - 3)(q - 4)(q - 5) + \\ & (q - 3)(q - 4)(q - 5)(q - 6) + 27\lambda^3 + 60\lambda^2(q - 3) + 42\lambda(q - 3)(q - 4) + 9(q - 3)(q - 4)(q - 5) + 18\lambda^2 + \\ & 48\lambda(q - 3) + 22(q - 3)(q - 4) + 9\lambda + 13q - 39. \\ 2Z_C U_C^v &= 21\lambda^5 + 6\lambda^4(q - 3) + 24\lambda^4 + 57\lambda^3(q - 3) + 24\lambda^2(q - 3)(q - 4) + 3\lambda(q - 3)(q - 4)(q - 5) + 27\lambda^3 + \\ & 36\lambda^2(q - 3) + 12\lambda(q - 3)(q - 4) + 6\lambda^2 + 12\lambda(q - 3) + 3\lambda. \\ 6Z_C U_C^N &= 45\lambda^5 + 12\lambda^4(q - 3) + 72\lambda^4 + 153\lambda^3(q - 3) + 66\lambda^2(q - 3)(q - 4) + 9\lambda(q - 3)(q - 4)(q - 5) + 81\lambda^3 + \\ & 120\lambda^2(q - 3) + 42\lambda(q - 3)(q - 4) + 36\lambda^2 + 48\lambda(q - 3) + 9\lambda. \\ \tilde{S}_C &= 6(2r^4t^8 + 16r^4t^7 + 12r^3t^8 + 56r^4t^6 + 104r^3t^7 + 28r^2t^8 + 112r^4t^5 + 396r^3t^6 + 260r^2t^7 + 31rt^8 + 140r^4t^4 + \\ & 864r^3t^5 + 1064r^2t^6 + 301rt^7 + 14t^8 + 112r^4t^3 + 1180r^3t^4 + 2504r^2t^5 + 1298rt^6 + 138t^7 + 56r^4t^2 + \\ & 1032r^3t^3 + 3704r^2t^4 + 3246rt^5 + 612t^6 + 16r^4t + 564r^3t^2 + 3524r^2t^3 + 5146rt^4 + 1596t^5 + 2r^4 + 176r^3t + \\ & 2104r^2t^2 + 5292rt^3 + 2676t^4 + 24r^3 + 720r^2t + 3444rt^2 + 2952t^3 + 108r^2 + 1296rt + 2088t^2 + 216r + \\ & 864t + 162)(r^3t^4 + 4r^3t^3 + 3r^2t^4 + 6r^3t^2 + 18r^2t^3 + 3rt^4 + 4r^3t + 36r^2t^2 + 24rt^3 + t^4 + r^3 + 30r^2t + \\ & 66rt^2 + 9t^3 + 9r^2 + 72rt + 36t^2 + 27r + 54t + 27)(rt^2 + 2rt + t^2 + r + 3t + 3)(t + 1)^3t. \end{aligned}$$

$$D_C^U = 3(2s^5t^8 + 16s^5t^7 + 10s^4t^8 + 56s^5t^6 + 95s^4t^7 + 18s^3t^8 + 112s^5t^5 + 387s^4t^6 + 207s^3t^7 + 14s^2t^8 + 140s^5t^4 + 888s^4t^5 + 993s^3t^6 + 198s^2t^7 + 4st^8 + 112s^5t^3 + 1260s^4t^4 + 2638s^3t^5 + 1144s^2t^6 + 75st^7 + 56s^5t^2 + 1135s^4t^3 + 4288s^3t^4 + 3585s^2t^5 + 555st^6 + 6t^7 + 16s^5t + 635s^4t^2 + 4395s^3t^3 + 6777s^2t^4 + 2133st^5 + 78t^6 + 2s^5 + 202s^4t + 2785s^3t^2 + 8017s^2t^3 + 4821st^4 + 406t^5 + 28s^4 + 1000s^3t + 5845s^2t^2 + 6733st^3 + 1158t^4 + 156s^3 + 2412s^2t + 5775st^2 + 1992t^3 + 432s^2 + 2808st + 2088t^2 + 594s + 1242t + 324)(s+3)(t+1)^3.$$

Local view 17 of 35.

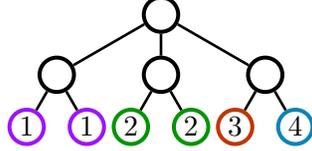

$$Z_C = 8\lambda^6 + 5\lambda^5(q-4) + \lambda^4(q-4)(q-5) + 14\lambda^5 + 22\lambda^4(q-4) + 10\lambda^3(q-4)(q-5) + 2\lambda^2(q-4)(q-5)(q-6) + 32\lambda^4 + 51\lambda^3(q-4) + 27\lambda^2(q-4)(q-5) + 5\lambda(q-4)(q-5)(q-6) + (q-4)(q-5)(q-6)(q-7) + 48\lambda^3 + 84\lambda^2(q-4) + 47\lambda(q-4)(q-5) + 15(q-4)(q-5)(q-6) + 60\lambda^2 + 115\lambda(q-4) + 66(q-4)(q-5) + 66\lambda + 92q - 340.$$

$$2Z_C U_C^v = 10\lambda^6 + 3\lambda^5(q-4) + 24\lambda^5 + 24\lambda^4(q-4) + 6\lambda^3(q-4)(q-5) + 38\lambda^4 + 39\lambda^3(q-4) + 12\lambda^2(q-4)(q-5) + 3\lambda(q-4)(q-5)(q-6) + 38\lambda^3 + 54\lambda^2(q-4) + 27\lambda(q-4)(q-5) + 48\lambda^2 + 63\lambda(q-4) + 34\lambda.$$

$$6Z_C U_C^N = 48\lambda^6 + 25\lambda^5(q-4) + 4\lambda^4(q-4)(q-5) + 70\lambda^5 + 88\lambda^4(q-4) + 30\lambda^3(q-4)(q-5) + 4\lambda^2(q-4)(q-5)(q-6) + 128\lambda^4 + 153\lambda^3(q-4) + 54\lambda^2(q-4)(q-5) + 5\lambda(q-4)(q-5)(q-6) + 144\lambda^3 + 168\lambda^2(q-4) + 47\lambda(q-4)(q-5) + 120\lambda^2 + 115\lambda(q-4) + 66\lambda.$$

$$\begin{aligned} \tilde{S}_C = & 2(8r^8t^{15} + 128r^8t^{14} + 82r^7t^{15} + 956r^8t^{13} + 1392r^7t^{14} + 368r^6t^{15} + 4420r^8t^{12} + 11038r^7t^{13} + 6624r^6t^{14} + \\ & 948r^5t^{15} + 14144r^8t^{11} + 54196r^7t^{12} + 55680r^6t^{13} + 18056r^5t^{14} + 1541r^4t^{15} + 33176r^8t^{10} + 184156r^7t^{11} + \\ & 289740r^6t^{12} + 160506r^5t^{13} + 30924r^4t^{14} + 1629r^3t^{15} + 58916r^8t^9 + 458504r^7t^{10} + 1043222r^6t^{11} + \\ & 883024r^5t^{12} + 289661r^4t^{13} + 34186r^3t^{14} + 1099r^2t^{15} + 80652r^8t^8 + 863784r^7t^9 + 2751704r^6t^{10} + \\ & 3361112r^5t^{11} + 1679622r^4t^{12} + 335637r^3t^{13} + 23874r^2t^{14} + 431rt^{15} + 85800r^8t^7 + 1253496r^7t^8 + \\ & 5490868r^6t^9 + 9373024r^5t^{10} + 6741057r^4t^{11} + 2043386r^3t^{12} + 244030r^2t^{13} + 9612rt^{14} + 74t^{15} + 70928r^8t^6 + \\ & 1412442r^7t^7 + 8437832r^6t^8 + 19776896r^5t^9 + 19830664r^4t^{10} + 8621729r^3t^{11} + 1552812r^2t^{12} + 101652rt^{13} + \\ & 1696t^{14} + 45188r^8t^5 + 1235632r^7t^6 + 10065316r^6t^7 + 32142232r^5t^8 + 44164209r^4t^9 + 26693890r^3t^{10} + \\ & 6866402r^2t^{11} + 673120rt^{12} + 18504t^{13} + 21788r^8t^4 + 832302r^7t^5 + 9318640r^6t^6 + 40560068r^5t^7 + \\ & 75808326r^4t^8 + 62632709r^3t^9 + 22323598r^2t^{10} + 3110230rt^{11} + 127104t^{12} + 7696r^8t^3 + 423892r^7t^4 + \\ & 6640336r^6t^5 + 39732640r^5t^6 + 101104052r^4t^7 + 113385106r^3t^8 + 55087475r^2t^9 + 10596752rt^{10} + \\ & 612252t^{11} + 1880r^8t^2 + 158008r^7t^3 + 3576284r^6t^4 + 29963866r^5t^5 + 104753312r^4t^6 + 159659830r^3t^7 + \\ & 105032966r^2t^8 + 27461787rt^9 + 2182776t^{10} + 284r^8t + 40696r^7t^2 + 1409062r^6t^3 + 17081560r^5t^4 + \\ & 83618838r^4t^5 + 174864732r^3t^6 + 155994678r^2t^7 + 55084350rt^8 + 5934978t^9 + 20r^8 + 6476r^7t + \\ & 383416r^6t^2 + 7124736r^5t^3 + 50496480r^4t^4 + 147743910r^3t^5 + 180484740r^2t^6 + 86211756rt^7 + 12515220t^8 + \\ & 480r^7 + 64428r^6t + 2052504r^5t^2 + 22328910r^4t^3 + 94568004r^3t^4 + 161373168r^2t^5 + 105302484rt^6 + \\ & 20628378t^7 + 5040r^6 + 365148r^5t + 6824520r^4t^2 + 44388648r^3t^3 + 109522476r^2t^4 + 99604242rt^5 + \\ & 26585820t^6 + 30240r^5 + 1288980r^4t + 14423400r^3t^2 + 54629154r^2t^3 + 71690832rt^4 + 26594406t^5 + \\ & 113400r^4 + 2900772r^3t + 18909288r^2t^2 + 38032416rt^3 + 20300220t^4 + 272160r^3 + 4061988r^2t + \\ & 14049288rt^2 + 11461338t^3 + 408240r^2 + 3233844rt + 4525632t^2 + 349920r + 1119744t + 131220)(t+1)^2t. \end{aligned}$$

$$D_C^U = (6s^5t^9 + 54s^5t^8 + 66s^4t^9 + 216s^5t^7 + 621s^4t^8 + 290s^3t^9 + 504s^5t^6 + 2610s^4t^7 + 2839s^3t^8 + 636s^2t^9 + 756s^5t^5 + 6429s^4t^6 + 12474s^3t^7 + 6444s^2t^8 + 694st^9 + 756s^5t^4 + 10224s^4t^5 + 32293s^3t^6 + 29436s^2t^7 + 7250st^8 + 300t^9 + 504s^5t^3 + 10881s^4t^4 + 54278s^3t^5 + 79695s^2t^6 + 34248st^7 + 3228t^8 + 216s^5t^2 + 7746s^4t^3 + 61401s^3t^4 + 141060s^2t^5 + 96427st^6 + 15696t^7 + 54s^5t + 3555s^4t^2 + 46718s^3t^3 + 169317s^2t^4 + 178904st^5 + 45660t^6 + 6s^5 + 954s^4t + 23035s^3t^2 + 137778s^2t^3 + 227277st^4 + 88242t^5 + 114s^4 + 6672s^3t + 73230s^2t^2 + 197844st^3 + 118164t^4 + 864s^3 + 23040s^2t + 113760st^2 + 110000t^3 + 3264s^2 + 39168st + 68704t^2 + 6144s + 26112t + 4608)(s+4)(t+1)^2.$$

Local view 18 of 35.

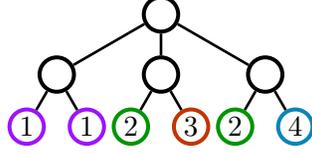

$$Z_C = \lambda^6 + 18\lambda^5 + 20\lambda^4(q-4) + 7\lambda^3(q-4)(q-5) + \lambda^2(q-4)(q-5)(q-6) + 29\lambda^4 + 46\lambda^3(q-4) + 27\lambda^2(q-4)(q-5) + 7\lambda(q-4)(q-5)(q-6) + (q-4)(q-5)(q-6)(q-7) + 48\lambda^3 + 100\lambda^2(q-4) + 60\lambda(q-4)(q-5) + 14(q-4)(q-5)(q-6) + 79\lambda^2 + 131\lambda(q-4) + 57(q-4)(q-5) + 62\lambda + 72q - 269.$$

$$2Z_C U_C^v = 2\lambda^6 + 28\lambda^5 + 20\lambda^4(q-4) + 3\lambda^3(q-4)(q-5) + 38\lambda^4 + 42\lambda^3(q-4) + 18\lambda^2(q-4)(q-5) + 3\lambda(q-4)(q-5)(q-6) + 46\lambda^3 + 72\lambda^2(q-4) + 24\lambda(q-4)(q-5) + 56\lambda^2 + 49\lambda(q-4) + 22\lambda.$$

$$6Z_C U_C^N = 6\lambda^6 + 90\lambda^5 + 80\lambda^4(q-4) + 21\lambda^3(q-4)(q-5) + 2\lambda^2(q-4)(q-5)(q-6) + 116\lambda^4 + 138\lambda^3(q-4) + 54\lambda^2(q-4)(q-5) + 7\lambda(q-4)(q-5)(q-6) + 144\lambda^3 + 200\lambda^2(q-4) + 60\lambda(q-4)(q-5) + 158\lambda^2 + 131\lambda(q-4) + 62\lambda.$$

$$\begin{aligned} \tilde{S}_C = & 2(8r^8t^{15} + 124r^8t^{14} + 79r^7t^{15} + 898r^8t^{13} + 1310r^7t^{14} + 341r^6t^{15} + 4030r^8t^{12} + 10141r^7t^{13} + 6040r^6t^{14} + \\ & 841r^5t^{15} + 12532r^8t^{11} + 48600r^7t^{12} + 49878r^6t^{13} + 15880r^5t^{14} + 1295r^4t^{15} + 28600r^8t^{10} + 161210r^7t^{11} + \\ & 254718r^6t^{12} + 139589r^5t^{13} + 26021r^4t^{14} + 1272r^3t^{15} + 49478r^8t^9 + 391964r^7t^{10} + 899515r^6t^{11} + 758024r^5t^{12} + \\ & 243019r^4t^{13} + 27157r^3t^{14} + 774r^2t^{15} + 66066r^8t^8 + 721500r^7t^9 + 2326416r^6t^{10} + 2844442r^5t^{11} + \\ & 1400713r^4t^{12} + 269106r^3t^{13} + 17548r^2t^{14} + 262rt^{15} + 68640r^8t^7 + 1023672r^7t^8 + 4551414r^6t^9 + 7812872r^5t^{10} + \\ & 5575465r^4t^{11} + 1644121r^3t^{12} + 184466r^2t^{13} + 6350rt^{14} + 36t^{15} + 55484r^8t^6 + 1128555r^7t^7 + 6857772r^6t^8 + \\ & 16226476r^5t^9 + 16239803r^4t^{10} + 6933022r^3t^{11} + 1194327r^2t^{12} + 71075rt^{13} + 964t^{14} + 34606r^8t^5 + 966670r^7t^6 + \\ & 8022195r^6t^7 + 25945424r^5t^8 + 35763164r^4t^9 + 21388831r^3t^{10} + 5333160r^2t^{11} + 488713rt^{12} + 11646t^{13} + \\ & 16354r^8t^4 + 638021r^7t^5 + 7284896r^6t^6 + 32197645r^5t^7 + 60635369r^4t^8 + 49892797r^3t^9 + 17416598r^2t^{10} + \\ & 2313698rt^{11} + 85614t^{12} + 5668r^8t^3 + 318640r^7t^4 + 5092978r^6t^5 + 31006824r^5t^6 + 79797163r^4t^7 + \\ & 89629023r^3t^8 + 43006542r^2t^9 + 8002700rt^{10} + 431364t^{11} + 1360r^8t^2 + 116556r^7t^3 + 2691774r^6t^4 + \\ & 22979909r^5t^5 + 81504000r^4t^6 + 125033068r^3t^7 + 81812339r^2t^8 + 20920710rt^9 + 1583880t^{10} + 202r^8t + \\ & 29480r^7t^2 + 1041069r^6t^3 + 12870136r^5t^4 + 64075503r^4t^5 + 135448356r^3t^6 + 120933135r^2t^7 + 42138435rt^8 + \\ & 4389372t^9 + 14r^8 + 4610r^7t + 278152r^6t^2 + 5272320r^5t^3 + 38072178r^4t^4 + 113010813r^3t^5 + 138938274r^2t^6 + \\ & 65990052rt^7 + 9367074t^8 + 336r^7 + 45906r^6t + 1491336r^5t^2 + 16548345r^4t^3 + 71312688r^3t^4 + 123070806r^2t^5 + \\ & 80401734rt^6 + 15544899t^7 + 3528r^6 + 260442r^5t + 4966920r^4t^2 + 32942484r^3t^3 + 82549962r^2t^4 + \\ & 75631401rt^5 + 20088162t^6 + 21168r^5 + 920430r^4t + 10515960r^3t^2 + 40589343r^2t^3 + 53963496rt^4 + \\ & 20072043t^5 + 79380r^4 + 2074086r^3t + 13812120r^2t^2 + 28281312rt^3 + 15243876t^4 + 190512r^3 + 2908710r^2t + \\ & 10281816rt^2 + 8525655t^3 + 285768r^2 + 2319678rt + 3318408t^2 + 244944r + 804816t + 91854)(t+1)^2t. \end{aligned}$$

$$\begin{aligned} D_C^U = & (6s^5t^9 + 54s^5t^8 + 62s^4t^9 + 216s^5t^7 + 595s^4t^8 + 254s^3t^9 + 504s^5t^6 + 2540s^4t^7 + 2588s^3t^8 + 517s^2t^9 + 756s^5t^5 + \\ & 6331s^4t^6 + 11744s^3t^7 + 5555s^2t^8 + 523st^9 + 756s^5t^4 + 10154s^4t^5 + 31177s^3t^6 + 26650s^2t^7 + 5887st^8 + 210t^9 + \\ & 504s^5t^3 + 10867s^4t^4 + 53386s^3t^5 + 75058s^2t^6 + 29662st^7 + 2469t^8 + 216s^5t^2 + 7760s^4t^3 + 61162s^3t^4 + \\ & 136931s^2t^5 + 88138st^6 + 12972t^7 + 54s^5t + 3565s^4t^2 + 46880s^3t^3 + 167917s^2t^4 + 170707st^5 + 40332t^6 + 6s^5 + \\ & 956s^4t + 23177s^3t^2 + 138438s^2t^3 + 223879st^4 + 82398t^5 + 114s^4 + 6704s^3t + 73974s^2t^2 + 198932st^3 + 115260t^4 + \\ & 864s^3 + 23232s^2t + 115456st^2 + 110576t^3 + 3264s^2 + 39680st + 70112t^2 + 6144s + 26624t + 4608)(s+4)(t+1)^2. \end{aligned}$$

Local view 19 of 35.

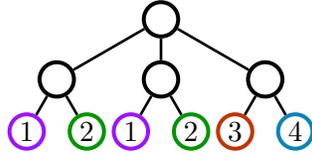

$$Z_C = 6\lambda^5 + 2\lambda^4(q-4) + 32\lambda^4 + 55\lambda^3(q-4) + 33\lambda^2(q-4)(q-5) + 9\lambda(q-4)(q-5)(q-6) + (q-4)(q-5)(q-6)(q-7) + 64\lambda^3 + 120\lambda^2(q-4) + 69\lambda(q-4)(q-5) + 13(q-4)(q-5)(q-6) + 84\lambda^2 + 136\lambda(q-4) + 49(q-4)(q-5) + 58\lambda + 56q - 212.$$

$$\begin{aligned}
2Z_C U_C^v &= 14\lambda^5 + 4\lambda^4(q-4) + 50\lambda^4 + 63\lambda^3(q-4) + 24\lambda^2(q-4)(q-5) + 3\lambda(q-4)(q-5)(q-6) + 66\lambda^3 + \\
&\quad 78\lambda^2(q-4) + 21\lambda(q-4)(q-5) + 46\lambda^2 + 38\lambda(q-4) + 16\lambda. \\
6Z_C U_C^N &= 30\lambda^5 + 8\lambda^4(q-4) + 128\lambda^4 + 165\lambda^3(q-4) + 66\lambda^2(q-4)(q-5) + 9\lambda(q-4)(q-5)(q-6) + 192\lambda^3 + \\
&\quad 240\lambda^2(q-4) + 69\lambda(q-4)(q-5) + 168\lambda^2 + 136\lambda(q-4) + 58\lambda. \\
\tilde{S}_C &= 2(2r^4t^8 + 16r^4t^7 + 12r^3t^8 + 56r^4t^6 + 104r^3t^7 + 28r^2t^8 + 112r^4t^5 + 396r^3t^6 + 260r^2t^7 + 31rt^8 + 140r^4t^4 + \\
&\quad 864r^3t^5 + 1064r^2t^6 + 301rt^7 + 14t^8 + 112r^4t^3 + 1180r^3t^4 + 2504r^2t^5 + 1298rt^6 + 138t^7 + 56r^4t^2 + \\
&\quad 1032r^3t^3 + 3704r^2t^4 + 3246rt^5 + 612t^6 + 16r^4t + 564r^3t^2 + 3524r^2t^3 + 5146rt^4 + 1596t^5 + 2r^4 + 176r^3t + \\
&\quad 2104r^2t^2 + 5292rt^3 + 2676t^4 + 24r^3 + 720r^2t + 3444rt^2 + 2952t^3 + 108r^2 + 1296rt + 2088t^2 + 216r + 864t + \\
&\quad 162)(4r^4t^6 + 24r^4t^5 + 15r^3t^6 + 60r^4t^4 + 120r^3t^5 + 21r^2t^6 + 80r^4t^3 + 378r^3t^4 + 210r^2t^5 + 12rt^6 + 60r^4t^2 + \\
&\quad 612r^3t^3 + 828r^2t^4 + 150rt^5 + 2t^6 + 24r^4t + 543r^3t^2 + 1650r^2t^3 + 741rt^4 + 36t^5 + 4r^4 + 252r^3t + 1767r^2t^2 + \\
&\quad 1836rt^3 + 225t^4 + 48r^3 + 972r^2t + 2421rt^2 + 702t^3 + 216r^2 + 1620rt + 1161t^2 + 432r + 972t + 324)(t+1)^3t. \\
D_C^U &= (6s^5t^8 + 48s^5t^7 + 58s^4t^8 + 168s^5t^6 + 511s^4t^7 + 218s^3t^8 + 336s^5t^5 + 1959s^4t^6 + 2113s^3t^7 + 398s^2t^8 + \\
&\quad 420s^5t^4 + 4274s^4t^5 + 8871s^3t^6 + 4223s^2t^7 + 352s^8 + 336s^5t^3 + 5810s^4t^4 + 21130s^3t^5 + 19395s^2t^6 + \\
&\quad 4061st^7 + 120t^8 + 168s^5t^2 + 5043s^4t^3 + 31304s^3t^4 + 50489s^2t^5 + 20349st^6 + 1500t^7 + 48s^5t + 2731s^4t^2 + \\
&\quad 29589s^3t^3 + 81725s^2t^4 + 57913st^5 + 8154t^6 + 6s^5 + 844s^4t + 17447s^3t^2 + 84468s^2t^3 + 102701st^4 + \\
&\quad 25302t^5 + 114s^4 + 5872s^3t + 54558s^2t^2 + 116628st^3 + 49236t^4 + 864s^3 + 20160s^2t + 83104st^2 + 61776t^3 + \\
&\quad 3264s^2 + 34048st + 48992t^2 + 6144s + 22528t + 4608)(s+4)(t+1)^3.
\end{aligned}$$

Local view 20 of 35.

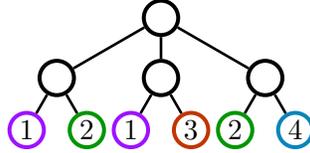

$$\begin{aligned}
Z_C &= 6\lambda^5 + 2\lambda^4(q-4) + 32\lambda^4 + 55\lambda^3(q-4) + 33\lambda^2(q-4)(q-5) + 9\lambda(q-4)(q-5)(q-6) + \\
&\quad (q-4)(q-5)(q-6)(q-7) + 64\lambda^3 + 120\lambda^2(q-4) + 69\lambda(q-4)(q-5) + 13(q-4)(q-5)(q-6) + 84\lambda^2 + \\
&\quad 136\lambda(q-4) + 49(q-4)(q-5) + 58\lambda + 56q - 212. \\
2Z_C U_C^v &= 14\lambda^5 + 4\lambda^4(q-4) + 50\lambda^4 + 63\lambda^3(q-4) + 24\lambda^2(q-4)(q-5) + 3\lambda(q-4)(q-5)(q-6) + 66\lambda^3 + \\
&\quad 78\lambda^2(q-4) + 21\lambda(q-4)(q-5) + 46\lambda^2 + 38\lambda(q-4) + 16\lambda. \\
6Z_C U_C^N &= 30\lambda^5 + 8\lambda^4(q-4) + 128\lambda^4 + 165\lambda^3(q-4) + 66\lambda^2(q-4)(q-5) + 9\lambda(q-4)(q-5)(q-6) + 192\lambda^3 + \\
&\quad 240\lambda^2(q-4) + 69\lambda(q-4)(q-5) + 168\lambda^2 + 136\lambda(q-4) + 58\lambda. \\
\tilde{S}_C &= 2(2r^4t^8 + 16r^4t^7 + 12r^3t^8 + 56r^4t^6 + 104r^3t^7 + 28r^2t^8 + 112r^4t^5 + 396r^3t^6 + 260r^2t^7 + 31rt^8 + 140r^4t^4 + \\
&\quad 864r^3t^5 + 1064r^2t^6 + 301rt^7 + 14t^8 + 112r^4t^3 + 1180r^3t^4 + 2504r^2t^5 + 1298rt^6 + 138t^7 + 56r^4t^2 + \\
&\quad 1032r^3t^3 + 3704r^2t^4 + 3246rt^5 + 612t^6 + 16r^4t + 564r^3t^2 + 3524r^2t^3 + 5146rt^4 + 1596t^5 + 2r^4 + 176r^3t + \\
&\quad 2104r^2t^2 + 5292rt^3 + 2676t^4 + 24r^3 + 720r^2t + 3444rt^2 + 2952t^3 + 108r^2 + 1296rt + 2088t^2 + 216r + 864t + \\
&\quad 162)(4r^4t^6 + 24r^4t^5 + 15r^3t^6 + 60r^4t^4 + 120r^3t^5 + 21r^2t^6 + 80r^4t^3 + 378r^3t^4 + 210r^2t^5 + 12rt^6 + 60r^4t^2 + \\
&\quad 612r^3t^3 + 828r^2t^4 + 150rt^5 + 2t^6 + 24r^4t + 543r^3t^2 + 1650r^2t^3 + 741rt^4 + 36t^5 + 4r^4 + 252r^3t + 1767r^2t^2 + \\
&\quad 1836rt^3 + 225t^4 + 48r^3 + 972r^2t + 2421rt^2 + 702t^3 + 216r^2 + 1620rt + 1161t^2 + 432r + 972t + 324)(t+1)^3t. \\
D_C^U &= (6s^5t^8 + 48s^5t^7 + 58s^4t^8 + 168s^5t^6 + 511s^4t^7 + 218s^3t^8 + 336s^5t^5 + 1959s^4t^6 + 2113s^3t^7 + 398s^2t^8 + \\
&\quad 420s^5t^4 + 4274s^4t^5 + 8871s^3t^6 + 4223s^2t^7 + 352s^8 + 336s^5t^3 + 5810s^4t^4 + 21130s^3t^5 + 19395s^2t^6 + \\
&\quad 4061st^7 + 120t^8 + 168s^5t^2 + 5043s^4t^3 + 31304s^3t^4 + 50489s^2t^5 + 20349st^6 + 1500t^7 + 48s^5t + 2731s^4t^2 + \\
&\quad 29589s^3t^3 + 81725s^2t^4 + 57913st^5 + 8154t^6 + 6s^5 + 844s^4t + 17447s^3t^2 + 84468s^2t^3 + 102701st^4 + \\
&\quad 25302t^5 + 114s^4 + 5872s^3t + 54558s^2t^2 + 116628st^3 + 49236t^4 + 864s^3 + 20160s^2t + 83104st^2 + 61776t^3 + \\
&\quad 3264s^2 + 34048st + 48992t^2 + 6144s + 22528t + 4608)(s+4)(t+1)^3.
\end{aligned}$$

Local view 21 of 35.

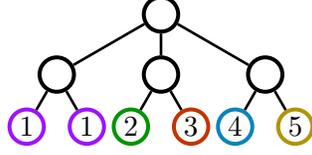

$$Z_C = 21\lambda^5 + 19\lambda^4(q-5) + 7\lambda^3(q-5)(q-6) + \lambda^2(q-5)(q-6)(q-7) + 44\lambda^4 + 64\lambda^3(q-5) + 30\lambda^2(q-5)(q-6) + 7\lambda(q-5)(q-6)(q-7) + (q-5)(q-6)(q-7)(q-8) + 104\lambda^3 + 148\lambda^2(q-5) + 81\lambda(q-5)(q-6) + 18(q-5)(q-6)(q-7) + 164\lambda^2 + 255\lambda(q-5) + 99(q-5)(q-6) + 204\lambda + 185q - 837.$$

$$2Z_C U_C^v = 31\lambda^5 + 18\lambda^4(q-5) + 3\lambda^3(q-5)(q-6) + 56\lambda^4 + 54\lambda^3(q-5) + 18\lambda^2(q-5)(q-6) + 3\lambda(q-5)(q-6)(q-7) + 96\lambda^3 + 102\lambda^2(q-5) + 33\lambda(q-5)(q-6) + 116\lambda^2 + 99\lambda(q-5) + 76\lambda.$$

$$6Z_C U_C^N = 105\lambda^5 + 76\lambda^4(q-5) + 21\lambda^3(q-5)(q-6) + 2\lambda^2(q-5)(q-6)(q-7) + 176\lambda^4 + 192\lambda^3(q-5) + 60\lambda^2(q-5)(q-6) + 7\lambda(q-5)(q-6)(q-7) + 312\lambda^3 + 296\lambda^2(q-5) + 81\lambda(q-5)(q-6) + 328\lambda^2 + 255\lambda(q-5) + 204\lambda.$$

$$\begin{aligned} \tilde{S}_C = & 2(10r^8t^{14} + 144r^8t^{13} + 99r^7t^{14} + 964r^8t^{12} + 1533r^7t^{13} + 430r^6t^{14} + 3976r^8t^{11} + 11022r^7t^{12} + 7136r^6t^{13} + \\ & 1072r^5t^{14} + 11286r^8t^{10} + 48758r^7t^{11} + 54918r^6t^{12} + 18986r^5t^{13} + 1679r^4t^{14} + 23320r^8t^9 + 148228r^7t^{10} + \\ & 259776r^6t^{11} + 155835r^5t^{12} + 31583r^4t^{13} + 1692r^3t^{14} + 36168r^8t^8 + 327534r^7t^9 + 843710r^6t^{10} + 785811r^5t^{11} + \\ & 275450r^4t^{12} + 33608r^3t^{13} + 1068r^2t^{14} + 42768r^8t^7 + 542400r^7t^8 + 1990048r^6t^9 + 2719785r^5t^{10} + \\ & 1476282r^4t^{11} + 310277r^3t^{12} + 22268r^2t^{13} + 380rt^{14} + 38742r^8t^6 + 683760r^7t^7 + 3514868r^6t^8 + \\ & 6834669r^5t^9 + 5432027r^4t^{10} + 1762685r^3t^{11} + 216929r^2t^{12} + 8324rt^{13} + 56t^{14} + 26752r^8t^5 + 659295r^7t^6 + \\ & 4721776r^6t^7 + 12858321r^5t^8 + 14515701r^4t^9 + 6880744r^3t^{10} + 1303789r^2t^{11} + 85568rt^{12} + 1320t^{13} + \\ & 13860r^8t^4 + 483837r^7t^5 + 4847426r^6t^6 + 18395595r^5t^7 + 29049328r^4t^8 + 19520168r^3t^9 + 5391911r^2t^{10} + \\ & 544098rt^{11} + 14436t^{12} + 5224r^8t^3 + 266010r^7t^4 + 3784112r^6t^5 + 20107425r^5t^6 + 44223420r^4t^7 + \\ & 41501360r^3t^8 + 16221041r^2t^9 + 2383945rt^{10} + 97464t^{11} + 1354r^8t^2 + 106242r^7t^3 + 2210998r^6t^4 + \\ & 16708357r^5t^5 + 51457222r^4t^6 + 67173962r^3t^7 + 36604192r^2t^8 + 7604559rt^9 + 453414t^{10} + 216r^8t + \\ & 29138r^7t^2 + 937552r^6t^3 + 10388432r^5t^4 + 45534522r^4t^5 + 83176107r^3t^6 + 62948034r^2t^7 + 18208905rt^8 + \\ & 1535850t^9 + 16r^8 + 4912r^7t + 272738r^6t^2 + 4685910r^5t^3 + 30160152r^4t^4 + 78399711r^3t^5 + 82912248r^2t^6 + \\ & 33258087rt^7 + 3905586t^8 + 384r^7 + 48720r^6t + 1449450r^5t^2 + 14497740r^4t^3 + 55370394r^3t^4 + 83251908r^2t^5 + \\ & 46586205rt^6 + 7579062t^7 + 4032r^6 + 275184r^5t + 4780350r^4t^2 + 28411182r^3t^3 + 62738118r^2t^4 + \\ & 49831119rt^5 + 11290914t^6 + 24192r^5 + 967680r^4t + 10011222r^3t^2 + 34413336r^2t^3 + 40090140rt^4 + \\ & 12866850t^5 + 90720r^4 + 2168208r^3t + 12990294r^2t^2 + 23537466rt^3 + 11055528t^4 + 217728r^3 + 3020976r^2t + \\ & 9539694rt^2 + 6954660t^3 + 326592r^2 + 2391120rt + 3032640t^2 + 279936r + 822312t + 104976)(t+1)^3t. \end{aligned}$$

$$\begin{aligned} D_C^U = & (6s^5t^8 + 48s^5t^7 + 90s^4t^8 + 168s^5t^6 + 759s^4t^7 + 536s^3t^8 + 336s^5t^5 + 2805s^4t^6 + 4752s^3t^7 + 1584s^2t^8 + \\ & 420s^5t^4 + 5934s^4t^5 + 18498s^3t^6 + 14712s^2t^7 + 2320st^8 + 336s^5t^3 + 7860s^4t^4 + 41323s^3t^5 + 60150s^2t^6 + \\ & 22500st^7 + 1344t^8 + 168s^5t^2 + 6675s^4t^3 + 57969s^3t^4 + 141615s^2t^5 + 96312st^6 + 13584t^7 + 48s^5t + \\ & 3549s^4t^2 + 52305s^3t^3 + 210243s^2t^4 + 238396st^5 + 60672t^6 + 6s^5 + 1080s^4t + 29645s^3t^2 + 201705s^2t^3 + \\ & 374142st^4 + 157376t^5 + 144s^4 + 9648s^3t + 122175s^2t^2 + 381903st^3 + 260616t^4 + 1380s^3 + 42720s^2t + \\ & 247875st^2 + 283140t^3 + 6600s^2 + 93600st + 197500t^2 + 15750s + 81000t + 15000)(s+5)(t+1)^3. \end{aligned}$$

Local view 22 of 35.

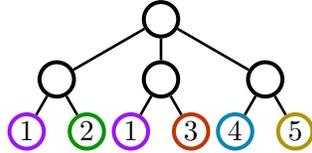

$$Z_C = 3\lambda^5 + \lambda^4(q-5) + 44\lambda^4 + 59\lambda^3(q-5) + 33\lambda^2(q-5)(q-6) + 9\lambda(q-5)(q-6)(q-7) + (q-5)(q-6)(q-7)(q-8) + 109\lambda^3 + 180\lambda^2(q-5) + 96\lambda(q-5)(q-6) + 17(q-5)(q-6)(q-7) + 204\lambda^2 + 278\lambda(q-5) + 88(q-5)(q-6) + 199\lambda + 153q - 699.$$

$$\begin{aligned}
2Z_C U_C^v &= 7\lambda^5 + 2\lambda^4(q-5) + 72\lambda^4 + 69\lambda^3(q-5) + 24\lambda^2(q-5)(q-6) + 3\lambda(q-5)(q-6)(q-7) + 117\lambda^3 + \\
&\quad 120\lambda^2(q-5) + 30\lambda(q-5)(q-6) + 122\lambda^2 + 82\lambda(q-5) + 57\lambda. \\
6Z_C U_C^N &= 15\lambda^5 + 4\lambda^4(q-5) + 176\lambda^4 + 177\lambda^3(q-5) + 66\lambda^2(q-5)(q-6) + 9\lambda(q-5)(q-6)(q-7) + 327\lambda^3 + \\
&\quad 360\lambda^2(q-5) + 96\lambda(q-5)(q-6) + 408\lambda^2 + 278\lambda(q-5) + 199\lambda. \\
\tilde{S}_C &= 2(2r^4t^8 + 16r^4t^7 + 12r^3t^8 + 56r^4t^6 + 104r^3t^7 + 28r^2t^8 + 112r^4t^5 + 396r^3t^6 + 260r^2t^7 + 31rt^8 + 140r^4t^4 + \\
&\quad 864r^3t^5 + 1064r^2t^6 + 301rt^7 + 14t^8 + 112r^4t^3 + 1180r^3t^4 + 2504r^2t^5 + 1298rt^6 + 138t^7 + 56r^4t^2 + \\
&\quad 1032r^3t^3 + 3704r^2t^4 + 3246rt^5 + 612t^6 + 16r^4t + 564r^3t^2 + 3524r^2t^3 + 5146rt^4 + 1596t^5 + 2r^4 + 176r^3t + \\
&\quad 2104r^2t^2 + 5292rt^3 + 2676t^4 + 24r^3 + 720r^2t + 3444rt^2 + 2952t^3 + 108r^2 + 1296rt + 2088t^2 + 216r + 864t + \\
&\quad 162)(5r^4t^6 + 30r^4t^5 + 18r^3t^6 + 75r^4t^4 + 147r^3t^5 + 24r^2t^6 + 100r^4t^3 + 468r^3t^4 + 249r^2t^5 + 12rt^6 + 75r^4t^2 + \\
&\quad 762r^3t^3 + 1008r^2t^4 + 168rt^5 + t^6 + 30r^4t + 678r^3t^2 + 2040r^2t^3 + 876rt^4 + 36t^5 + 5r^4 + 315r^3t + 2202r^2t^2 + \\
&\quad 2241rt^3 + 252t^4 + 60r^3 + 1215r^2t + 3006rt^2 + 837t^3 + 270r^2 + 2025rt + 1431t^2 + 540r + 1215t + 405)(t+1)^3t. \\
D_C^U &= (6s^5t^8 + 48s^5t^7 + 86s^4t^8 + 168s^5t^6 + 737s^4t^7 + 486s^3t^8 + 336s^5t^5 + 2757s^4t^6 + 4453s^3t^7 + 1354s^2t^8 + \\
&\quad 420s^5t^4 + 5884s^4t^5 + 17787s^3t^6 + 13216s^2t^7 + 1860s^8 + 336s^5t^3 + 7840s^4t^4 + 40506s^3t^5 + 56274s^2t^6 + \\
&\quad 19247st^7 + 1008t^8 + 168s^5t^2 + 6681s^4t^3 + 57584s^3t^4 + 136711s^2t^5 + 87123st^6 + 11004t^7 + 48s^5t + \\
&\quad 3557s^4t^2 + 52377s^3t^3 + 207559s^2t^4 + 225599st^5 + 52716t^6 + 6s^5 + 1082s^4t + 29787s^3t^2 + 201945s^2t^3 + \\
&\quad 366091st^4 + 145164t^5 + 144s^4 + 9688s^3t + 123105s^2t^2 + 381903st^3 + 251836t^4 + 1380s^3 + 43020s^2t + \\
&\quad 250525st^2 + 282390t^3 + 6600s^2 + 94600st + 200250t^2 + 15750s + 82250t + 15000)(s+5)(t+1)^3.
\end{aligned}$$

Local view 23 of 35.

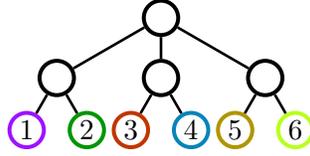

$$\begin{aligned}
Z_C &= 54\lambda^4 + 63\lambda^3(q-6) + 33\lambda^2(q-6)(q-7) + 9\lambda(q-6)(q-7)(q-8) + (q-6)(q-7)(q-8)(q-9) + 162\lambda^3 + \\
&\quad 240\lambda^2(q-6) + 123\lambda(q-6)(q-7) + 21(q-6)(q-7)(q-8) + 378\lambda^2 + 474\lambda(q-6) + 139(q-6)(q-7) + \\
&\quad 486\lambda + 328q - 1752. \\
2Z_C U_C^v &= 90\lambda^4 + 75\lambda^3(q-6) + 24\lambda^2(q-6)(q-7) + 3\lambda(q-6)(q-7)(q-8) + 180\lambda^3 + 162\lambda^2(q-6) + \\
&\quad 39\lambda(q-6)(q-7) + 234\lambda^2 + 144\lambda(q-6) + 144\lambda. \\
6Z_C U_C^N &= 216\lambda^4 + 189\lambda^3(q-6) + 66\lambda^2(q-6)(q-7) + 9\lambda(q-6)(q-7)(q-8) + 486\lambda^3 + 480\lambda^2(q-6) + \\
&\quad 123\lambda(q-6)(q-7) + 756\lambda^2 + 474\lambda(q-6) + 486\lambda. \\
\tilde{S}_C &= 6(2r^4t^8 + 16r^4t^7 + 12r^3t^8 + 56r^4t^6 + 104r^3t^7 + 28r^2t^8 + 112r^4t^5 + 396r^3t^6 + 260r^2t^7 + 31rt^8 + 140r^4t^4 + \\
&\quad 864r^3t^5 + 1064r^2t^6 + 301rt^7 + 14t^8 + 112r^4t^3 + 1180r^3t^4 + 2504r^2t^5 + 1298rt^6 + 138t^7 + 56r^4t^2 + \\
&\quad 1032r^3t^3 + 3704r^2t^4 + 3246rt^5 + 612t^6 + 16r^4t + 564r^3t^2 + 3524r^2t^3 + 5146rt^4 + 1596t^5 + 2r^4 + 176r^3t + \\
&\quad 2104r^2t^2 + 5292rt^3 + 2676t^4 + 24r^3 + 720r^2t + 3444rt^2 + 2952t^3 + 108r^2 + 1296rt + 2088t^2 + 216r + \\
&\quad 864t + 162)(2r^3t^4 + 8r^3t^3 + 7r^2t^4 + 12r^3t^2 + 38r^2t^3 + 9rt^4 + 8r^3t + 73r^2t^2 + 57rt^3 + 4t^4 + 2r^3 + 60r^2t + \\
&\quad 138rt^2 + 27t^3 + 18r^2 + 144rt + 81t^2 + 54r + 108t + 54)(rt+r+3)(t+1)^4t. \\
D_C^U &= 3(2s^4t^6 + 12s^4t^5 + 32s^3t^6 + 30s^4t^4 + 203s^3t^5 + 190s^2t^6 + 40s^4t^3 + 537s^3t^4 + 1270s^2t^5 + 496st^6 + 30s^4t^2 + \\
&\quad 759s^3t^3 + 3549s^2t^4 + 3471st^5 + 480t^6 + 12s^4t + 605s^3t^2 + 5318s^2t^3 + 10224st^4 + 3480t^5 + 2s^4 + 258s^3t + \\
&\quad 4515s^2t^2 + 16253st^3 + 10770t^4 + 46s^3 + 2062s^2t + 14740st^2 + 18190t^3 + 396s^2 + 7248st + 17700t^2 + \\
&\quad 1512s + 9432t + 2160)(st+s+3t+6)(s+6)(t+1)^4.
\end{aligned}$$

Local view 24 of 35.

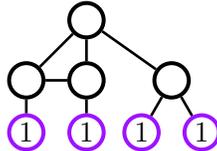

$$\begin{aligned}
 Z_C &= \lambda^8 + 5\lambda^5(q-1) + 5\lambda^4(q-1) + 8\lambda^3(q-1)(q-2) + \lambda^2(q-1)(q-2)(q-3) + 2\lambda^3(q-1) + \\
 &\quad 9\lambda^2(q-1)(q-2) + 6\lambda(q-1)(q-2)(q-3) + (q-1)(q-2)(q-3)(q-4) + 2\lambda^2(q-1) + \\
 &\quad 6\lambda(q-1)(q-2) + 3(q-1)(q-2)(q-3) + \lambda(q-1) + 2(q-1)(q-2). \\
 2Z_C U_C^v &= 3\lambda^8 + 8\lambda^5(q-1) + 7\lambda^4(q-1) + 5\lambda^3(q-1)(q-2) + 4\lambda^3(q-1) + 11\lambda^2(q-1)(q-2) + \\
 &\quad 3\lambda(q-1)(q-2)(q-3) + 2\lambda^2(q-1) + 2\lambda(q-1)(q-2). \\
 6Z_C U_C^N &= 9\lambda^8 + 28\lambda^5(q-1) + 23\lambda^4(q-1) + 27\lambda^3(q-1)(q-2) + 2\lambda^2(q-1)(q-2)(q-3) + 6\lambda^3(q-1) + \\
 &\quad 19\lambda^2(q-1)(q-2) + 7\lambda(q-1)(q-2)(q-3) + 4\lambda^2(q-1) + 8\lambda(q-1)(q-2) + 2\lambda(q-1). \\
 \tilde{S}_C &= 2(2r^8t^{15} + 30r^8t^{14} + 22r^7t^{15} + 210r^8t^{13} + 348r^7t^{14} + 107r^6t^{15} + 910r^8t^{12} + 2572r^7t^{13} + 1772r^6t^{14} + 300r^5t^{15} + \\
 &\quad 2730r^8t^{11} + 11776r^7t^{12} + 13752r^6t^{13} + 5168r^5t^{14} + 529r^4t^{15} + 6006r^8t^{10} + 37338r^7t^{11} + 66265r^6t^{12} + \\
 &\quad 41910r^5t^{13} + 9431r^4t^{14} + 597r^3t^{15} + 10010r^8t^9 + 86812r^7t^{10} + 221472r^6t^{11} + 211780r^5t^{12} + 79589r^4t^{13} + \\
 &\quad 10995r^3t^{14} + 415r^2t^{15} + 12870r^8t^8 + 152856r^7t^9 + 543324r^6t^{10} + 744278r^5t^{11} + 420433r^4t^{12} + 96326r^3t^{13} + \\
 &\quad 7942r^2t^{14} + 158r^2t^{15} + 12870r^8t^7 + 207504r^7t^8 + 1009908r^6t^9 + 1923580r^5t^{10} + 1550155r^4t^{11} + 530694r^3t^{12} + \\
 &\quad 72342r^2t^{13} + 3208r^2t^{14} + 24t^{15} + 10010r^8t^6 + 218922r^7t^7 + 1447350r^6t^8 + 3771308r^5t^9 + 4214356r^4t^{10} + \\
 &\quad 2048859r^3t^{11} + 415447r^2t^{12} + 30651rt^{13} + 544t^{14} + 6006r^8t^5 + 179476r^7t^6 + 1611639r^6t^7 + 5704600r^5t^8 + \\
 &\quad 8707559r^4t^9 + 5851225r^3t^{10} + 1677481r^2t^{11} + 183991rt^{12} + 5566t^{13} + 2730r^8t^4 + 113388r^7t^5 + 1393760r^6t^6 + \\
 &\quad 6705848r^5t^7 + 13897154r^4t^8 + 12729936r^3t^9 + 5026737r^2t^{10} + 777101rt^{11} + 35186t^{12} + 910r^8t^3 + 54208r^7t^4 + \\
 &\quad 928196r^6t^5 + 6121480r^5t^6 + 17247938r^4t^7 + 21428316r^3t^8 + 11506629r^2t^9 + 2441885rt^{10} + 155742t^{11} + \\
 &\quad 210r^8t^2 + 18982r^7t^3 + 467361r^6t^4 + 4301614r^5t^5 + 16628045r^4t^6 + 28079804r^3t^7 + 20421375r^2t^8 + \\
 &\quad 5877780r^9 + 513150t^{10} + 30r^8t + 4596r^7t^2 + 172198r^6t^3 + 2284180r^5t^4 + 12340032r^4t^5 + 28600134r^3t^6 + \\
 &\quad 28254375r^2t^7 + 10995174rt^8 + 1298340t^9 + 2r^8 + 688r^7t + 43824r^6t^2 + 886950r^5t^3 + 6918813r^4t^4 + \\
 &\quad 22431804r^3t^5 + 30413628r^2t^6 + 16062570rt^7 + 2559519t^8 + 48r^7 + 6888r^6t + 237708r^5t^2 + 2835810r^4t^3 + \\
 &\quad 13294656r^3t^4 + 25226640r^2t^5 + 18278622rt^6 + 3948642t^7 + 504r^6 + 39312r^5t + 801900r^4t^2 + 5760450r^3t^3 + \\
 &\quad 15819651r^2t^4 + 16042698rt^5 + 4752189t^6 + 3024r^5 + 139860r^4t + 1722060r^3t^2 + 7256466r^2t^3 + 10654092rt^4 + \\
 &\quad 4415958t^5 + 11340r^4 + 317520r^3t + 2297808r^2t^2 + 5180274rt^3 + 3108213t^4 + 27216r^3 + 449064r^2t + \\
 &\quad 1740852rt^2 + 1603800t^3 + 40824r^2 + 361584rt + 572994t^2 + 34992r + 126846t + 13122)(r+2)(t+1)^3. \\
 \tilde{S}_C|_{q=2} &= 2(4t^3 + 7t^2 + 6t + 2)(t+2)^8(t+1)^3. \\
 D_C^U &= (4s^4t^8 + 32s^4t^7 + 22s^3t^8 + 112s^4t^6 + 195s^3t^7 + 44s^2t^8 + 224s^4t^5 + 753s^3t^6 + 436s^2t^7 + 38st^8 + 280s^4t^4 + 1658s^3t^5 + \\
 &\quad 1859s^2t^6 + 423st^7 + 12t^8 + 224s^4t^3 + 2280s^3t^4 + 4496s^2t^5 + 1989st^6 + 150t^7 + 112s^4t^2 + 2007s^3t^3 + 6790s^2t^4 + \\
 &\quad 5272st^5 + 774t^6 + 32s^4t + 1105s^3t^2 + 6584s^2t^3 + 8734st^4 + 2240t^5 + 4s^4 + 348s^3t + 4011s^2t^2 + 9341st^3 + \\
 &\quad 4068t^4 + 48s^3 + 1404s^2t + 6327st^2 + 4812t^3 + 216s^2 + 2484st + 3645t^2 + 432s + 1620t + 324)(s+3)(s+2)(t+1)^3. \\
 D_C^U|_{q=2} &= 2(3t^2 + 6t + 4)(t+2)^4(t+1)^3.
 \end{aligned}$$

Local view 25 of 35.

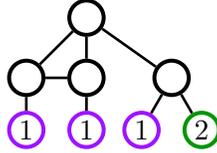

$$\begin{aligned}
 Z_C &= \lambda^7 + \lambda^6 + \lambda^5(q-2) + 2\lambda^5 + 8\lambda^4(q-2) + 2\lambda^3(q-2)(q-3) + 6\lambda^4 + 16\lambda^3(q-2) + 21\lambda^2(q-2)(q-3) + \\
 &\quad 8\lambda(q-2)(q-3)(q-4) + (q-2)(q-3)(q-4)(q-5) + 5\lambda^3 + 29\lambda^2(q-2) + 24\lambda(q-2)(q-3) + \\
 &\quad 6(q-2)(q-3)(q-4) + \lambda^2 + 9\lambda(q-2) + 8(q-2)(q-3) + 2q - 4. \\
 2Z_C U_C^v &= 3\lambda^7 + 2\lambda^6 + 2\lambda^5(q-2) + 4\lambda^5 + 12\lambda^4(q-2) + 2\lambda^3(q-2)(q-3) + 10\lambda^4 + 20\lambda^3(q-2) + \\
 &\quad 17\lambda^2(q-2)(q-3) + 3\lambda(q-2)(q-3)(q-4) + 5\lambda^3 + 21\lambda^2(q-2) + 8\lambda(q-2)(q-3) + 2\lambda(q-2). \\
 6Z_C U_C^N &= 8\lambda^7 + 7\lambda^6 + 6\lambda^5(q-2) + 12\lambda^5 + 38\lambda^4(q-2) + 8\lambda^3(q-2)(q-3) + 26\lambda^4 + 52\lambda^3(q-2) + \\
 &\quad 45\lambda^2(q-2)(q-3) + 9\lambda(q-2)(q-3)(q-4) + 16\lambda^3 + 63\lambda^2(q-2) + 28\lambda(q-2)(q-3) + 3\lambda^2 + 12\lambda(q-2).
 \end{aligned}$$

$$\begin{aligned} \tilde{Z}_C &= (4r^8t^{14} + 56r^8t^{13} + 44r^7t^{14} + 364r^8t^{12} + 652r^7t^{13} + 208r^6t^{14} + 1456r^8t^{11} + 4484r^7t^{12} + 3266r^6t^{13} + 554r^5t^{14} + \\ & 4004r^8t^{10} + 18968r^7t^{11} + 23784r^6t^{12} + 9220r^5t^{13} + 910r^4t^{14} + 8008r^8t^9 + 55132r^7t^{10} + 106466r^6t^{11} + \\ & 71092r^5t^{12} + 16066r^4t^{13} + 940r^3t^{14} + 12012r^8t^8 + 116468r^7t^9 + 327264r^6t^{10} + 336710r^5t^{11} + 131148r^4t^{12} + \\ & 17675r^3t^{13} + 590r^2t^{14} + 13728r^8t^7 + 184404r^7t^8 + 730716r^6t^9 + 1094526r^5t^{10} + 656896r^4t^{11} + 152915r^3t^{12} + \\ & 11937r^2t^{13} + 202rt^{14} + 12012r^8t^6 + 222288r^7t^7 + 1222092r^6t^8 + 2583346r^5t^9 + 2257058r^4t^{10} + 809875r^3t^{11} + \\ & 109880r^2t^{12} + 4490rt^{13} + 28t^{14} + 8008r^8t^5 + 204996r^7t^6 + 1555188r^6t^7 + 4565542r^5t^8 + 5629710r^4t^9 + \\ & 2939665r^3t^{10} + 615979r^2t^{11} + 44347rt^{12} + 712t^{13} + 4004r^8t^4 + 143924r^7t^5 + 1513152r^6t^6 + 6137370r^5t^7 + \\ & 10513862r^4t^8 + 7744626r^3t^9 + 2361556r^2t^{10} + 263944rt^{11} + 7662t^{12} + 1456r^8t^3 + 75724r^7t^4 + 1120138r^6t^5 + \\ & 6305888r^5t^6 + 14935738r^4t^7 + 15280200r^3t^8 + 6567844r^2t^9 + 1069469rt^{10} + 48700t^{11} + 364r^8t^2 + \\ & 28952r^7t^3 + 621008r^6t^4 + 4927678r^5t^5 + 16217196r^4t^6 + 22941188r^3t^7 + 13683768r^2t^8 + 3138850rt^9 + \\ & 208914t^{10} + 56r^8t + 7604r^7t^2 + 250026r^6t^3 + 2882722r^5t^4 + 13392248r^4t^5 + 26337976r^3t^6 + 21709866r^2t^7 + \\ & 6902040rt^8 + 647076t^9 + 4r^8 + 1228r^7t + 69104r^6t^2 + 1224152r^5t^3 + 8278770r^4t^4 + 23007300r^3t^5 + \\ & 26361756r^2t^6 + 11567754rt^7 + 1500912t^8 + 92r^7 + 11736r^6t + 356688r^5t^2 + 3714366r^4t^3 + 15050172r^3t^4 + \\ & 24378930r^2t^5 + 14857560rt^6 + 2656044t^7 + 924r^6 + 63828r^5t + 1143180r^4t^2 + 7147080r^3t^3 + 16898112r^2t^4 + \\ & 14554674rt^5 + 3607848t^6 + 5292r^5 + 216000r^4t + 2328372r^3t^2 + 8509590r^2t^3 + 10702854rt^4 + 3745116t^5 + \\ & 18900r^4 + 465588r^3t + 2941272r^2t^2 + 5726376rt^3 + 2924586t^4 + 43092r^3 + 624024r^2t + 2105352rt^2 + \\ & 1665522t^3 + 61236r^2 + 475308rt + 653184t^2 + 49572r + 157464t + 17496)(rt + r + 2t + 3)(t + 1)^3. \end{aligned}$$

$$\tilde{S}_C|_{q=2} = 4(t^3 + 2t^2 + 3t + 1)(t + 2)^8(t + 1)^3.$$

$$\begin{aligned} D_C^U &= (4s^4t^8 + 32s^4t^7 + 22s^3t^8 + 112s^4t^6 + 195s^3t^7 + 44s^2t^8 + 224s^4t^5 + 753s^3t^6 + 436s^2t^7 + 38st^8 + 280s^4t^4 + 1658s^3t^5 + \\ & 1859s^2t^6 + 423st^7 + 12t^8 + 224s^4t^3 + 2280s^3t^4 + 4496s^2t^5 + 1989st^6 + 150t^7 + 112s^4t^2 + 2007s^3t^3 + 6790s^2t^4 + \\ & 5272st^5 + 774t^6 + 32s^4t + 1105s^3t^2 + 6584s^2t^3 + 8734st^4 + 2240t^5 + 4s^4 + 348s^3t + 4011s^2t^2 + 9341st^3 + 4068t^4 + \\ & 48s^3 + 1404s^2t + 6327st^2 + 4812t^3 + 216s^2 + 2484st + 3645t^2 + 432s + 1620t + 324)(st + s + t + 2)(s + 3)(t + 1)^2. \end{aligned}$$

$$D_C^U|_{q=2} = 2(3t^2 + 6t + 4)(t + 2)^4(t + 1)^2.$$

*Local view 26 of 35.*

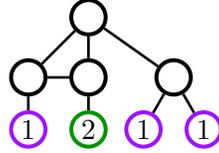

$$\begin{aligned} Z_C &= \lambda^7 + 2\lambda^6 + 2\lambda^5(q - 2) + 3\lambda^5 + 12\lambda^4(q - 2) + 7\lambda^3(q - 2)(q - 3) + \lambda^2(q - 2)(q - 3)(q - 4) + 4\lambda^4 + \\ & 15\lambda^3(q - 2) + 15\lambda^2(q - 2)(q - 3) + 6\lambda(q - 2)(q - 3)(q - 4) + (q - 2)(q - 3)(q - 4)(q - 5) + 3\lambda^3 + \\ & 17\lambda^2(q - 2) + 21\lambda(q - 2)(q - 3) + 7(q - 2)(q - 3)(q - 4) + 2\lambda^2 + 15\lambda(q - 2) + 12(q - 2)(q - 3) + \lambda + 4q - 8. \\ 2Z_C U_C^v &= 3\lambda^7 + 4\lambda^6 + 4\lambda^5(q - 2) + 5\lambda^5 + 14\lambda^4(q - 2) + 5\lambda^3(q - 2)(q - 3) + 6\lambda^4 + 17\lambda^3(q - 2) + 11\lambda^2(q - 2)(q - 3) + \\ & 3\lambda(q - 2)(q - 3)(q - 4) + 3\lambda^3 + 13\lambda^2(q - 2) + 11\lambda(q - 2)(q - 3) + 2\lambda^2 + 9\lambda(q - 2) + \lambda. \\ 6Z_C U_C^N &= 8\lambda^7 + 13\lambda^6 + 11\lambda^5(q - 2) + 17\lambda^5 + 54\lambda^4(q - 2) + 23\lambda^3(q - 2)(q - 3) + 2\lambda^2(q - 2)(q - 3)(q - 4) + 18\lambda^4 + \\ & 49\lambda^3(q - 2) + 33\lambda^2(q - 2)(q - 3) + 7\lambda(q - 2)(q - 3)(q - 4) + 10\lambda^3 + 39\lambda^2(q - 2) + 25\lambda(q - 2)(q - 3) + \\ & 5\lambda^2 + 18\lambda(q - 2) + \lambda. \end{aligned}$$

$$\begin{aligned} \tilde{S}_C &= (4r^9t^{16} + 64r^9t^{15} + 56r^8t^{16} + 480r^9t^{14} + 936r^8t^{15} + 344r^7t^{16} + 2240r^9t^{13} + 7332r^8t^{14} + 6008r^7t^{15} + 1218r^6t^{16} + \\ &7280r^9t^{12} + 35724r^8t^{13} + 49178r^7t^{14} + 22248r^6t^{15} + 2747r^5t^{16} + 17472r^9t^{11} + 121160r^8t^{12} + 250336r^7t^{13} + \\ &190418r^6t^{14} + 52515r^5t^{15} + 4112r^4t^{16} + 32032r^9t^{10} + 303264r^8t^{11} + 886706r^7t^{12} + 1013216r^6t^{13} + \\ &470127r^5t^{14} + 82245r^4t^{15} + 4115r^3t^{16} + 45760r^9t^9 + 579436r^8t^{10} + 2316724r^7t^{11} + 3749964r^6t^{12} + \\ &2615189r^5t^{13} + 769711r^4t^{14} + 85886r^3t^{15} + 2682r^2t^{16} + 51480r^9t^8 + 862004r^8t^9 + 4617556r^7t^{10} + \\ &10232436r^6t^{11} + 10113999r^5t^{12} + 4473676r^4t^{13} + 838579r^3t^{14} + 58030r^2t^{15} + 1046rt^{16} + 45760r^9t^7 + \\ &1009008r^8t^8 + 7160496r^7t^9 + 21287484r^6t^{10} + 28825339r^5t^{11} + 18070074r^4t^{12} + 5084426r^3t^{13} + 588544r^2t^{14} + \\ &23182rt^{15} + 188t^{16} + 32032r^9t^6 + 932360r^8t^7 + 8729532r^7t^8 + 34432992r^6t^9 + 62605753r^5t^{10} + 53770851r^4t^{11} + \\ &21423163r^3t^{12} + 3711467r^2t^{13} + 242417rt^{14} + 4196t^{15} + 17472r^9t^5 + 677820r^8t^6 + 8393552r^7t^7 + \\ &43753866r^6t^8 + 105665559r^5t^9 + 121896961r^4t^{10} + 66498786r^3t^{11} + 16279291r^2t^{12} + 1582660rt^{13} + 44778t^{14} + \\ &7280r^9t^4 + 383604r^8t^5 + 6343346r^7t^6 + 43812864r^6t^7 + 140019440r^5t^8 + 214675450r^4t^9 + 157253303r^3t^{10} + \\ &52635547r^2t^{11} + 7205113rt^{12} + 300812t^{13} + 2240r^9t^3 + 165672r^8t^4 + 3728048r^7t^5 + 34451082r^6t^6 + \\ &146114290r^5t^7 + 296722376r^4t^8 + 288879206r^3t^9 + 129709697r^2t^{10} + 24218883rt^{11} + 1416222t^{12} + 480r^9t^2 + \\ &52784r^8t^3 + 1670218r^7t^4 + 21045200r^6t^5 + 119638620r^5t^6 + 322830314r^4t^7 + 416463980r^3t^8 + 248394900r^2t^9 + \\ &62114124rt^{10} + 4937946t^{11} + 64r^9t + 11700r^8t^2 + 551396r^7t^3 + 9789224r^6t^4 + 76032544r^5t^5 + 275439646r^4t^6 + \\ &472527116r^3t^7 + 373394412r^2t^8 + 123892263rt^9 + 13161564t^{10} + 4r^9 + 1612r^8t + 126496r^7t^2 + 3351300r^6t^3 + \\ &36753882r^5t^4 + 182267148r^4t^5 + 420322494r^3t^6 + 441829224r^2t^7 + 194096880rt^8 + 27317358t^9 + 104r^8 + \\ &18016r^7t + 796200r^6t^2 + 13059396r^5t^3 + 91653024r^4t^4 + 289844232r^3t^5 + 409893066r^2t^6 + 239481954rt^7 + \\ &44576406t^8 + 1200r^7 + 117264r^6t + 3215376r^5t^2 + 33833700r^4t^3 + 151766334r^3t^4 + 294750576r^2t^5 + \\ &231755796rt^6 + 57332502t^7 + 8064r^6 + 489888r^5t + 8640000r^4t^2 + 58269132r^3t^3 + 160869240r^2t^4 + \\ &173884968rt^5 + 57878226t^6 + 34776r^5 + 1362312r^4t + 15448320r^3t^2 + 64316268r^2t^3 + 99015534rt^4 + \\ &45328896t^5 + 99792r^4 + 2522016r^3t + 17723448r^2t^2 + 41275980rt^3 + 26953560t^4 + 190512r^3 + 2997648r^2t + \\ &11838960rt^2 + 11731068t^3 + 233280r^2 + 2076192rt + 3507948t^2 + 166212r + 638604t + 52488)(t + 1)^2. \end{aligned}$$

$$\tilde{S}_C|_{q=2} = 2(t^4 + 4t^3 + 7t^2 + 6t + 1)(t^2 + 2t + 2)(t + 2)^8(t + 1)^2.$$

$$\begin{aligned} D_C^U &= (4s^5t^9 + 36s^5t^8 + 28s^4t^9 + 144s^5t^7 + 269s^4t^8 + 79s^3t^9 + 336s^5t^6 + 1152s^4t^7 + 802s^3t^8 + 113s^2t^9 + \\ &504s^5t^5 + 2887s^4t^6 + 3645s^3t^7 + 1195s^2t^8 + 82st^9 + 504s^5t^4 + 4666s^4t^5 + 9743s^3t^6 + 5700s^2t^7 + 890st^8 + \\ &24t^9 + 336s^5t^3 + 5043s^4t^4 + 16889s^3t^5 + 16121s^2t^6 + 4401st^7 + 264t^8 + 144s^5t^2 + 3644s^4t^3 + 19692s^3t^4 + \\ &29821s^2t^5 + 13053st^6 + 1338t^7 + 36s^5t + 1697s^4t^2 + 15439s^3t^3 + 37425s^2t^4 + 25626st^5 + 4126t^6 + 4s^5 + \\ &462s^4t + 7843s^3t^2 + 31854s^2t^3 + 34530st^4 + 8552t^5 + 56s^4 + 2340s^3t + 17715s^2t^2 + 31909st^3 + 12342t^4 + \\ &312s^3 + 5832s^2t + 19485st^2 + 12378t^3 + 864s^2 + 7128st + 8316t^2 + 1188s + 3402t + 648)(s + 3)(t + 1)^2. \end{aligned}$$

$$D_C^U|_{q=2} = 4(t^2 + 2t + 2)(t + 2)^4(t + 1)^2.$$

Local view 27 of 35.

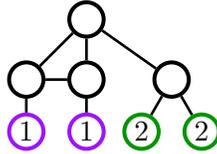

$$\begin{aligned} Z_C &= \lambda^7 + 3\lambda^6 + 3\lambda^5(q - 2) + 2\lambda^5 + 11\lambda^4(q - 2) + 8\lambda^3(q - 2)(q - 3) + \lambda^2(q - 2)(q - 3)(q - 4) + 2\lambda^4 + \\ &14\lambda^3(q - 2) + 12\lambda^2(q - 2)(q - 3) + 6\lambda(q - 2)(q - 3)(q - 4) + (q - 2)(q - 3)(q - 4)(q - 5) + 5\lambda^3 + \\ &16\lambda^2(q - 2) + 24\lambda(q - 2)(q - 3) + 7(q - 2)(q - 3)(q - 4) + 3\lambda^2 + 19\lambda(q - 2) + 11(q - 2)(q - 3) + 2q - 4. \\ 2Z_C U_C^v &= 2\lambda^7 + 7\lambda^6 + 4\lambda^5(q - 2) + 4\lambda^5 + 15\lambda^4(q - 2) + 5\lambda^3(q - 2)(q - 3) + 2\lambda^4 + 14\lambda^3(q - 2) + 11\lambda^2(q - 2)(q - 3) + \\ &3\lambda(q - 2)(q - 3)(q - 4) + 6\lambda^3 + 16\lambda^2(q - 2) + 11\lambda(q - 2)(q - 3) + 3\lambda^2 + 8\lambda(q - 2). \\ 6Z_C U_C^N &= 8\lambda^7 + 21\lambda^6 + 18\lambda^5(q - 2) + 10\lambda^5 + 47\lambda^4(q - 2) + 27\lambda^3(q - 2)(q - 3) + 2\lambda^2(q - 2)(q - 3)(q - 4) + 8\lambda^4 + \\ &48\lambda^3(q - 2) + 25\lambda^2(q - 2)(q - 3) + 7\lambda(q - 2)(q - 3)(q - 4) + 18\lambda^3 + 34\lambda^2(q - 2) + 29\lambda(q - 2)(q - 3) + \\ &7\lambda^2 + 24\lambda(q - 2). \end{aligned}$$

$$\begin{aligned} \tilde{S}_C &= 2(2r^9t^{17} + 34r^9t^{16} + 30r^8t^{17} + 272r^9t^{15} + 528r^8t^{16} + 193r^7t^{17} + 1360r^9t^{14} + 4374r^8t^{15} + 3523r^7t^{16} + \\ &706r^6t^{17} + 4760r^9t^{13} + 22648r^8t^{14} + 30289r^7t^{15} + 13377r^6t^{16} + 1632r^5t^{17} + 12376r^9t^{12} + 82082r^8t^{13} + \\ &162831r^7t^{14} + 119478r^6t^{15} + 32080r^5t^{16} + 2488r^4t^{17} + 24752r^9t^{11} + 220948r^8t^{12} + 612812r^7t^{13} + \\ &667658r^6t^{14} + 297594r^5t^{15} + 50655r^4t^{16} + 2511r^3t^{17} + 38896r^9t^{10} + 457366r^8t^{11} + 1712852r^7t^{12} + \\ &2612872r^6t^{13} + 1728785r^5t^{14} + 487512r^4t^{15} + 52850r^3t^{16} + 1620r^2t^{17} + 48620r^9t^9 + 743600r^8t^{10} + \\ &3680782r^7t^{11} + 7595415r^6t^{12} + 7037884r^5t^{13} + 2942040r^4t^{14} + 526887r^3t^{15} + 35199r^2t^{16} + 606rt^{17} + \\ &48620r^9t^8 + 961246r^8t^9 + 6209918r^7t^{10} + 16974252r^6t^{11} + 21291234r^5t^{12} + 12454960r^4t^{13} + 3299365r^3t^{14} + \\ &362982r^2t^{15} + 13588rt^{16} + 100t^{17} + 38896r^9t^7 + 993564r^8t^8 + 8325537r^7t^9 + 29774808r^6t^{10} + 49529088r^5t^{11} + \\ &39212682r^4t^{12} + 14513697r^3t^{13} + 2355570r^2t^{14} + 144792rt^{15} + 2316t^{16} + 24752r^9t^6 + 821106r^8t^7 + \\ &8918899r^7t^8 + 41485986r^6t^9 + 90436566r^5t^{10} + 94982130r^4t^{11} + 47533145r^3t^{12} + 10756318r^2t^{13} + \\ &972620rt^{14} + 25488t^{15} + 12376r^9t^5 + 539448r^8t^6 + 7633285r^7t^7 + 46159759r^6t^8 + 131141028r^5t^9 + \\ &180641225r^4t^{10} + 119871384r^3t^{11} + 36619498r^2t^{12} + 4605495rt^{13} + 177048t^{14} + 4760r^9t^4 + 278278r^8t^5 + \\ &5188915r^7t^6 + 41000622r^6t^7 + 151799532r^5t^8 + 272864112r^4t^9 + 237500090r^3t^{10} + 96108204r^2t^{11} + \\ &16285593rt^{12} + 868478t^{13} + 1360r^9t^3 + 110348r^8t^4 + 2766954r^7t^5 + 28898418r^6t^6 + 140185306r^5t^7 + \\ &328975930r^4t^8 + 373890368r^3t^9 + 198351034r^2t^{10} + 44457254rt^{11} + 3187250t^{12} + 272r^9t^2 + 32482r^8t^3 + \\ &1133006r^7t^4 + 15960212r^6t^5 + 102642729r^5t^6 + 316324390r^4t^7 + 469894193r^3t^8 + 325496542r^2t^9 + \\ &95546900rt^{10} + 9044796t^{11} + 34r^9t + 6688r^8t^2 + 344012r^7t^3 + 6760153r^6t^4 + 58825220r^5t^5 + 241007787r^4t^6 + \\ &470973223r^3t^7 + 426633918r^2t^8 + 163435575rt^9 + 20235840t^{10} + 2r^9 + 860r^8t + 72976r^7t^2 + 2120112r^6t^3 + \\ &25820158r^5t^4 + 143594604r^4t^5 + 373934139r^3t^6 + 446108022r^2t^7 + 223468308rt^8 + 36075132t^9 + 52r^8 + \\ &9656r^7t + 463788r^6t^2 + 8377308r^5t^3 + 65438517r^4t^4 + 232019454r^3t^5 + 369537102r^2t^6 + 243912546rt^7 + \\ &51460191t^8 + 600r^7 + 63168r^6t + 1891944r^5t^2 + 22003380r^4t^3 + 109990818r^3t^4 + 239161248r^2t^5 + \\ &210998169rt^6 + 58650588t^7 + 4032r^6 + 265356r^5t + 5137236r^4t^2 + 38403396r^3t^3 + 118164771r^2t^4 + \\ &142629660rt^5 + 53020413t^6 + 17388r^5 + 742392r^4t + 9284544r^3t^2 + 42931296r^2t^3 + 73581210rt^4 + \\ &37477242t^5 + 49896r^4 + 1383480r^3t + 10768788r^2t^2 + 27879876rt^3 + 20221731t^4 + 95256r^3 + 1656288r^2t + \\ &7272504rt^2 + 8008794t^3 + 116640r^2 + 1156194rt + 2178252t^2 + 83106r + 358668t + 26244)(t + 1). \end{aligned}$$

$$\tilde{S}_C|_{q=2} = 2(3t^6 + 14t^5 + 33t^4 + 48t^3 + 41t^2 + 18t + 2)(t + 2)^8(t + 1).$$

$$\begin{aligned} D_C^U &= (4s^4t^8 + 32s^4t^7 + 22s^3t^8 + 112s^4t^6 + 195s^3t^7 + 44s^2t^8 + 224s^4t^5 + 753s^3t^6 + 436s^2t^7 + 38st^8 + 280s^4t^4 + \\ &1658s^3t^5 + 1859s^2t^6 + 423st^7 + 12t^8 + 224s^4t^3 + 2280s^3t^4 + 4496s^2t^5 + 1989st^6 + 150t^7 + 112s^4t^2 + \\ &2007s^3t^3 + 6790s^2t^4 + 5272st^5 + 774t^6 + 32s^4t + 1105s^3t^2 + 6584s^2t^3 + 8734st^4 + 2240t^5 + 4s^4 + 348s^3t + \\ &4011s^2t^2 + 9341st^3 + 4068t^4 + 48s^3 + 1404s^2t + 6327st^2 + 4812t^3 + 216s^2 + 2484st + 3645t^2 + 432s + \\ &1620t + 324)(st^2 + 2st + t^2 + s + 2t + 2)(s + 3)(t + 1). \end{aligned}$$

$$D_C^U|_{q=2} = 2(3t^2 + 6t + 4)(t + 2)^4(t + 1).$$

Local view 28 of 35.

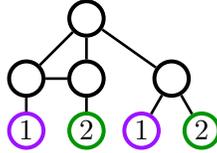

$$\begin{aligned} Z_C &= 2\lambda^6 + 4\lambda^5 + 7\lambda^4(q - 2) + \lambda^3(q - 2)(q - 3) + 4\lambda^4 + 25\lambda^3(q - 2) + 24\lambda^2(q - 2)(q - 3) + \\ &8\lambda(q - 2)(q - 3)(q - 4) + (q - 2)(q - 3)(q - 4)(q - 5) + 4\lambda^3 + 18\lambda^2(q - 2) + 21\lambda(q - 2)(q - 3) + \\ &6(q - 2)(q - 3)(q - 4) + 2\lambda^2 + 13\lambda(q - 2) + 9(q - 2)(q - 3) + 2q - 4. \end{aligned}$$

$$\begin{aligned} 2Z_C U_C^v &= 6\lambda^6 + 8\lambda^5 + 15\lambda^4(q - 2) + 2\lambda^3(q - 2)(q - 3) + 4\lambda^4 + 23\lambda^3(q - 2) + 17\lambda^2(q - 2)(q - 3) + \\ &3\lambda(q - 2)(q - 3)(q - 4) + 4\lambda^3 + 14\lambda^2(q - 2) + 8\lambda(q - 2)(q - 3) + 2\lambda^2 + 5\lambda(q - 2). \end{aligned}$$

$$\begin{aligned} 6Z_C U_C^N &= 14\lambda^6 + 22\lambda^5 + 33\lambda^4(q - 2) + 4\lambda^3(q - 2)(q - 3) + 18\lambda^4 + 83\lambda^3(q - 2) + 53\lambda^2(q - 2)(q - 3) + \\ &9\lambda(q - 2)(q - 3)(q - 4) + 14\lambda^3 + 40\lambda^2(q - 2) + 24\lambda(q - 2)(q - 3) + 4\lambda^2 + 15\lambda(q - 2). \end{aligned}$$

$$\begin{aligned} \tilde{S}_C &= 2(2r^9t^{14} + 28r^9t^{13} + 26r^8t^{14} + 182r^9t^{12} + 386r^8t^{13} + 150r^7t^{14} + 728r^9t^{11} + 2656r^8t^{12} + 2356r^7t^{13} + \\ & 503r^6t^{14} + 2002r^9t^{10} + 11228r^8t^{11} + 17132r^7t^{12} + 8349r^6t^{13} + 1082r^5t^{14} + 4004r^9t^9 + 32582r^8t^{10} + \\ & 76452r^7t^{11} + 64091r^6t^{12} + 18948r^5t^{13} + 1555r^4t^{14} + 6006r^9t^8 + 68662r^8t^9 + 233930r^7t^{10} + 301645r^6t^{11} + \\ & 153338r^5t^{12} + 28627r^4t^{13} + 1501r^3t^{14} + 6864r^9t^7 + 108372r^8t^8 + 519240r^7t^9 + 972583r^6t^{10} + 760298r^5t^{11} + \\ & 243619r^4t^{12} + 28877r^3t^{13} + 942r^2t^{14} + 6006r^9t^6 + 130152r^8t^7 + 862272r^7t^8 + 2272875r^6t^9 + 2581016r^5t^{10} + \\ & 1270386r^4t^{11} + 257436r^3t^{12} + 18801r^2t^{13} + 349rt^{14} + 4004r^9t^5 + 119526r^8t^6 + 1088424r^7t^7 + 3970673r^6t^8 + \\ & 6347086r^5t^9 + 4535361r^4t^{10} + 1408325r^3t^{11} + 174724r^2t^{12} + 7178rt^{13} + 58t^{14} + 2002r^9t^4 + 83534r^8t^5 + \\ & 1049514r^7t^6 + 5268479r^6t^7 + 11661826r^5t^8 + 11727539r^4t^9 + 5278986r^3t^{10} + 999565r^2t^{11} + 69174rt^{12} + \\ & 1224t^{13} + 728r^9t^3 + 43736r^8t^4 + 769380r^7t^5 + 5335860r^6t^6 + 16265434r^5t^7 + 22653365r^4t^8 + 14339118r^3t^9 + \\ & 3926007r^2t^{10} + 412337rt^{11} + 12172t^{12} + 182r^9t^2 + 16636r^8t^3 + 422140r^7t^4 + 4105380r^6t^5 + 17307668r^5t^6 + \\ & 33210656r^4t^7 + 29103325r^3t^8 + 11188194r^2t^9 + 1693081rt^{10} + 75318t^{11} + 28r^9t + 4346r^8t^2 + 168116r^7t^3 + \\ & 2362312r^6t^4 + 13983454r^5t^5 + 37136434r^4t^6 + 44838724r^3t^7 + 23843502r^2t^8 + 5054880r^9 + 322518t^{10} + \\ & 2r^9 + 698r^8t + 45942r^7t^2 + 985904r^6t^3 + 8444864r^5t^4 + 31522428r^4t^5 + 52697454r^3t^6 + 38594097r^2t^7 + \\ & 11302191rt^8 + 1007352t^9 + 52r^8 + 7712r^7t + 282138r^6t^2 + 3696948r^5t^3 + 19994868r^4t^4 + 47016732r^3t^5 + \\ & 47675988r^2t^6 + 19212930rt^7 + 2361150t^8 + 600r^7 + 49560r^6t + 1109106r^5t^2 + 9190584r^4t^3 + 31347252r^3t^4 + \\ & 44728416r^2t^5 + 24946542rt^6 + 4213728t^7 + 4032r^6 + 204120r^5t + 2893806r^4t^2 + 15143868r^3t^3 + \\ & 31369248r^2t^4 + 24618654rt^5 + 5750352t^6 + 17388r^5 + 558684r^4t + 5010498r^3t^2 + 15944688r^2t^3 + \\ & 18174942rt^4 + 5970834t^5 + 49896r^4 + 1016064r^3t + 5550606r^2t^2 + 9730692rt^3 + 4643244t^4 + 95256r^3 + \\ & 1183896r^2t + 3569184rt^2 + 2621484t^3 + 116640r^2 + 801900rt + 1014768t^2 + 83106r + 240570t + 26244)(t+1)^4. \end{aligned}$$

$$\tilde{S}_C|_{q=2} = 4(t^3 + 2t^2 + 3t + 1)(t + 2)^8(t + 1)^4.$$

$$\begin{aligned} D_C^U &= (4s^5t^8 + 32s^5t^7 + 26s^4t^8 + 112s^5t^6 + 229s^4t^7 + 66s^3t^8 + 224s^5t^5 + 881s^4t^6 + 640s^3t^7 + 82s^2t^8 + 280s^5t^4 + \\ & 1936s^4t^5 + 2699s^3t^6 + 872s^2t^7 + 50st^8 + 224s^5t^3 + 2660s^4t^4 + 6496s^3t^5 + 4015s^2t^6 + 579st^7 + 12t^8 + 112s^5t^2 + \\ & 2341s^4t^3 + 9796s^3t^4 + 10551s^2t^5 + 2895st^6 + 150t^7 + 32s^5t + 1289s^4t^2 + 9500s^3t^3 + 17430s^2t^4 + 8277st^5 + \\ & 810t^6 + 4s^5 + 406s^4t + 5791s^3t^2 + 18639s^2t^3 + 14942st^4 + 2510t^5 + 56s^4 + 2028s^3t + 12639s^2t^2 + 17608st^3 + \\ & 4932t^4 + 312s^3 + 4968s^2t + 13329st^2 + 6384t^3 + 864s^2 + 5940st + 5400t^2 + 1188s + 2754t + 648)(s + 3)(t + 1)^3. \end{aligned}$$

$$D_C^U|_{q=2} = 8(t + 2)^4(t + 1)^3.$$

Local view 29 of 35.

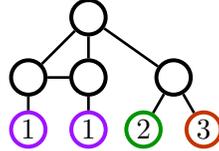

$$\begin{aligned} Z_C &= 3\lambda^6 + \lambda^5(q - 3) + 4\lambda^5 + 6\lambda^4(q - 3) + 2\lambda^3(q - 3)(q - 4) + 8\lambda^4 + 28\lambda^3(q - 3) + 21\lambda^2(q - 3)(q - 4) + \\ & 8\lambda(q - 3)(q - 4)(q - 5) + (q - 3)(q - 4)(q - 5)(q - 6) + 30\lambda^3 + 59\lambda^2(q - 3) + 48\lambda(q - 3)(q - 4) + \\ & 10(q - 3)(q - 4)(q - 5) + 20\lambda^2 + 65\lambda(q - 3) + 26(q - 3)(q - 4) + 16\lambda + 16q - 48. \end{aligned}$$

$$\begin{aligned} 2Z_C U_C^v &= 7\lambda^6 + 2\lambda^5(q - 3) + 8\lambda^5 + 8\lambda^4(q - 3) + 2\lambda^3(q - 3)(q - 4) + 12\lambda^4 + 36\lambda^3(q - 3) + 17\lambda^2(q - 3)(q - 4) + \\ & 3\lambda(q - 3)(q - 4)(q - 5) + 38\lambda^3 + 43\lambda^2(q - 3) + 17\lambda(q - 3)(q - 4) + 10\lambda^2 + 22\lambda(q - 3) + 6\lambda. \end{aligned}$$

$$\begin{aligned} 6Z_C U_C^N &= 21\lambda^6 + 6\lambda^5(q - 3) + 24\lambda^5 + 30\lambda^4(q - 3) + 8\lambda^3(q - 3)(q - 4) + 36\lambda^4 + 92\lambda^3(q - 3) + 45\lambda^2(q - 3)(q - 4) + \\ & 9\lambda(q - 3)(q - 4)(q - 5) + 96\lambda^3 + 129\lambda^2(q - 3) + 55\lambda(q - 3)(q - 4) + 48\lambda^2 + 76\lambda(q - 3) + 18\lambda. \end{aligned}$$

$$\begin{aligned}
\tilde{S}_C &= 2(2r^9t^{16} + 32r^9t^{15} + 30r^8t^{16} + 240r^9t^{14} + 496r^8t^{15} + 190r^7t^{16} + 1120r^9t^{13} + 3846r^8t^{14} + 3272r^7t^{15} + 679r^6t^{16} + \\
&3640r^9t^{12} + 18564r^8t^{13} + 26410r^7t^{14} + 12221r^6t^{15} + 1527r^5t^{16} + 8736r^9t^{11} + 62426r^8t^{12} + 132624r^7t^{13} + \\
&102994r^6t^{14} + 28740r^5t^{15} + 2259r^4t^{16} + 16016r^9t^{10} + 155064r^8t^{11} + 463766r^7t^{12} + 539596r^6t^{13} + \\
&253080r^5t^{14} + 44405r^4t^{15} + 2210r^3t^{16} + 22880r^9t^9 + 294294r^8t^{10} + 1197400r^7t^{11} + 1967252r^6t^{12} + \\
&1384544r^5t^{13} + 408290r^4t^{14} + 45262r^3t^{15} + 1385r^2t^{16} + 25740r^9t^8 + 435292r^8t^9 + 2361194r^7t^{10} + \\
&5292570r^6t^{11} + 5268304r^5t^{12} + 2331773r^4t^{13} + 433889r^3t^{14} + 29438r^2t^{15} + 508rt^{16} + 22880r^9t^7 + \\
&507078r^8t^8 + 3627360r^7t^9 + 10869330r^6t^{10} + 14786648r^5t^{11} + 9260658r^4t^{12} + 2584320r^3t^{13} + 293553r^2t^{14} + \\
&11122rt^{15} + 84t^{16} + 16016r^9t^6 + 466752r^8t^7 + 4387218r^7t^8 + 17381892r^6t^9 + 31669522r^5t^{10} + 27125551r^4t^{11} + \\
&10706419r^3t^{12} + 1820973r^2t^{13} + 114948rt^{14} + 1868t^{15} + 8736r^9t^5 + 338338r^8t^6 + 4191352r^7t^7 + \\
&21873963r^6t^8 + 52798808r^5t^9 + 60625090r^4t^{10} + 32719790r^3t^{11} + 7862259r^2t^{12} + 741213rt^{13} + 19884t^{14} + \\
&3640r^9t^4 + 191100r^8t^5 + 3152270r^7t^6 + 21732973r^6t^7 + 69245503r^5t^8 + 105464877r^4t^9 + 76315475r^3t^{10} + \\
&25054353r^2t^{11} + 3331527rt^{12} + 132918t^{13} + 1120r^9t^3 + 82446r^8t^4 + 1846672r^7t^5 + 16990394r^6t^6 + \\
&71672540r^5t^7 + 144314633r^4t^8 + 138581496r^3t^9 + 60964129r^2t^{10} + 11061474rt^{11} + 621114t^{12} + 240r^9t^2 + \\
&26264r^8t^3 + 826050r^7t^4 + 10341016r^6t^5 + 58346176r^5t^6 + 155827088r^4t^7 + 197993517r^3t^8 + 115556569r^2t^9 + \\
&28064376rt^{10} + 2146944t^{11} + 32r^9t + 5826r^8t^2 + 272744r^7t^3 + 4803298r^6t^4 + 36958760r^5t^5 + 132301778r^4t^6 + \\
&223259032r^3t^7 + 172433508r^2t^8 + 55509378rt^9 + 5675940t^{10} + 2r^9 + 804r^8t + 62686r^7t^2 + 1645892r^6t^3 + \\
&17855238r^5t^4 + 87369846r^4t^5 + 197965242r^3t^6 + 203193063r^2t^7 + 86509998rt^8 + 11709072t^9 + 52r^8 + \\
&8960r^7t + 392346r^6t^2 + 6358824r^5t^3 + 43978902r^4t^4 + 136518204r^3t^5 + 188376498r^2t^6 + 106570620rt^7 + \\
&19053252t^8 + 600r^7 + 58128r^6t + 1574046r^5t^2 + 16305300r^4t^3 + 71730702r^3t^4 + 135859680r^2t^5 + \\
&103381704rt^6 + 24537924t^7 + 4032r^6 + 241920r^5t + 4197150r^4t^2 + 27738072r^3t^3 + 74652678r^2t^4 + \\
&78079788rt^5 + 24919488t^6 + 17388r^5 + 669816r^4t + 7437258r^3t^2 + 30171852r^2t^3 + 44949330rt^4 + \\
&19729494t^5 + 49896r^4 + 1233792r^3t + 8443278r^2t^2 + 19029816rt^3 + 11919636t^4 + 95256r^3 + 1458000r^2t + \\
&5571018rt^2 + 5298372t^3 + 116640r^2 + 1003104rt + 1627128t^2 + 83106r + 306180t + 26244)(t + 1)^2. \\
D_C^U &= (4s^4t^8 + 32s^4t^7 + 22s^3t^8 + 112s^4t^6 + 195s^3t^7 + 44s^2t^8 + 224s^4t^5 + 753s^3t^6 + 436s^2t^7 + 38st^8 + 280s^4t^4 + 1658s^3t^5 + \\
&1859s^2t^6 + 423st^7 + 12t^8 + 224s^4t^3 + 2280s^3t^4 + 4496s^2t^5 + 1989st^6 + 150t^7 + 112s^4t^2 + 2007s^3t^3 + 6790s^2t^4 + \\
&5272st^5 + 774t^6 + 32s^4t + 1105s^3t^2 + 6584s^2t^3 + 8734st^4 + 2240t^5 + 4s^4 + 348s^3t + 4011s^2t^2 + 9341st^3 + 4068t^4 + \\
&48s^3 + 1404s^2t + 6327st^2 + 4812t^3 + 216s^2 + 2484st + 3645t^2 + 432s + 1620t + 324)(st + s + 2)(s + 3)(t + 1)^2.
\end{aligned}$$

Local view 30 of 35.

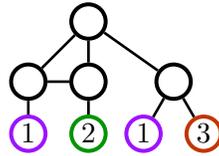

$$\begin{aligned}
Z_C &= \lambda^6 + 6\lambda^5 + 6\lambda^4(q-3) + \lambda^3(q-3)(q-4) + 13\lambda^4 + 31\lambda^3(q-3) + 24\lambda^2(q-3)(q-4) + \\
&8\lambda(q-3)(q-4)(q-5) + (q-3)(q-4)(q-5)(q-6) + 21\lambda^3 + 60\lambda^2(q-3) + 45\lambda(q-3)(q-4) + \\
&10(q-3)(q-4)(q-5) + 27\lambda^2 + 59\lambda(q-3) + 27(q-3)(q-4) + 11\lambda + 19q - 55. \\
2Z_C U_C^v &= 3\lambda^6 + 14\lambda^5 + 13\lambda^4(q-3) + 2\lambda^3(q-3)(q-4) + 19\lambda^4 + 33\lambda^3(q-3) + 17\lambda^2(q-3)(q-4) + \\
&3\lambda(q-3)(q-4)(q-5) + 21\lambda^3 + 42\lambda^2(q-3) + 17\lambda(q-3)(q-4) + 19\lambda^2 + 23\lambda(q-3) + 5\lambda. \\
6Z_C U_C^N &= 7\lambda^6 + 35\lambda^5 + 29\lambda^4(q-3) + 4\lambda^3(q-3)(q-4) + 57\lambda^4 + 103\lambda^3(q-3) + 53\lambda^2(q-3)(q-4) + \\
&9\lambda(q-3)(q-4)(q-5) + 71\lambda^3 + 134\lambda^2(q-3) + 51\lambda(q-3)(q-4) + 61\lambda^2 + 67\lambda(q-3) + 12\lambda.
\end{aligned}$$

$$\begin{aligned}
 \tilde{S}_C &= (4r^8t^{14} + 56r^8t^{13} + 48r^7t^{14} + 364r^8t^{12} + 708r^7t^{13} + 242r^6t^{14} + 1456r^8t^{11} + 4844r^7t^{12} + 3786r^6t^{13} + \\
 &678r^5t^{14} + 4004r^8t^{10} + 20376r^7t^{11} + 27422r^6t^{12} + 11284r^5t^{13} + 1166r^4t^{14} + 8008r^8t^9 + 58872r^7t^{10} + \\
 &121894r^6t^{11} + 86746r^5t^{12} + 20640r^4t^{13} + 1267r^3t^{14} + 12012r^8t^8 + 123596r^7t^9 + 371544r^6t^{10} + 408452r^5t^{11} + \\
 &168452r^4t^{12} + 23817r^3t^{13} + 849r^2t^{14} + 13728r^8t^7 + 194436r^7t^8 + 821604r^6t^9 + 1316462r^5t^{10} + 840728r^4t^{11} + \\
 &206198r^3t^{12} + 16940r^2t^{13} + 320rt^{14} + 12012r^8t^6 + 232848r^7t^7 + 1359432r^6t^8 + 3073206r^5t^9 + 2868048r^4t^{10} + \\
 &1090508r^3t^{11} + 155508r^2t^{12} + 6779rt^{13} + 52t^{14} + 8008r^8t^5 + 213312r^7t^6 + 1709964r^6t^7 + 5359846r^5t^8 + \\
 &7077040r^4t^9 + 3938135r^3t^{10} + 871224r^2t^{11} + 66006rt^{12} + 1166t^{13} + 4004r^8t^4 + 148764r^7t^5 + 1643298r^6t^6 + \\
 &7096018r^5t^7 + 13029736r^4t^8 + 10277361r^3t^9 + 3330281r^2t^{10} + 391838rt^{11} + 12044t^{12} + 1456r^8t^3 + \\
 &77748r^7t^4 + 1200818r^6t^5 + 7167552r^5t^6 + 18187392r^4t^7 + 19994068r^3t^8 + 9193464r^2t^9 + 1585738rt^{10} + \\
 &75836t^{11} + 364r^8t^2 + 29528r^7t^3 + 656862r^6t^4 + 5497634r^5t^5 + 19343858r^4t^6 + 29463014r^3t^7 + 18908970r^2t^8 + \\
 &4631567rt^9 + 325224t^{10} + 56r^8t + 7704r^7t^2 + 260846r^6t^3 + 3152508r^5t^4 + 15602488r^4t^5 + 33049912r^3t^6 + \\
 &29443716r^2t^7 + 10074894rt^8 + 1005702t^9 + 4r^8 + 1236r^7t + 71092r^6t^2 + 1310722r^5t^3 + 9395664r^4t^4 + \\
 &28084716r^3t^5 + 34881678r^2t^6 + 16588062rt^7 + 2314836t^8 + 92r^7 + 11904r^6t + 373572r^5t^2 + 4096536r^4t^3 + \\
 &17795280r^3t^4 + 31283154r^2t^5 + 20776716rt^6 + 4032126t^7 + 924r^6 + 65340r^5t + 1222560r^4t^2 + 8151660r^3t^3 + \\
 &20899890r^2t^4 + 19696446rt^5 + 5343678t^6 + 5292r^5 + 223560r^4t + 2551392r^3t^2 + 10080558r^2t^3 + 13903488rt^4 + \\
 &5361876t^5 + 18900r^4 + 488268r^3t + 3315492r^2t^2 + 7078266rt^3 + 4006908t^4 + 43092r^3 + 664848r^2t + \\
 &2452356t^2 + 2158812t^3 + 61236r^2 + 516132rt + 790236t^2 + 49572r + 174960t + 17496)(rt + r + 2t + 3)(t + 1)^3. \\
 D_C^U &= (4s^5t^8 + 32s^5t^7 + 24s^4t^8 + 112s^5t^6 + 215s^4t^7 + 57s^3t^8 + 224s^5t^5 + 839s^4t^6 + 565s^3t^7 + 69s^2t^8 + 280s^5t^4 + \\
 &1866s^4t^5 + 2435s^3t^6 + 736s^2t^7 + 44st^8 + 224s^5t^3 + 2590s^4t^4 + 5986s^3t^5 + 3439s^2t^6 + 489st^7 + 12t^8 + 112s^5t^2 + \\
 &2299s^4t^3 + 9211s^3t^4 + 9239s^2t^5 + 2406st^6 + 138t^7 + 32s^5t + 1275s^4t^2 + 9101s^3t^3 + 15677s^2t^4 + 6905st^5 + \\
 &696t^6 + 4s^5 + 404s^4t + 5641s^3t^2 + 17259s^2t^3 + 12742st^4 + 2054t^5 + 56s^4 + 2004s^3t + 12045s^2t^2 + 15565st^3 + \\
 &3984t^4 + 312s^3 + 4860s^2t + 12303st^2 + 5304t^3 + 864s^2 + 5724st + 4752t^2 + 1188s + 2592t + 648)(s + 3)(t + 1)^3.
 \end{aligned}$$

Local view 31 of 35.

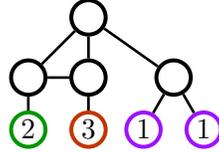

$$\begin{aligned}
 Z_C &= 3\lambda^6 + \lambda^5(q-3) + 9\lambda^5 + 15\lambda^4(q-3) + 7\lambda^3(q-3)(q-4) + \lambda^2(q-3)(q-4)(q-5) + 10\lambda^4 + 27\lambda^3(q-3) + \\
 &18\lambda^2(q-3)(q-4) + 6\lambda(q-3)(q-4)(q-5) + (q-3)(q-4)(q-5)(q-6) + 17\lambda^3 + 45\lambda^2(q-3) + \\
 &39\lambda(q-3)(q-4) + 11(q-3)(q-4)(q-5) + 24\lambda^2 + 60\lambda(q-3) + 33(q-3)(q-4) + 14\lambda + 27q - 77. \\
 2Z_C U_C^V &= 7\lambda^6 + 2\lambda^5(q-3) + 15\lambda^5 + 18\lambda^4(q-3) + 5\lambda^3(q-3)(q-4) + 14\lambda^4 + 27\lambda^3(q-3) + 11\lambda^2(q-3)(q-4) + \\
 &3\lambda(q-3)(q-4)(q-5) + 17\lambda^3 + 31\lambda^2(q-3) + 20\lambda(q-3)(q-4) + 18\lambda^2 + 33\lambda(q-3) + 10\lambda. \\
 6Z_C U_C^N &= 21\lambda^6 + 6\lambda^5(q-3) + 49\lambda^5 + 66\lambda^4(q-3) + 23\lambda^3(q-3)(q-4) + 2\lambda^2(q-3)(q-4)(q-5) + 44\lambda^4 + \\
 &89\lambda^3(q-3) + 39\lambda^2(q-3)(q-4) + 7\lambda(q-3)(q-4)(q-5) + 57\lambda^3 + 101\lambda^2(q-3) + 46\lambda(q-3)(q-4) + \\
 &56\lambda^2 + 71\lambda(q-3) + 16\lambda.
 \end{aligned}$$

$$\begin{aligned}
\tilde{S}_C &= 2(2r^9t^{16} + 32r^9t^{15} + 30r^8t^{16} + 240r^9t^{14} + 500r^8t^{15} + 191r^7t^{16} + 1120r^9t^{13} + 3904r^8t^{14} + 3330r^7t^{15} + 686r^6t^{16} + \\
&3640r^9t^{12} + 18954r^8t^{13} + 27187r^7t^{14} + 12548r^6t^{15} + 1546r^5t^{16} + 8736r^9t^{11} + 64038r^8t^{12} + 137928r^7t^{13} + \\
&107398r^6t^{14} + 29719r^5t^{15} + 2284r^4t^{16} + 16016r^9t^{10} + 159640r^8t^{11} + 486558r^7t^{12} + 570750r^6t^{13} + \\
&267015r^5t^{14} + 46164r^4t^{15} + 2228r^3t^{16} + 22880r^9t^9 + 303732r^8t^{10} + 1265216r^7t^{11} + 2107256r^6t^{12} + \\
&1488160r^5t^{13} + 435527r^4t^{14} + 47289r^3t^{15} + 1397r^2t^{16} + 25740r^9t^8 + 449878r^8t^9 + 2508230r^7t^{10} + \\
&5729730r^6t^{11} + 5757222r^5t^{12} + 2546224r^4t^{13} + 468068r^3t^{14} + 30988r^2t^{15} + 518rt^{16} + 22880r^9t^7 + \\
&524238r^8t^8 + 3866424r^7t^9 + 11865360r^6t^{10} + 16389450r^5t^{11} + 10324641r^4t^{12} + 2868751r^3t^{13} + 320902r^2t^{14} + \\
&11874rt^{15} + 88t^{16} + 16016r^9t^6 + 482196r^8t^7 + 4683051r^7t^8 + 19084404r^6t^9 + 35504178r^5t^{10} + 30785410r^4t^{11} + \\
&12187312r^3t^{12} + 2058396r^2t^{13} + 127874rt^{14} + 2044t^{15} + 8736r^9t^5 + 348920r^8t^6 + 4471226r^7t^7 + \\
&24088782r^6t^8 + 59682900r^5t^9 + 69808403r^4t^{10} + 38054727r^3t^{11} + 9152010r^2t^{12} + 855668rt^{13} + 22652t^{14} + \\
&3640r^9t^4 + 196534r^8t^5 + 3353679r^7t^6 + 23935160r^6t^7 + 78652998r^5t^8 + 122758494r^4t^9 + 90331359r^3t^{10} + \\
&29905312r^2t^{11} + 3974529rt^{12} + 157296t^{13} + 1120r^9t^3 + 84474r^8t^4 + 1955200r^7t^5 + 18655334r^6t^6 + \\
&81499663r^5t^7 + 169115669r^4t^8 + 166228537r^3t^9 + 74280460r^2t^{10} + 13576423rt^{11} + 761354t^{12} + 240r^9t^2 + \\
&26784r^8t^3 + 868512r^7t^4 + 11283094r^6t^5 + 66152431r^5t^6 + 183029936r^4t^7 + 239556490r^3t^8 + 143028836r^2t^9 + \\
&35262818rt^{10} + 2715174t^{11} + 32r^9t + 5908r^8t^2 + 284148r^7t^3 + 5190156r^6t^4 + 41599812r^5t^5 + 155004162r^4t^6 + \\
&271093024r^3t^7 + 215677563r^2t^8 + 71020089rt^9 + 7369116t^{10} + 2r^9 + 810r^8t + 64568r^7t^2 + 1754882r^6t^3 + \\
&19857670r^5t^4 + 101558130r^4t^5 + 239896251r^3t^6 + 255372768r^2t^7 + 112047975rt^8 + 15516234t^9 + 52r^8 + \\
&9104r^7t + 411204r^6t^2 + 6951528r^5t^3 + 50417382r^4t^4 + 164074044r^3t^5 + 236403936r^2t^6 + 138853683rt^7 + \\
&25605288t^8 + 600r^7 + 59640r^6t + 1681776r^5t^2 + 18310590r^4t^3 + 84894156r^3t^4 + 169053750r^2t^5 + \\
&134568351rt^6 + 33209784t^7 + 4032r^6 + 250992r^5t + 4580820r^4t^2 + 32058612r^3t^3 + 91358064r^2t^4 + \\
&100749744rt^5 + 33708312t^6 + 17388r^5 + 703836r^4t + 8309304r^3t^2 + 35958654r^2t^3 + 56976534rt^4 + \\
&26448444t^5 + 49896r^4 + 1315440r^3t + 9678204r^2t^2 + 23432976rt^3 + 15679332t^4 + 95256r^3 + 1580472r^2t + \\
&6566832rt^2 + 6754914t^3 + 116640r^2 + 1108080rt + 1977048t^2 + 83106r + 345546t + 26244)(t + 1)^2. \\
D_C^U &= (4s^5t^9 + 36s^5t^8 + 26s^4t^9 + 144s^5t^7 + 251s^4t^8 + 70s^3t^9 + 336s^5t^6 + 1082s^4t^7 + 709s^3t^8 + 100s^2t^9 + \\
&504s^5t^5 + 2733s^4t^6 + 3231s^3t^7 + 1033s^2t^8 + 76st^9 + 504s^5t^4 + 4456s^4t^5 + 8705s^3t^6 + 4852s^2t^7 + 788st^8 + \\
&24t^9 + 336s^5t^3 + 4861s^4t^4 + 15284s^3t^5 + 13657s^2t^6 + 3732st^7 + 252t^8 + 144s^5t^2 + 3546s^4t^3 + 18123s^3t^4 + \\
&25444s^2t^5 + 10703st^6 + 1200t^7 + 36s^5t + 1667s^4t^2 + 14491s^3t^3 + 32539s^2t^4 + 20682st^5 + 3442t^6 + 4s^5 + \\
&458s^4t + 7519s^3t^2 + 28500s^2t^3 + 28087st^4 + 6692t^5 + 56s^4 + 2292s^3t + 16419s^2t^2 + 26797st^3 + 9366t^4 + \\
&312s^3 + 5616s^2t + 17217st^2 + 9570t^3 + 864s^2 + 6696st + 6858t^2 + 1188s + 3078t + 648)(s + 3)(t + 1)^2.
\end{aligned}$$

Local view 32 of 35.

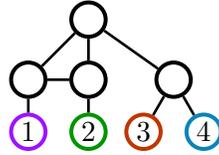

$$\begin{aligned}
Z_C &= 8\lambda^5 + 5\lambda^4(q-4) + \lambda^3(q-4)(q-5) + 20\lambda^4 + 37\lambda^3(q-4) + 24\lambda^2(q-4)(q-5) + 8\lambda(q-4)(q-5)(q-6) + \\
&(q-4)(q-5)(q-6)(q-7) + 48\lambda^3 + 102\lambda^2(q-4) + 69\lambda(q-4)(q-5) + 14(q-4)(q-5)(q-6) + 88\lambda^2 + \\
&153\lambda(q-4) + 57(q-4)(q-5) + 72\lambda + 72q - 268. \\
2Z_C U_C^v &= 20\lambda^5 + 11\lambda^4(q-4) + 2\lambda^3(q-4)(q-5) + 30\lambda^4 + 43\lambda^3(q-4) + 17\lambda^2(q-4)(q-5) + \\
&3\lambda(q-4)(q-5)(q-6) + 54\lambda^3 + 70\lambda^2(q-4) + 26\lambda(q-4)(q-5) + 58\lambda^2 + 59\lambda(q-4) + 30\lambda. \\
6Z_C U_C^N &= 48\lambda^5 + 25\lambda^4(q-4) + 4\lambda^3(q-4)(q-5) + 88\lambda^4 + 123\lambda^3(q-4) + 53\lambda^2(q-4)(q-5) + \\
&9\lambda(q-4)(q-5)(q-6) + 160\lambda^3 + 228\lambda^2(q-4) + 78\lambda(q-4)(q-5) + 200\lambda^2 + 173\lambda(q-4) + 80\lambda.
\end{aligned}$$

$$\begin{aligned}
 \tilde{S}_C &= 2(2r^9t^{15} + 30r^9t^{14} + 30r^8t^{15} + 210r^9t^{13} + 468r^8t^{14} + 188r^7t^{15} + 910r^9t^{12} + 3406r^8t^{13} + 3082r^7t^{14} + 659r^6t^{15} + \\
 & 2730r^9t^{11} + 15340r^8t^{12} + 23532r^7t^{13} + 11408r^6t^{14} + 1440r^5t^{15} + 6006r^9t^{10} + 47814r^8t^{11} + 111016r^7t^{12} + \\
 & 91792r^6t^{13} + 26378r^5t^{14} + 2044r^4t^{15} + 10010r^9t^9 + 109252r^8t^{10} + 361928r^7t^{11} + 455516r^6t^{12} + \\
 & 224150r^5t^{13} + 39680r^4t^{14} + 1882r^3t^{15} + 12870r^9t^8 + 189046r^8t^9 + 863786r^7t^{10} + 1559456r^6t^{11} + \\
 & 1172686r^5t^{12} + 356593r^4t^{13} + 38846r^3t^{14} + 1076r^2t^{15} + 12870r^9t^7 + 252252r^8t^8 + 1559184r^7t^9 + \\
 & 3902050r^6t^{10} + 4225742r^5t^{11} + 1969513r^4t^{12} + 369982r^3t^{13} + 23783r^2t^{14} + 343rt^{15} + 10010r^9t^6 + \\
 & 261690r^8t^7 + 2167704r^7t^8 + 7373180r^6t^9 + 11112784r^5t^{10} + 7481176r^4t^{11} + 2160581r^3t^{12} + 241096r^2t^{13} + \\
 & 8209r^{14} + 46t^{15} + 6006r^9t^5 + 211068r^8t^6 + 2340492r^7t^7 + 10714936r^6t^8 + 22037174r^5t^9 + 20710820r^4t^{10} + \\
 & 8661988r^3t^{11} + 1492527r^2t^{12} + 89207rt^{13} + 1206t^{14} + 2730r^9t^4 + 131274r^8t^5 + 1962686r^7t^6 + 12075719r^6t^7 + \\
 & 33561442r^5t^8 + 43181117r^4t^9 + 25274768r^3t^{10} + 6326238r^2t^{11} + 588063rt^{12} + 14190t^{13} + 910r^9t^3 + \\
 & 61828r^8t^4 + 1267948r^7t^5 + 10555476r^6t^6 + 39581306r^5t^7 + 69057053r^4t^8 + 55480210r^3t^9 + 19480875r^2t^{10} + \\
 & 2642632rt^{11} + 100314t^{12} + 210r^9t^2 + 21346r^8t^3 + 619752r^7t^4 + 7098628r^6t^5 + 36153148r^5t^6 + 85415728r^4t^7 + \\
 & 93318869r^3t^8 + 45073097r^2t^9 + 8603313rt^{10} + 480120t^{11} + 30r^9t + 5100r^8t^2 + 221872r^7t^3 + 3607292r^6t^4 + \\
 & 25367752r^5t^5 + 81712316r^4t^6 + 121278082r^3t^7 + 79839699r^2t^8 + 21007956rt^9 + 1657206t^{10} + 2r^9 + 754r^8t + \\
 & 54926r^7t^2 + 1340974r^6t^3 + 13429356r^5t^4 + 59961492r^4t^5 + 121769814r^3t^6 + 109189197r^2t^7 + 39232647rt^8 + \\
 & 4278276t^9 + 52r^8 + 8408r^7t + 344298r^6t^2 + 5192352r^5t^3 + 33141552r^4t^4 + 93663768r^3t^5 + 115280100r^2t^6 + \\
 & 56533950rt^7 + 8433882t^8 + 600r^7 + 54600r^6t + 1384290r^5t^2 + 13353390r^4t^3 + 54178488r^3t^4 + 93151512r^2t^5 + \\
 & 62863398rt^6 + 12819654t^7 + 4032r^6 + 227556r^5t + 3701970r^4t^2 + 22799448r^3t^3 + 56528604r^2t^4 + \\
 & 53471502rt^5 + 15033600t^6 + 17388r^5 + 631260r^4t + 6584490r^3t^2 + 24907986r^2t^3 + 34127082rt^4 + \\
 & 13485366t^5 + 49896r^4 + 1165752r^3t + 7510158r^2t^2 + 15788682rt^3 + 9073620t^4 + 95256r^3 + 1382184r^2t + \\
 & 4983444rt^2 + 4420656t^3 + 116640r^2 + 954990rt + 1465290t^2 + 83106r + 293058t + 26244)(t + 1)^3. \\
 D_C^U &= (4s^5t^8 + 32s^5t^7 + 42s^4t^8 + 112s^5t^6 + 361s^4t^7 + 176s^3t^8 + 224s^5t^5 + 1357s^4t^6 + 1614s^3t^7 + 372s^2t^8 + \\
 & 280s^5t^4 + 2916s^4t^5 + 6479s^3t^6 + 3596s^2t^7 + 402st^8 + 224s^5t^3 + 3920s^4t^4 + 14900s^3t^5 + 15278s^2t^6 + \\
 & 4033st^7 + 180t^8 + 112s^5t^2 + 3377s^4t^3 + 21506s^3t^4 + 37371s^2t^5 + 17904st^6 + 1848t^7 + 32s^5t + 1821s^4t^2 + \\
 & 19970s^3t^3 + 57722s^2t^4 + 46119st^5 + 8442t^6 + 4s^5 + 562s^4t + 11655s^3t^2 + 57767s^2t^3 + 75748st^4 + \\
 & 22554t^5 + 76s^4 + 3908s^3t + 36610s^2t^2 + 81534st^3 + 38928t^4 + 576s^3 + 13424s^2t + 56256st^2 + 44808t^3 + \\
 & 2176s^2 + 22720st + 33696t^2 + 4096s + 15104t + 3072)(s + 4)(t + 1)^3.
 \end{aligned}$$

Local view 33 of 35.

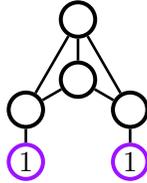

$$\begin{aligned}
 Z_C &= \lambda^7 + \lambda^5(q - 1) + 6\lambda^4(q - 1) + 2\lambda^3(q - 1)(q - 2) + 5\lambda^3(q - 1) + 15\lambda^2(q - 1)(q - 2) + \\
 & 7\lambda(q - 1)(q - 2)(q - 3) + (q - 1)(q - 2)(q - 3)(q - 4) + 2\lambda^2(q - 1) + 6\lambda(q - 1)(q - 2) + \\
 & 3(q - 1)(q - 2)(q - 3) + \lambda(q - 1) + 2(q - 1)(q - 2). \\
 2Z_C U_C^v &= 3\lambda^7 + 3\lambda^5(q - 1) + 10\lambda^4(q - 1) + 4\lambda^3(q - 1)(q - 2) + 5\lambda^3(q - 1) + 10\lambda^2(q - 1)(q - 2) + \\
 & 3\lambda(q - 1)(q - 2)(q - 3) + 2\lambda^2(q - 1) + 4\lambda(q - 1)(q - 2) + \lambda(q - 1). \\
 6Z_C U_C^N &= 9\lambda^7 + 7\lambda^5(q - 1) + 30\lambda^4(q - 1) + 8\lambda^3(q - 1)(q - 2) + 19\lambda^3(q - 1) + 38\lambda^2(q - 1)(q - 2) + \\
 & 9\lambda(q - 1)(q - 2)(q - 3) + 6\lambda^2(q - 1) + 8\lambda(q - 1)(q - 2) + \lambda(q - 1).
 \end{aligned}$$

$$\begin{aligned} \tilde{S}_C &= 2(4r^8t^{13} + 52r^8t^{12} + 43r^7t^{13} + 312r^8t^{11} + 601r^7t^{12} + 202r^6t^{13} + 1144r^8t^{10} + 3869r^7t^{11} + 3028r^6t^{12} + \\ & 540r^5t^{13} + 2860r^8t^9 + 15191r^7t^{10} + 20867r^6t^{11} + 8680r^5t^{12} + 897r^4t^{13} + 5148r^8t^8 + 40590r^7t^9 + \\ & 87561r^6t^{10} + 63967r^5t^{11} + 15488r^4t^{12} + 951r^3t^{13} + 6864r^8t^7 + 77946r^7t^8 + 249672r^6t^9 + 286459r^5t^{10} + \\ & 122037r^4t^{11} + 17660r^3t^{12} + 636r^2t^{13} + 6864r^8t^6 + 110682r^7t^7 + 510972r^6t^8 + 870418r^5t^9 + 582615r^4t^{10} + \\ & 148697r^3t^{11} + 12644r^2t^{12} + 251rt^{13} + 5148r^8t^5 + 117678r^7t^6 + 772338r^6t^7 + 1896176r^5t^8 + 1883784r^4t^9 + \\ & 755755r^3t^{10} + 113399r^2t^{11} + 5249rt^{12} + 46t^{13} + 2860r^8t^4 + 93687r^7t^5 + 873102r^6t^6 + 3048260r^5t^7 + \\ & 4362023r^4t^8 + 2595899r^3t^9 + 612010r^2t^{10} + 49715rt^{11} + 978t^{12} + 1144r^8t^3 + 55165r^7t^4 + 738294r^6t^5 + \\ & 3662690r^5t^6 + 7449312r^4t^7 + 6378524r^3t^8 + 2228185r^2t^9 + 283566rt^{10} + 9634t^{11} + 312r^8t^2 + 23353r^7t^3 + \\ & 461272r^6t^4 + 3290362r^5t^5 + 9506758r^4t^6 + 11554675r^3t^7 + 5798142r^2t^8 + 1090936rt^9 + 57660t^{10} + 52r^8t + \\ & 6731r^7t^2 + 206995r^6t^3 + 2183128r^5t^4 + 9071459r^4t^5 + 15644259r^3t^6 + 11121681r^2t^7 + 2999361rt^8 + \\ & 233508t^9 + 4r^8 + 1184r^7t + 63185r^6t^2 + 1040021r^5t^3 + 6394875r^4t^4 + 15846771r^3t^5 + 15952293r^2t^6 + \\ & 6080067rt^7 + 676602t^8 + 96r^7 + 11760r^6t + 336915r^5t^2 + 3238095r^4t^3 + 11869965r^3t^4 + 17136468r^2t^5 + \\ & 9223605rt^6 + 1446633t^7 + 1008r^6 + 66528r^5t + 1115505r^4t^2 + 6394347r^3t^3 + 13634190r^2t^4 + \\ & 10494252rt^5 + 2317167t^6 + 6048r^5 + 234360r^4t + 2346921r^3t^2 + 7817769r^2t^3 + 8861886rt^4 + 2788263t^5 + \\ & 22680r^4 + 526176r^3t + 3062043r^2t^2 + 5408775rt^3 + 2496339t^4 + 54432r^3 + 734832r^2t + 2263545rt^2 + \\ & 1621053t^3 + 81648r^2 + 583200rt + 725355t^2 + 69984r + 201204t + 26244)(r + 2)(t + 1)^5. \end{aligned}$$

$$\tilde{S}_C|_{q=2} = 2(t^4 + 5t^3 + 12t^2 + 12t + 8)(t + 2)^7(t + 1)^5.$$

$$\begin{aligned} D_C^U &= (2s^3t^6 + 12s^3t^5 + 9s^2t^6 + 30s^3t^4 + 57s^2t^5 + 13st^6 + 40s^3t^3 + 153s^2t^4 + 87st^5 + 6t^6 + 30s^3t^2 + 225s^2t^3 + \\ & 249st^4 + 42t^5 + 12s^3t + 192s^2t^2 + 397st^3 + 126t^4 + 2s^3 + 90s^2t + 384st^2 + 214t^3 + 18s^2 + 216st + 234t^2 + \\ & 54s + 162t + 54)(st + s + 2t + 3)(s + 3)(s + 2)(t + 1)^4. \end{aligned}$$

$$D_C^U|_{q=2} = 4(t + 2)^4(t + 1)^4.$$

Local view 34 of 35.

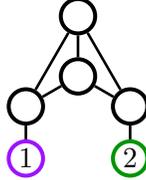

$$\begin{aligned} Z_C &= 2\lambda^6 + \lambda^5(q - 2) + 2\lambda^5 + 4\lambda^4(q - 2) + 2\lambda^3(q - 2)(q - 3) + 2\lambda^4 + 17\lambda^3(q - 2) + 15\lambda^2(q - 2)(q - 3) + \\ & 7\lambda(q - 2)(q - 3)(q - 4) + (q - 2)(q - 3)(q - 4)(q - 5) + 6\lambda^3 + 20\lambda^2(q - 2) + 27\lambda(q - 2)(q - 3) + \\ & 7(q - 2)(q - 3)(q - 4) + 4\lambda^2 + 21\lambda(q - 2) + 11(q - 2)(q - 3) + 2q - 4. \end{aligned}$$

$$\begin{aligned} 2Z_C U_C^v &= 6\lambda^6 + 3\lambda^5(q - 2) + 4\lambda^5 + 8\lambda^4(q - 2) + 4\lambda^3(q - 2)(q - 3) + 2\lambda^4 + 19\lambda^3(q - 2) + 10\lambda^2(q - 2)(q - 3) + \\ & 3\lambda(q - 2)(q - 3)(q - 4) + 8\lambda^3 + 16\lambda^2(q - 2) + 13\lambda(q - 2)(q - 3) + 4\lambda^2 + 11\lambda(q - 2). \end{aligned}$$

$$\begin{aligned} 6Z_C U_C^N &= 16\lambda^6 + 7\lambda^5(q - 2) + 12\lambda^5 + 20\lambda^4(q - 2) + 8\lambda^3(q - 2)(q - 3) + 10\lambda^4 + 65\lambda^3(q - 2) + 38\lambda^2(q - 2)(q - 3) + \\ & 9\lambda(q - 2)(q - 3)(q - 4) + 24\lambda^3 + 52\lambda^2(q - 2) + 35\lambda(q - 2)(q - 3) + 10\lambda^2 + 27\lambda(q - 2). \end{aligned}$$

$$\begin{aligned}
 \tilde{S}_C &= 2(4r^9t^{14} + 56r^9t^{13} + 53r^8t^{14} + 364r^9t^{12} + 782r^8t^{13} + 311r^7t^{14} + 1456r^9t^{11} + 5354r^8t^{12} + 4832r^7t^{13} + 1060r^6t^{14} + \\
 & 4004r^9t^{10} + 22544r^8t^{11} + 34816r^7t^{12} + 17332r^6t^{13} + 2316r^5t^{14} + 8008r^9t^9 + 65219r^8t^{10} + 154196r^7t^{11} + \\
 & 131337r^6t^{12} + 39801r^5t^{13} + 3375r^4t^{14} + 12012r^9t^8 + 137126r^8t^9 + 468955r^7t^{10} + 611406r^6t^{11} + 316853r^5t^{12} + \\
 & 60787r^4t^{13} + 3294r^3t^{14} + 13728r^9t^7 + 216084r^8t^8 + 1036032r^7t^9 + 1953617r^6t^{10} + 1549056r^5t^{11} + \\
 & 507416r^4t^{12} + 61882r^3t^{13} + 2084r^2t^{14} + 12012r^9t^6 + 259248r^8t^7 + 1714584r^7t^8 + 4532826r^6t^9 + \\
 & 5196588r^5t^{10} + 2601672r^4t^{11} + 539998r^3t^{12} + 40572r^2t^{13} + 777rt^{14} + 8008r^9t^5 + 237963r^8t^6 + 2159352r^7t^7 + \\
 & 7875952r^6t^8 + 12656061r^5t^9 + 9154266r^4t^{10} + 2898053r^3t^{11} + 368617r^2t^{12} + 15562rt^{13} + 130t^{14} + 4004r^9t^4 + \\
 & 166298r^8t^5 + 2079597r^7t^6 + 10411054r^6t^7 + 23079416r^5t^8 + 23386011r^4t^9 + 10681470r^3t^{10} + 2065453r^2t^{11} + \\
 & 146527rt^{12} + 2660t^{13} + 1456r^9t^3 + 87098r^8t^4 + 1524080r^7t^5 + 10521252r^6t^6 + 32016814r^5t^7 + 44738506r^4t^8 + \\
 & 28598227r^3t^9 + 7961479r^2t^{10} + 854726rt^{11} + 25834t^{12} + 364r^9t^2 + 33152r^8t^3 + 836696r^7t^4 + 8089266r^6t^5 + \\
 & 33954977r^5t^6 + 65118602r^4t^7 + 57362099r^3t^8 + 22316625r^2t^9 + 3439366rt^{10} + 156416t^{11} + 56r^9t + 8669r^8t^2 + \\
 & 333652r^7t^3 + 4657791r^6t^4 + 27397004r^5t^5 + 72476656r^4t^6 + 87578534r^3t^7 + 46902435r^2t^8 + 10082132rt^9 + \\
 & 655872t^{10} + 4r^9 + 1394r^8t + 91361r^7t^2 + 1947660r^6t^3 + 16555585r^5t^4 + 61388212r^4t^5 + 102294306r^3t^6 + \\
 & 75087492r^2t^7 + 22187058rt^8 + 2008428t^9 + 104r^8 + 15376r^7t + 559087r^6t^2 + 7265440r^5t^3 + 38953572r^4t^4 + \\
 & 90978576r^3t^5 + 92034801r^2t^6 + 37230984rt^7 + 4624848t^8 + 1200r^7 + 98616r^6t + 2188881r^5t^2 + 17956608r^4t^3 + \\
 & 60654834r^3t^4 + 85967946r^2t^5 + 47881692rt^6 + 8131536t^7 + 8064r^6 + 405216r^5t + 5684337r^4t^2 + 29395476r^3t^3 + \\
 & 60250743r^2t^4 + 46981404rt^5 + 10971288t^6 + 34776r^5 + 1106028r^4t + 9789147r^3t^2 + 30725676r^2t^3 + \\
 & 34631793rt^4 + 11309382t^5 + 99792r^4 + 2004912r^3t + 10777293r^2t^2 + 18600840rt^3 + 8772300t^4 + 190512r^3 + \\
 & 2326968r^2t + 6881031rt^2 + 4966920t^3 + 233280r^2 + 1568808rt + 1940598t^2 + 166212r + 468018t + 52488)(t+1)^4. \\
 \tilde{S}_C|_{q=2} &= 4(2t^4 + 7t^3 + 12t^2 + 12t + 4)(t+2)^7(t+1)^4. \\
 D_C^U &= (2s^3t^6 + 12s^3t^5 + 9s^2t^6 + 30s^3t^4 + 57s^2t^5 + 13st^6 + 40s^3t^3 + 153s^2t^4 + 87st^5 + 6t^6 + 30s^3t^2 + 225s^2t^3 + \\
 & 249st^4 + 42t^5 + 12s^3t + 192s^2t^2 + 397st^3 + 126t^4 + 2s^3 + 90s^2t + 384st^2 + 214t^3 + 18s^2 + 216st + 234t^2 + \\
 & 54s + 162t + 54)(st + s + 2t + 3)(st + s + t + 2)(s + 3)(t + 1)^3. \\
 D_C^U|_{q=2} &= 4(t+2)^4(t+1)^3.
 \end{aligned}$$

Local view 35 of 35 (named  $K_4$ ).

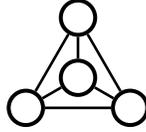

$$\begin{aligned}
 Z_C &= \lambda^6q + 4\lambda^3(q-1)q + 3\lambda^2(q-1)q + 6\lambda(q-1)(q-2)q + (q-1)(q-2)(q-3)q. \\
 2Z_C U_C^v &= 3\lambda^6q + 6\lambda^3(q-1)q + 3\lambda^2(q-1)q + 3\lambda(q-1)(q-2)q. \\
 6Z_C U_C^N &= 9\lambda^6q + 18\lambda^3(q-1)q + 9\lambda^2(q-1)q + 9\lambda(q-1)(q-2)q. \\
 \tilde{S}_C &= 6(2r^5t^8 + 16r^5t^7 + 14r^4t^8 + 56r^5t^6 + 125r^4t^7 + 40r^3t^8 + 112r^5t^5 + 485r^4t^6 + 392r^3t^7 + 59r^2t^8 + 140r^5t^4 + \\
 & 1070r^4t^5 + 1668r^3t^6 + 620r^2t^7 + 45rt^8 + 112r^5t^3 + 1470r^4t^4 + 4032r^3t^5 + 2857r^2t^6 + 496rt^7 + 14t^8 + \\
 & 56r^5t^2 + 1289r^4t^3 + 6068r^3t^4 + 7512r^2t^5 + 2445r^6 + 160t^7 + 16r^5t + 705r^4t^2 + 5832r^3t^3 + 12328r^2t^4 + \\
 & 6942rt^5 + 838t^6 + 2r^5 + 220r^4t + 3500r^3t^2 + 12962r^2t^3 + 12358rt^4 + 2556t^5 + 30r^4 + 1200r^3t + 8550r^2t^2 + \\
 & 14160rt^3 + 4908t^4 + 180r^3 + 3240r^2t + 10260rt^2 + 6093t^3 + 540r^2 + 4320rt + 4833t^2 + 810r + 2268t + \\
 & 486)(rt^2 + 2rt + t^2 + r + 3t + 3)^2(r+3)(r+2)(t+1)^6. \\
 \tilde{S}_C|_{q=2} &= 12(t^2 + t + 2)(t+2)^7(t+1)^6. \\
 D_C^U &= 0.
 \end{aligned}$$

## REFERENCES

- [1] E. Davies, M. Jenssen, W. Perkins, and B. Roberts. Extremes of the internal energy of the Potts models on cubic graphs. *arXiv preprint arXiv:1610.08496*, 2016.

LONDON SCHOOL OF ECONOMICS

*E-mail address:* {e.s.davies,m.o.jenssen,b.j.roberts}@lse.ac.uk

UNIVERSITY OF BIRMINGHAM

*E-mail address:* math@willperkins.org
